# Supplementary material for: Ghost-free High Dynamic Range Imaging via Hybrid CNN-Transformer and Structure Tensor
Source: arXiv:2212.00595 source file (2022-12-01)

# Supplementary Material

## Ghost-free High Dynamic Range Imaging via Hybrid CNN-Transformer and Structure Tensor

Yu Yuan[1], Jiaqi Wu[2], Zhongliang Jing[1], Henry Leung[3], Han Pan[1]

[1] Shanghai Jiao Tong University

[2] University of Electronic Science and Technology of China

[3] University of Calgary

# 1. Comparison against state-of-the-art approaches (2 input LDR images)

# Scene No.1

# Input LDR image 1

Exposure Value: -2.0

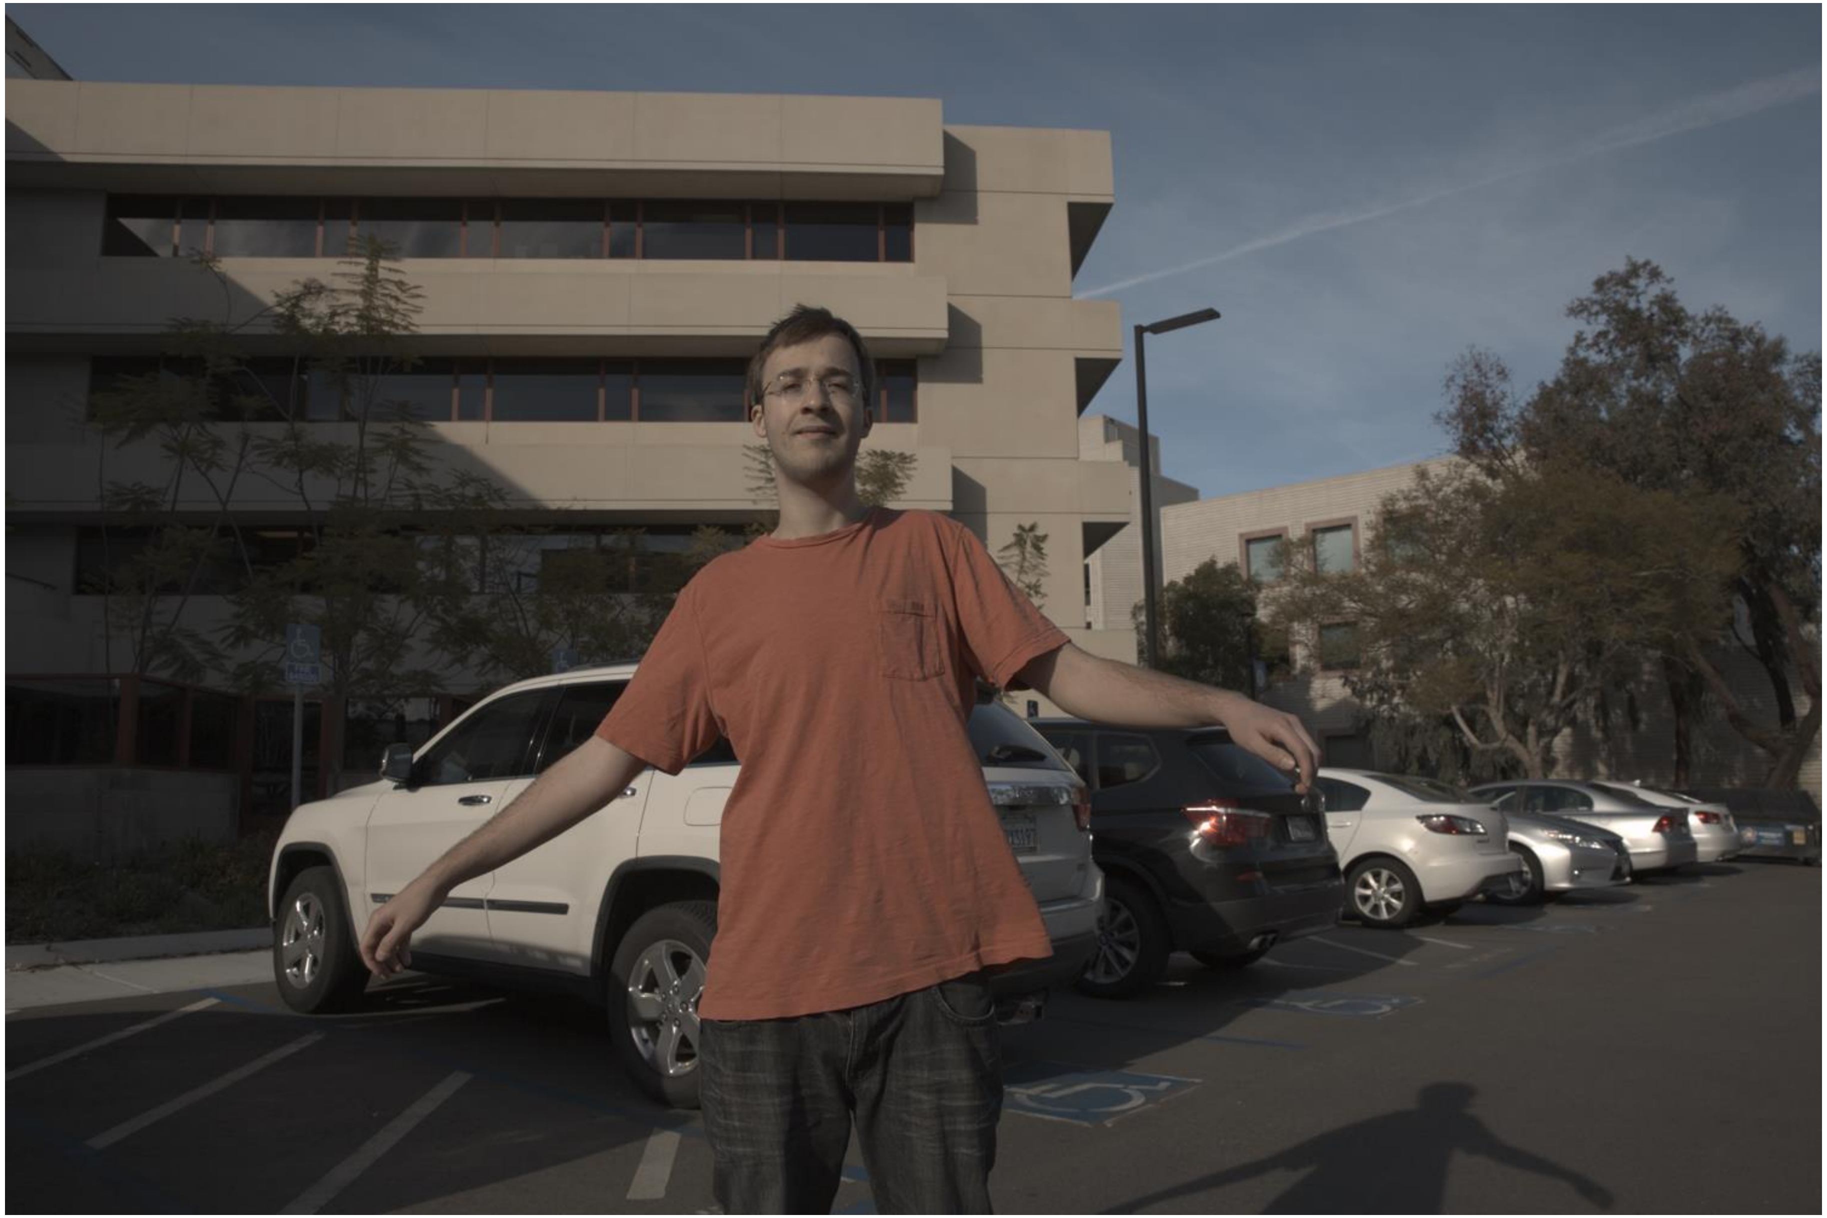

# Input LDR image 2
Exposure Value: 0.0

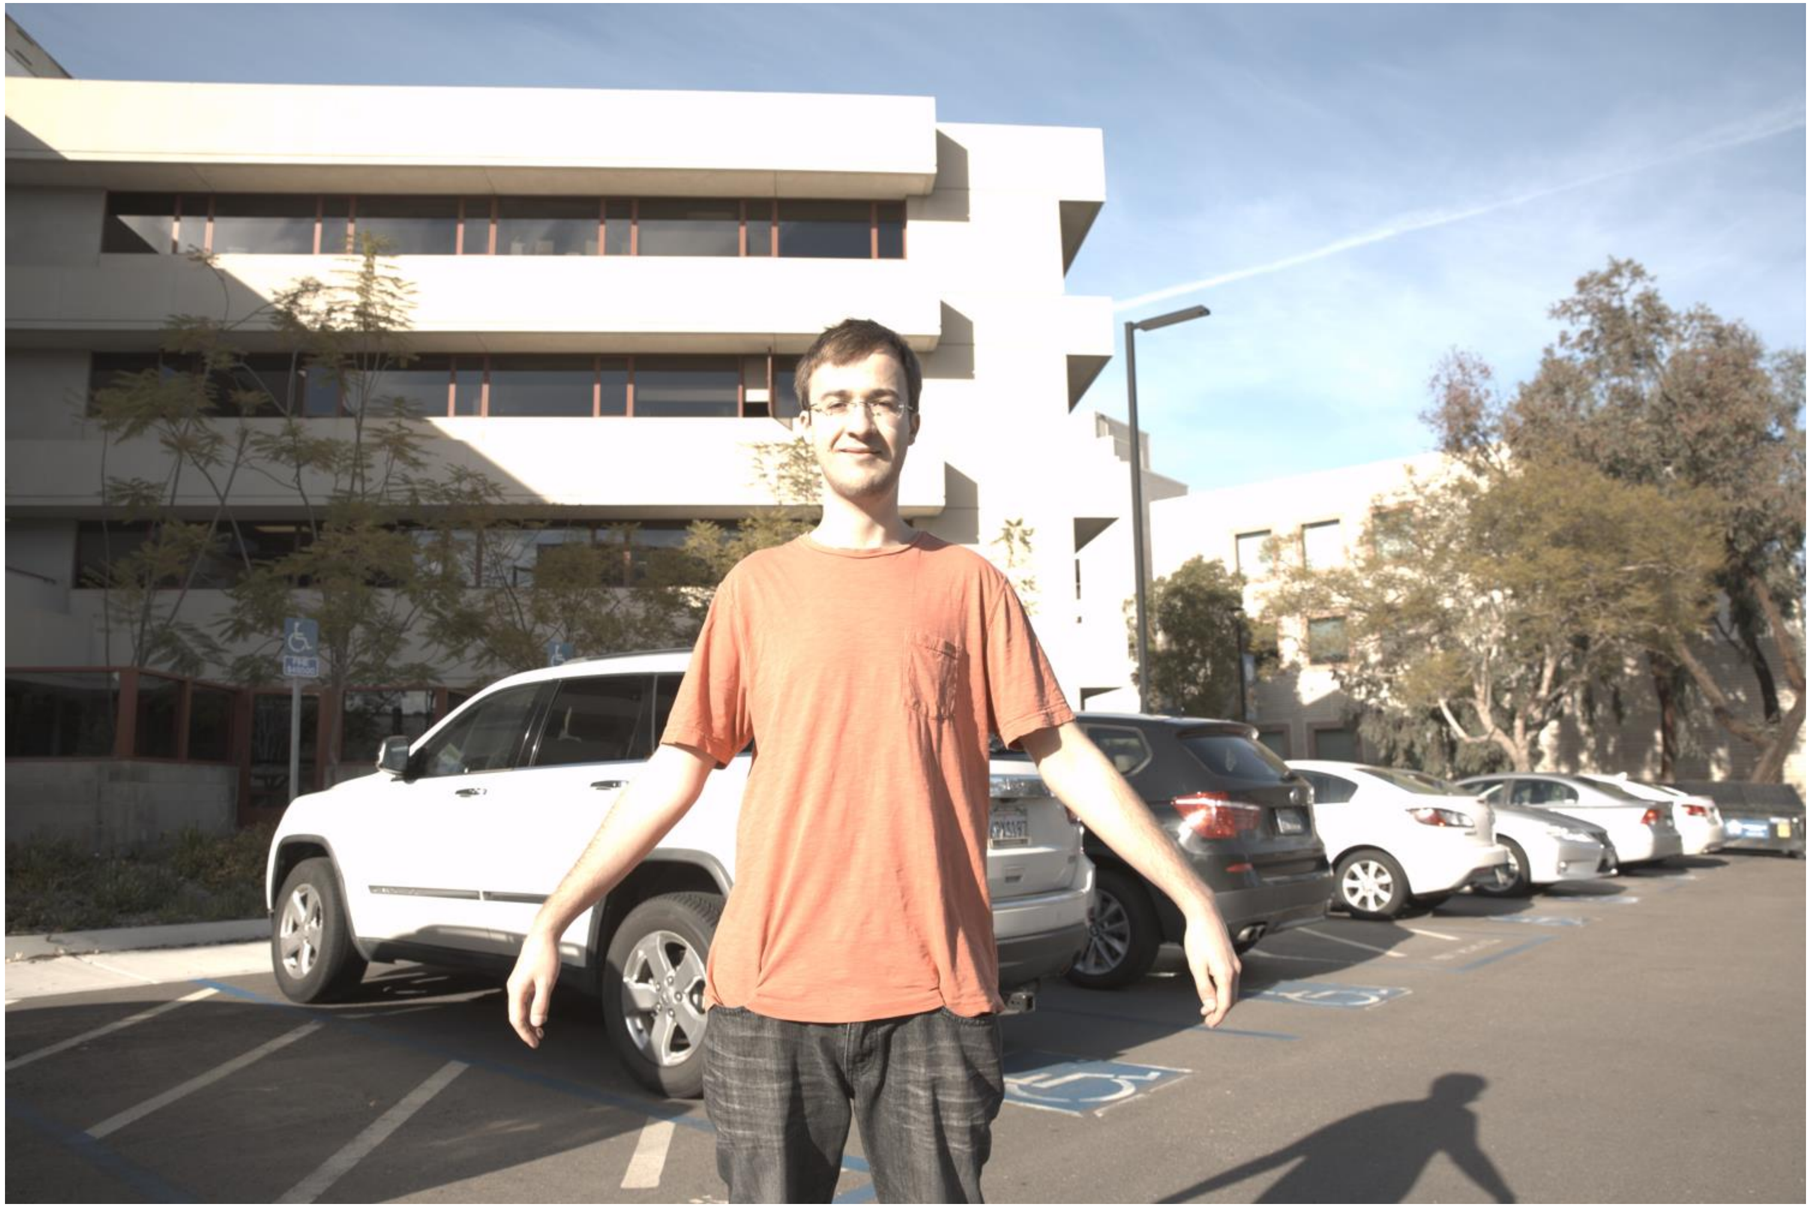

# HDR result
Sen et al. [2012]

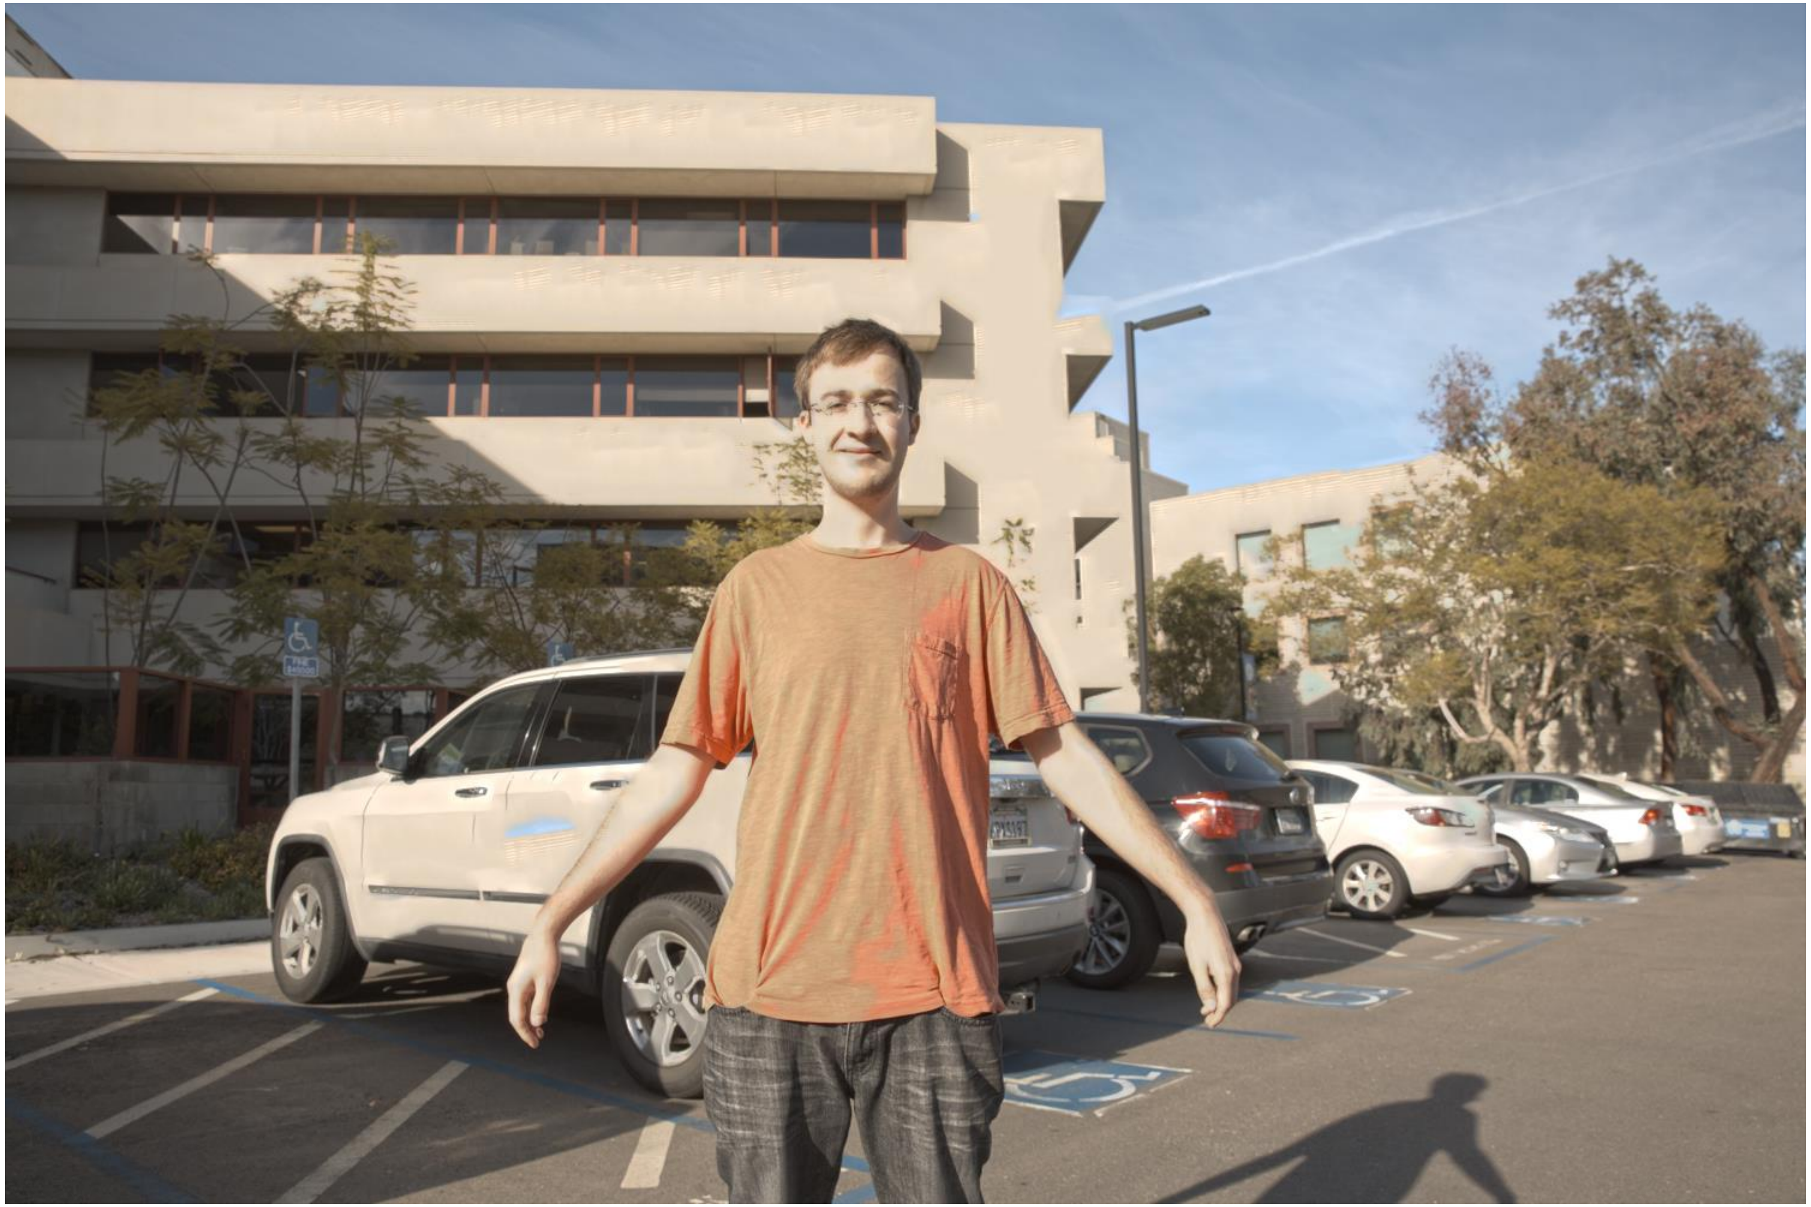

# HDR result
Kalantari et al. [2017]

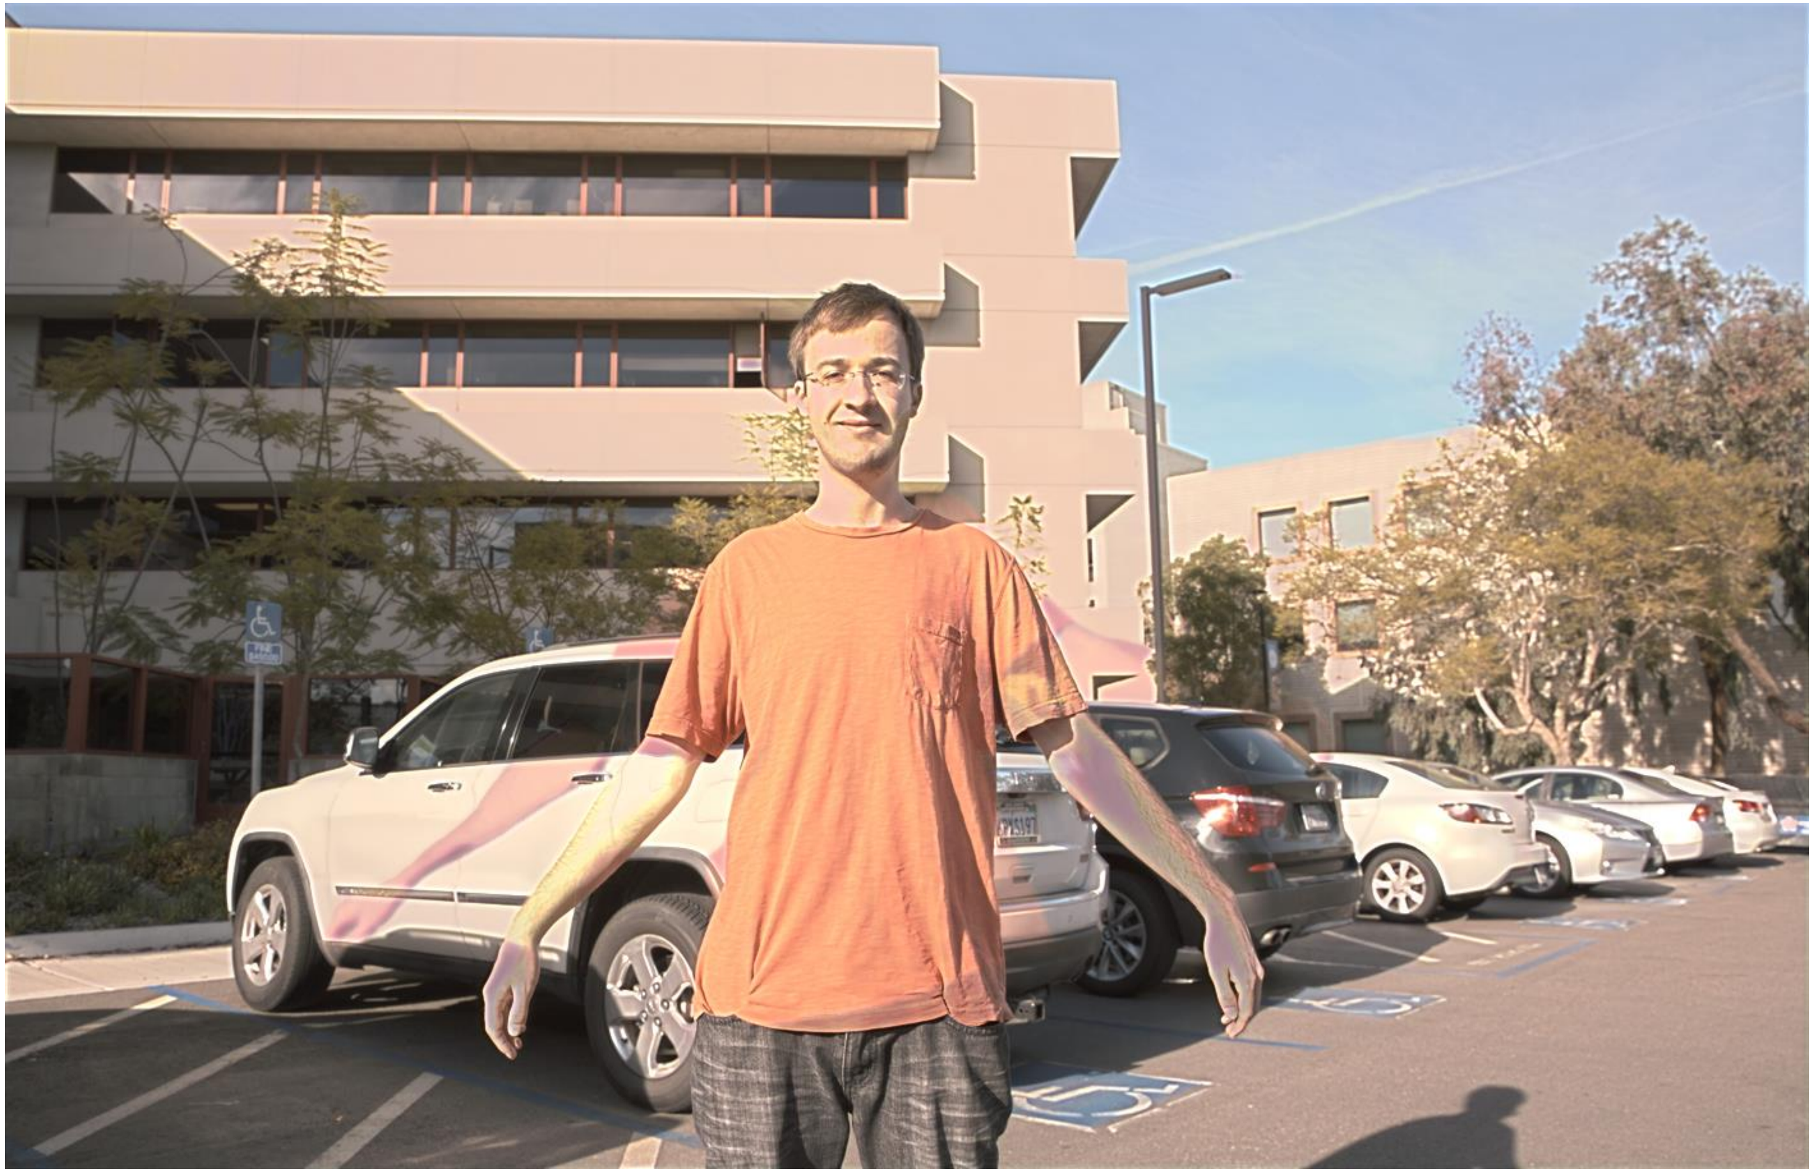

# HDR result
Wu et al. [2018]

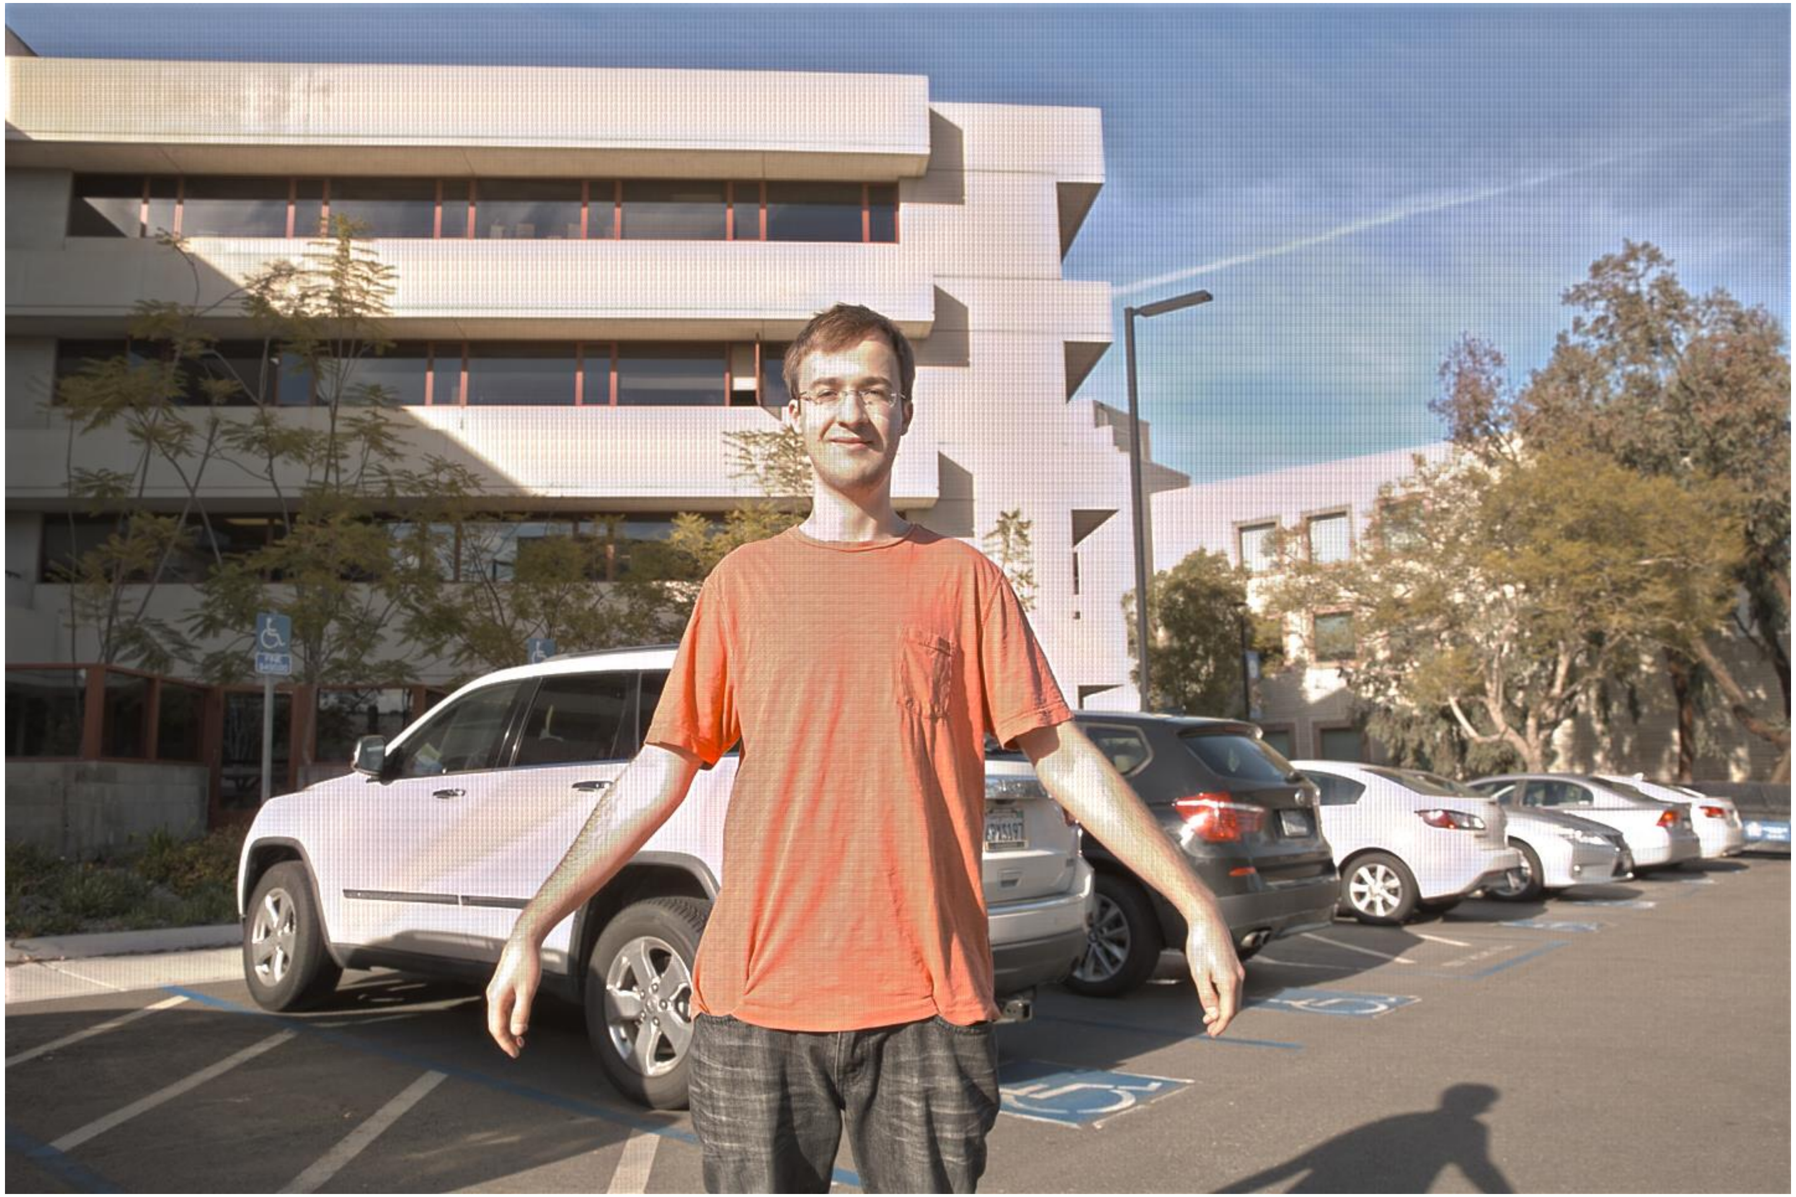

# HDR result
Yan et al. [2019]

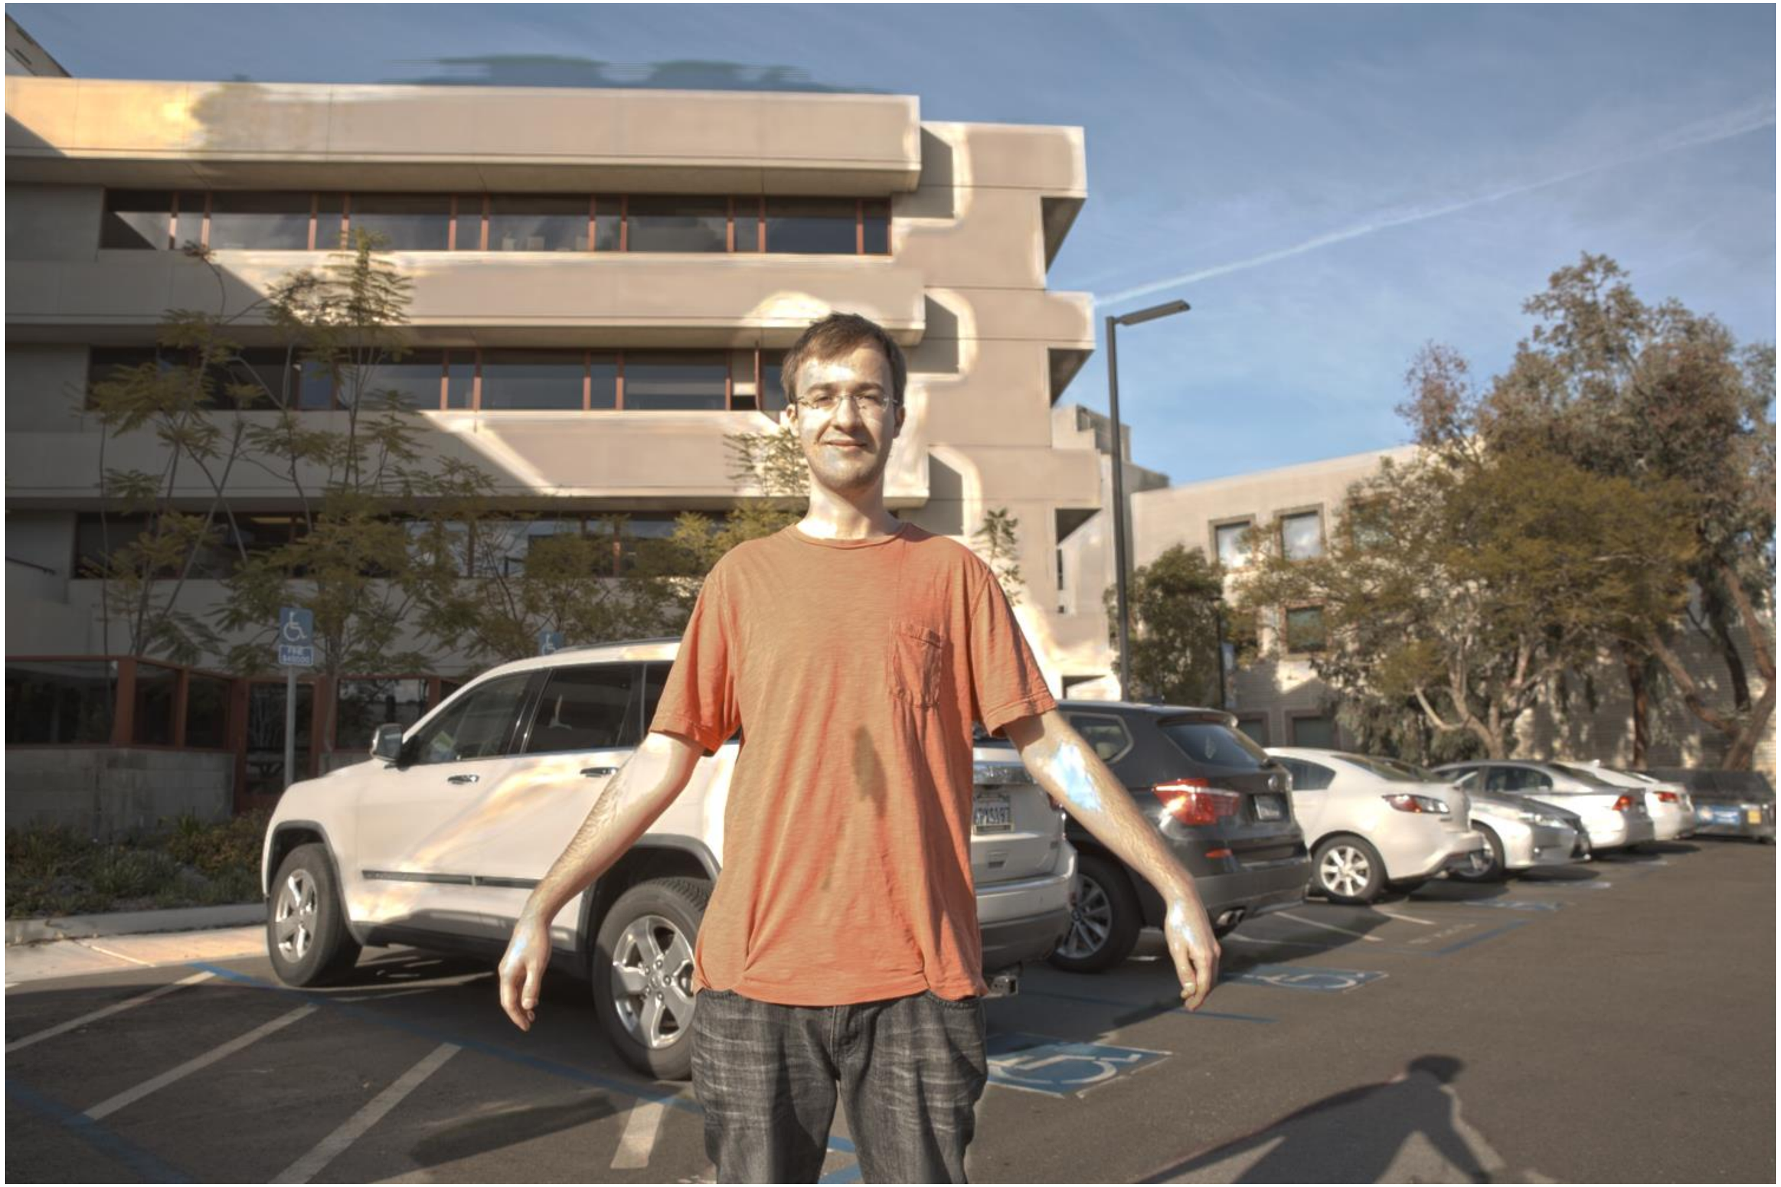

# HDR result
Li et al. [2020]

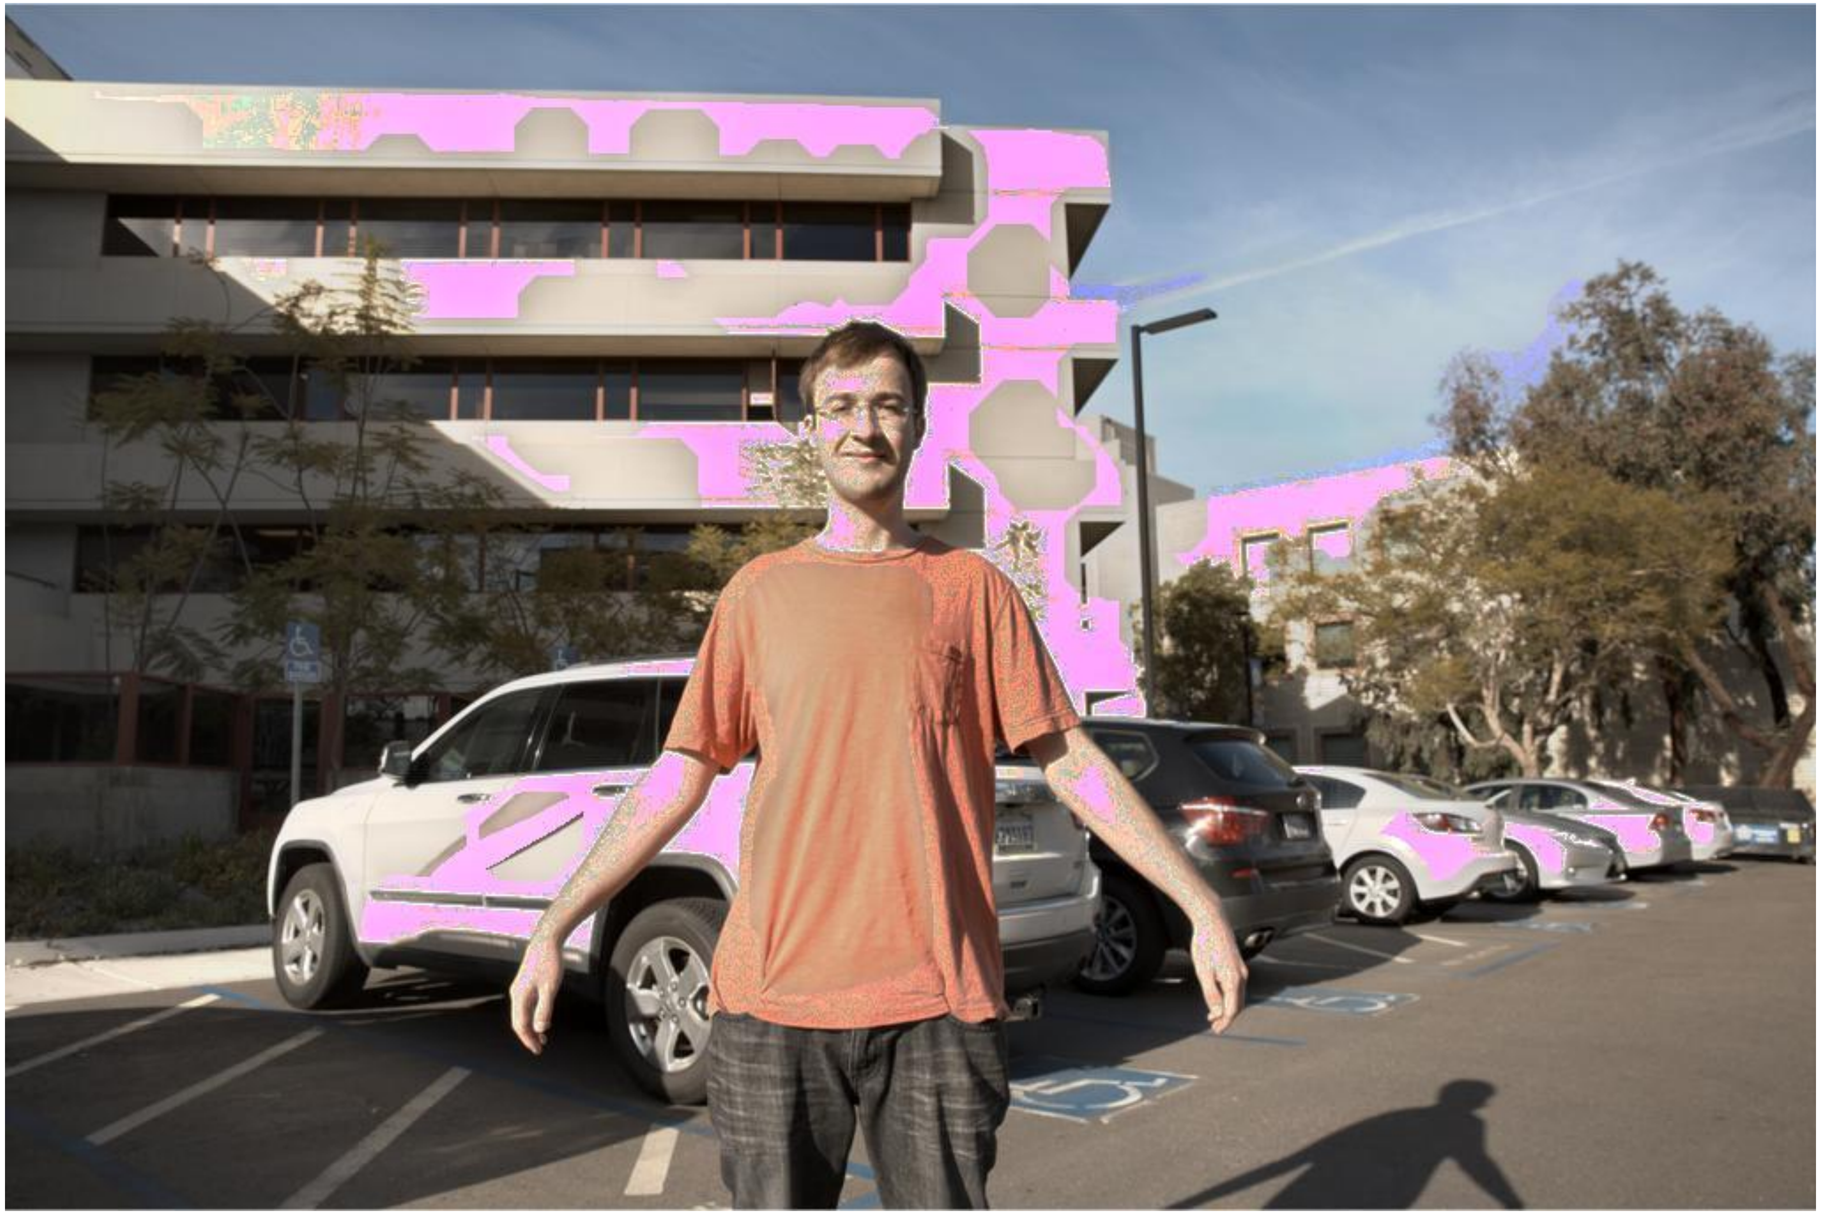

# HDR result
Niu et al. [2021]

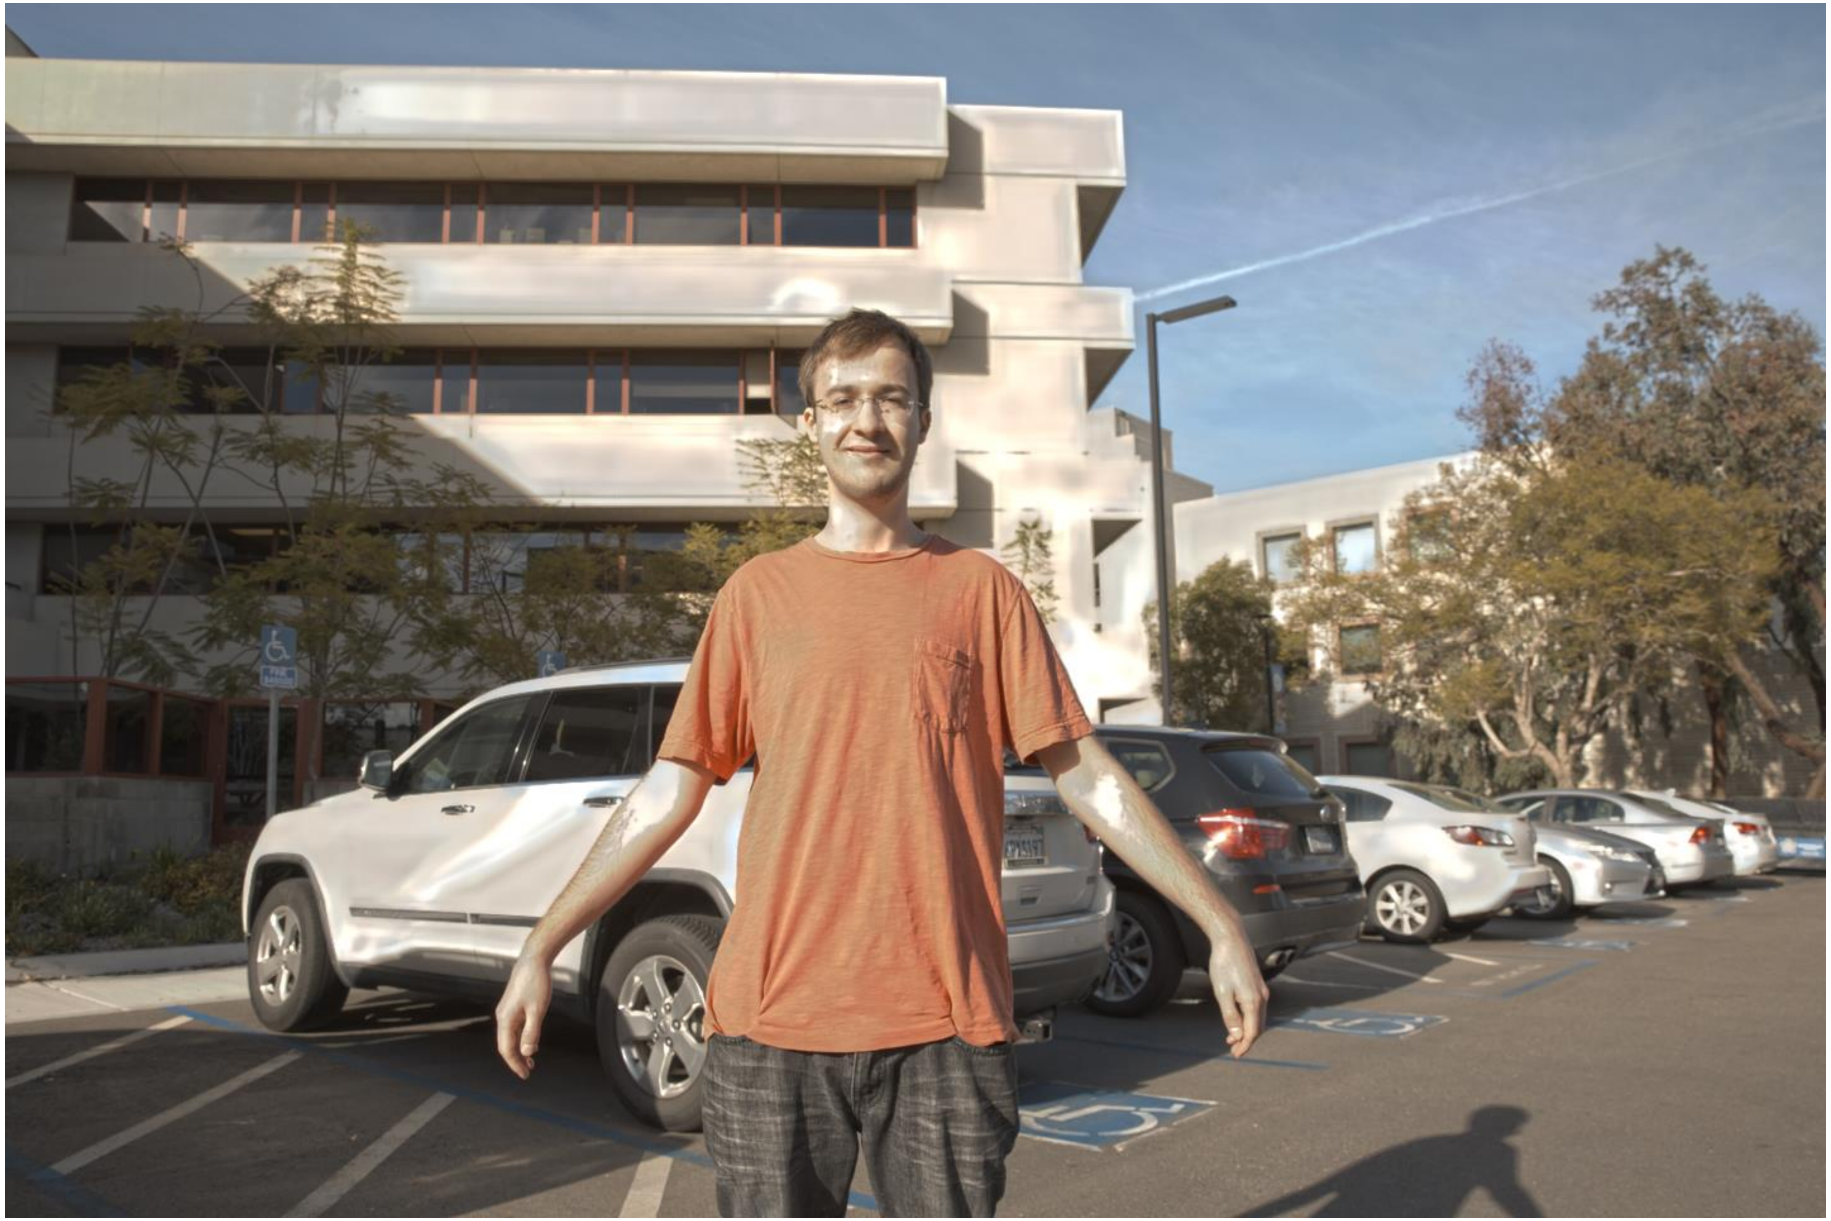

# HDR result
Ours

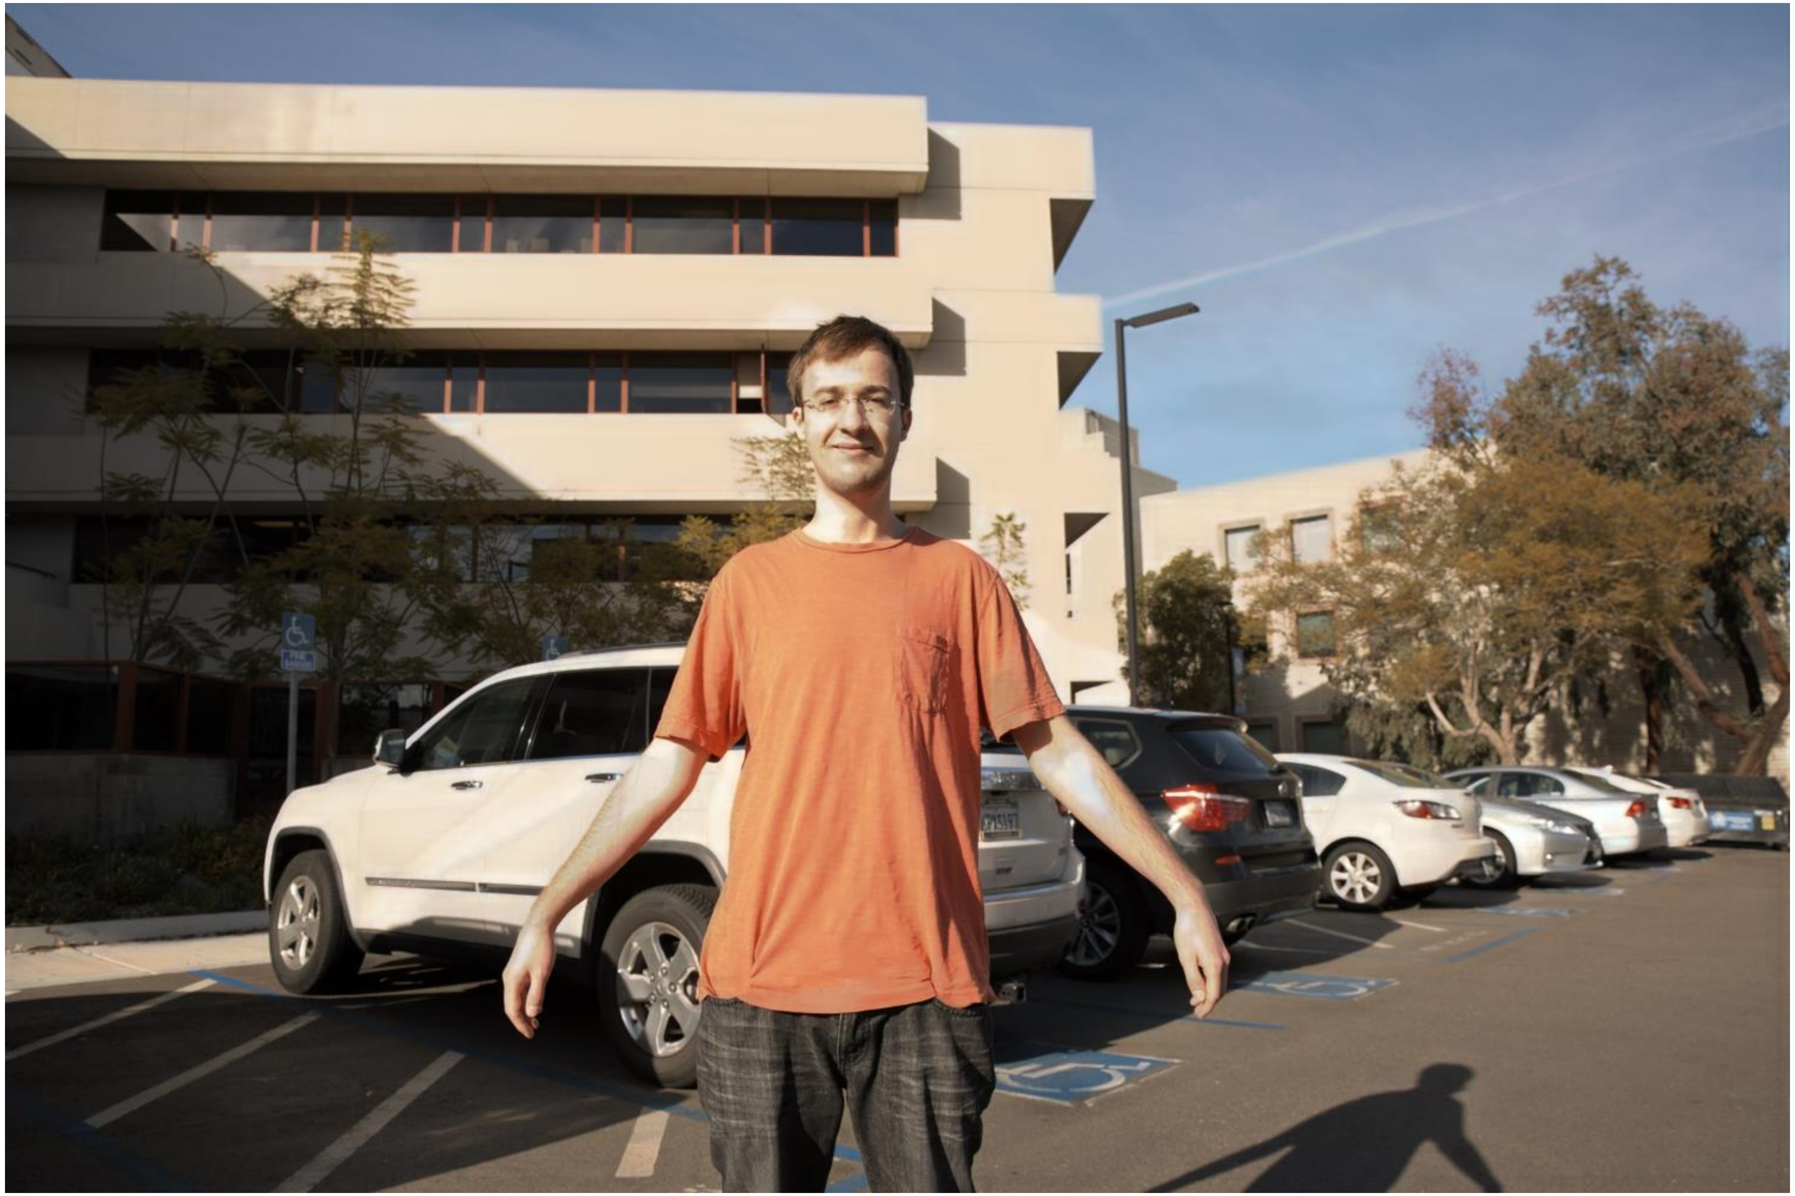

# HDR
Ground Truth

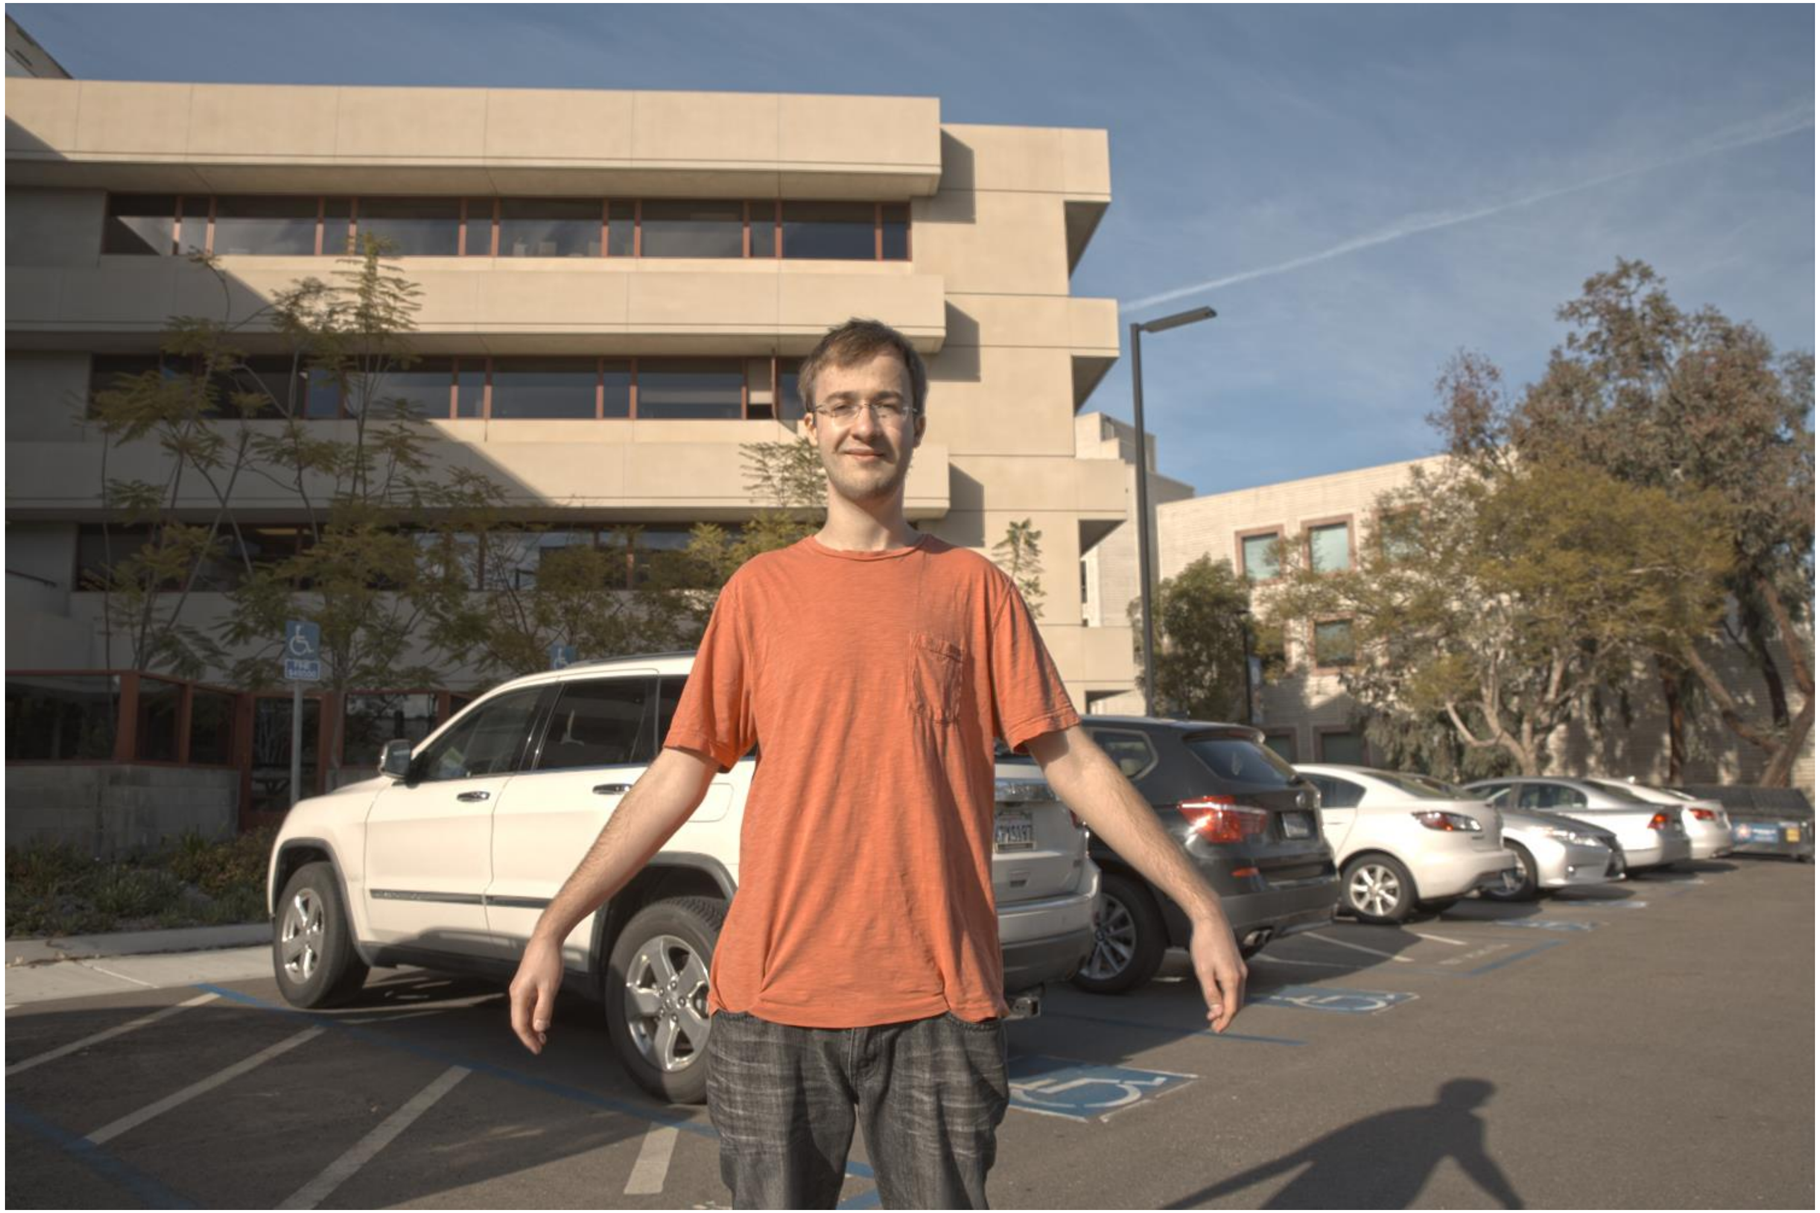

# Scene No.2

# Input LDR image 1
## Exposure Value: -2.0

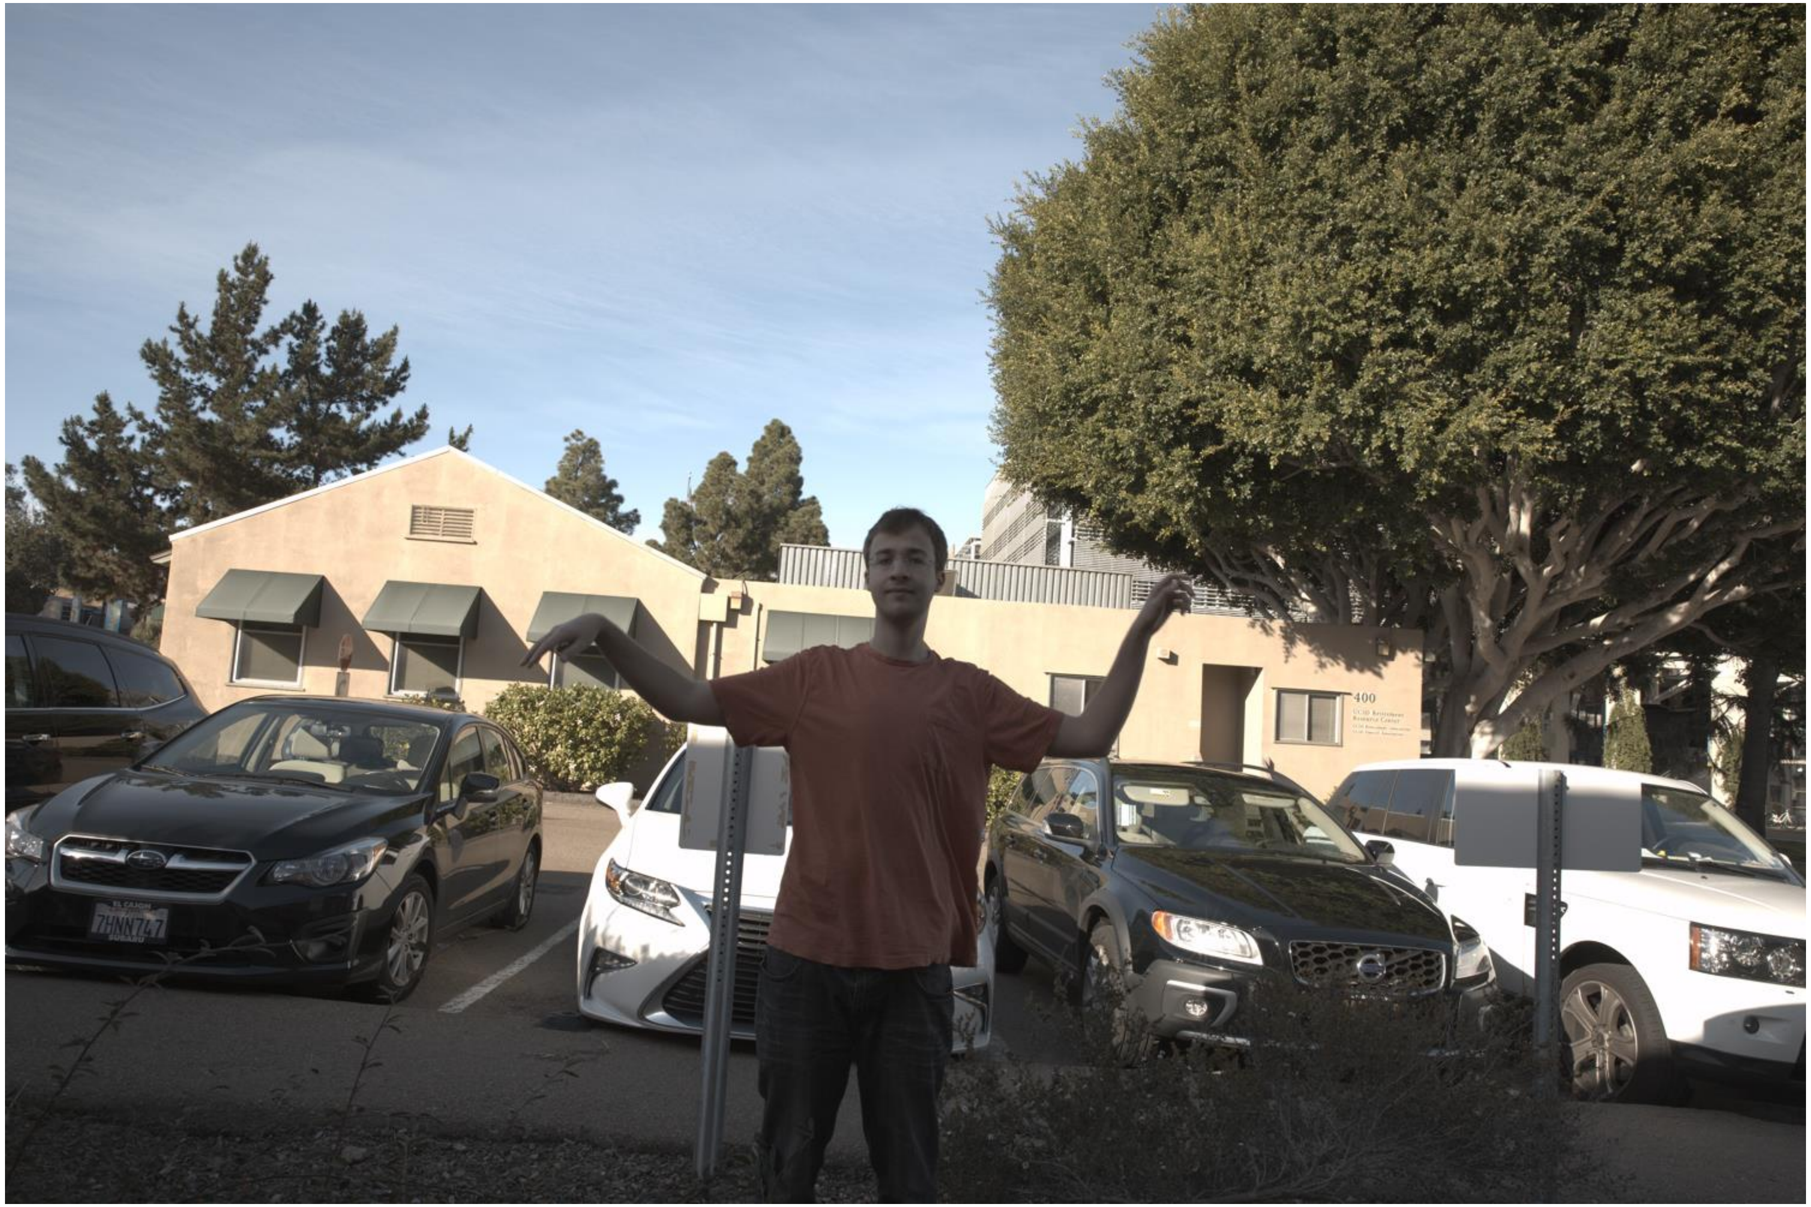

# Input LDR image 2

Exposure Value: 0.0

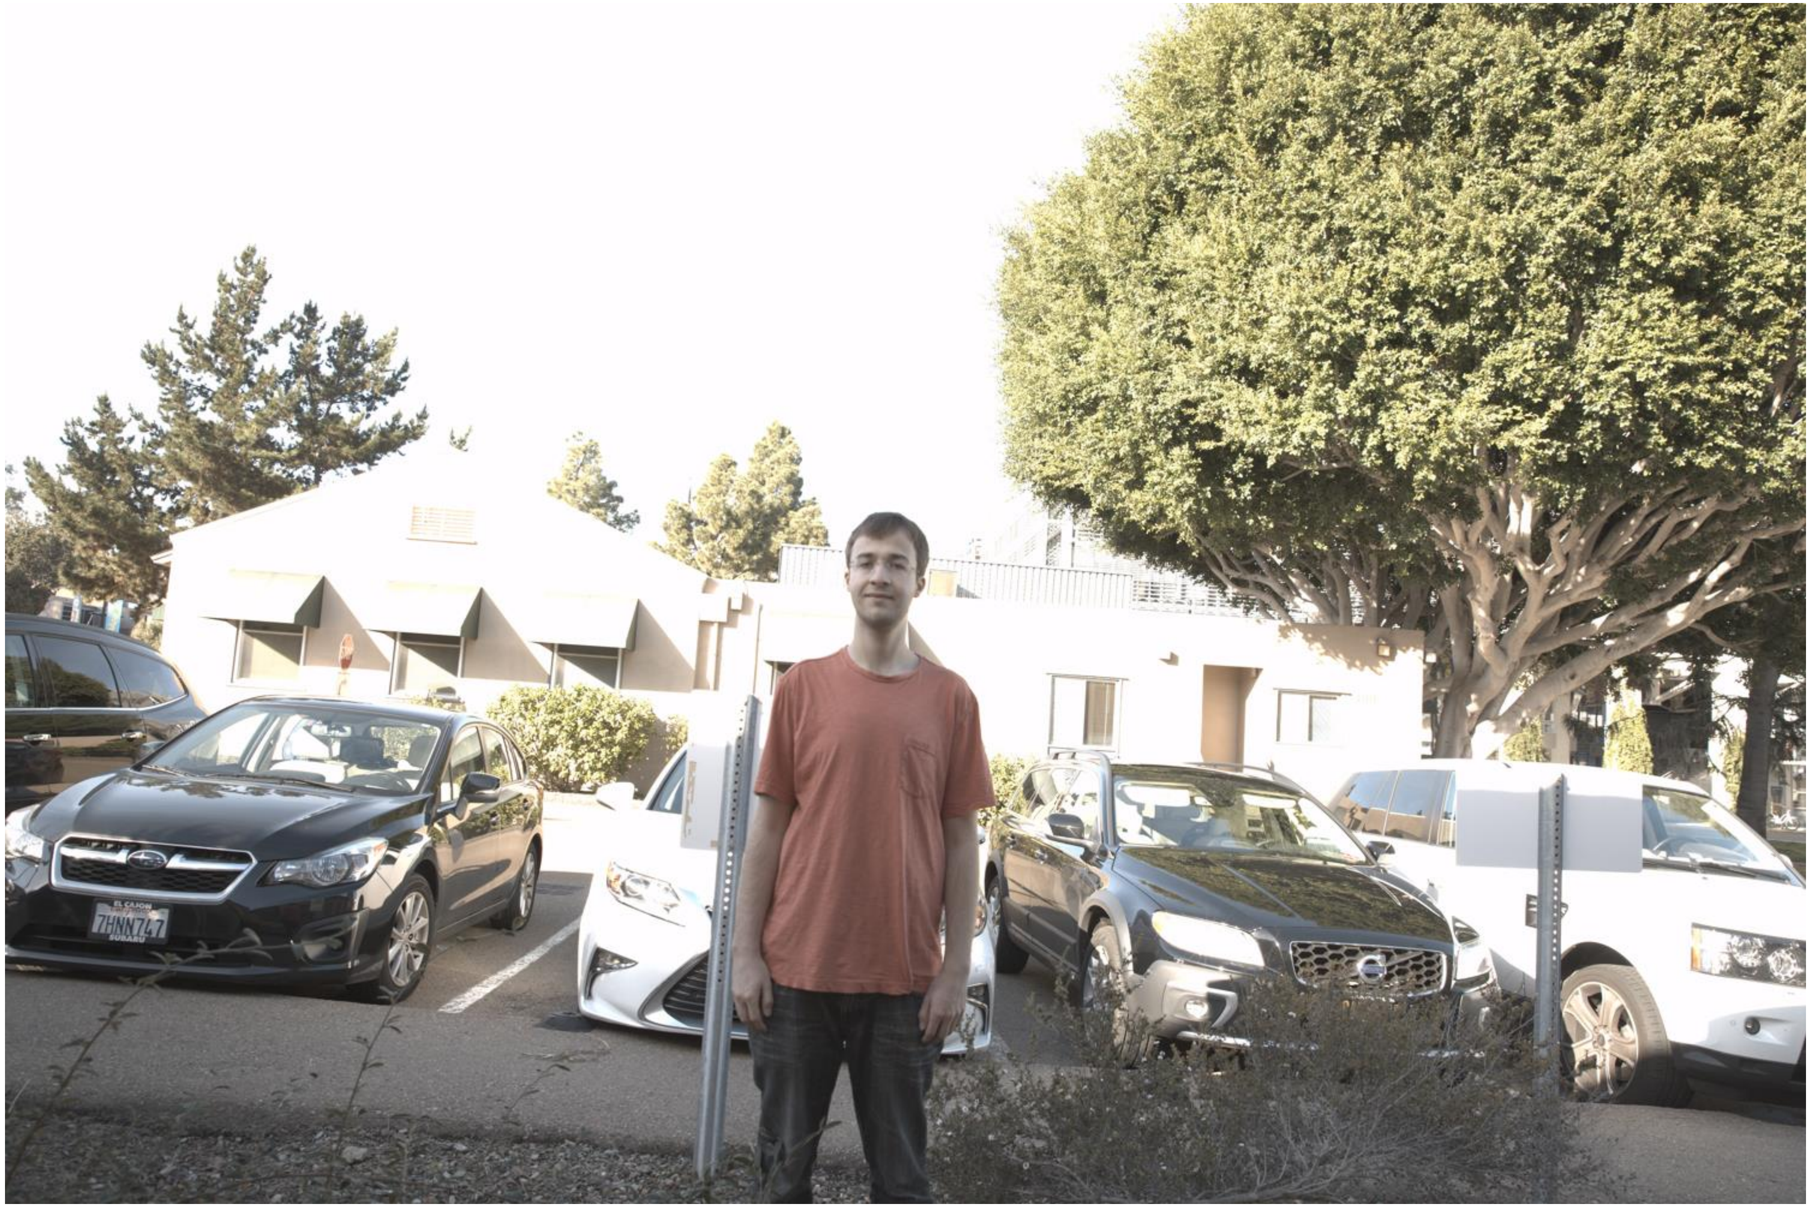

# HDR result
Sen et al. [2012]

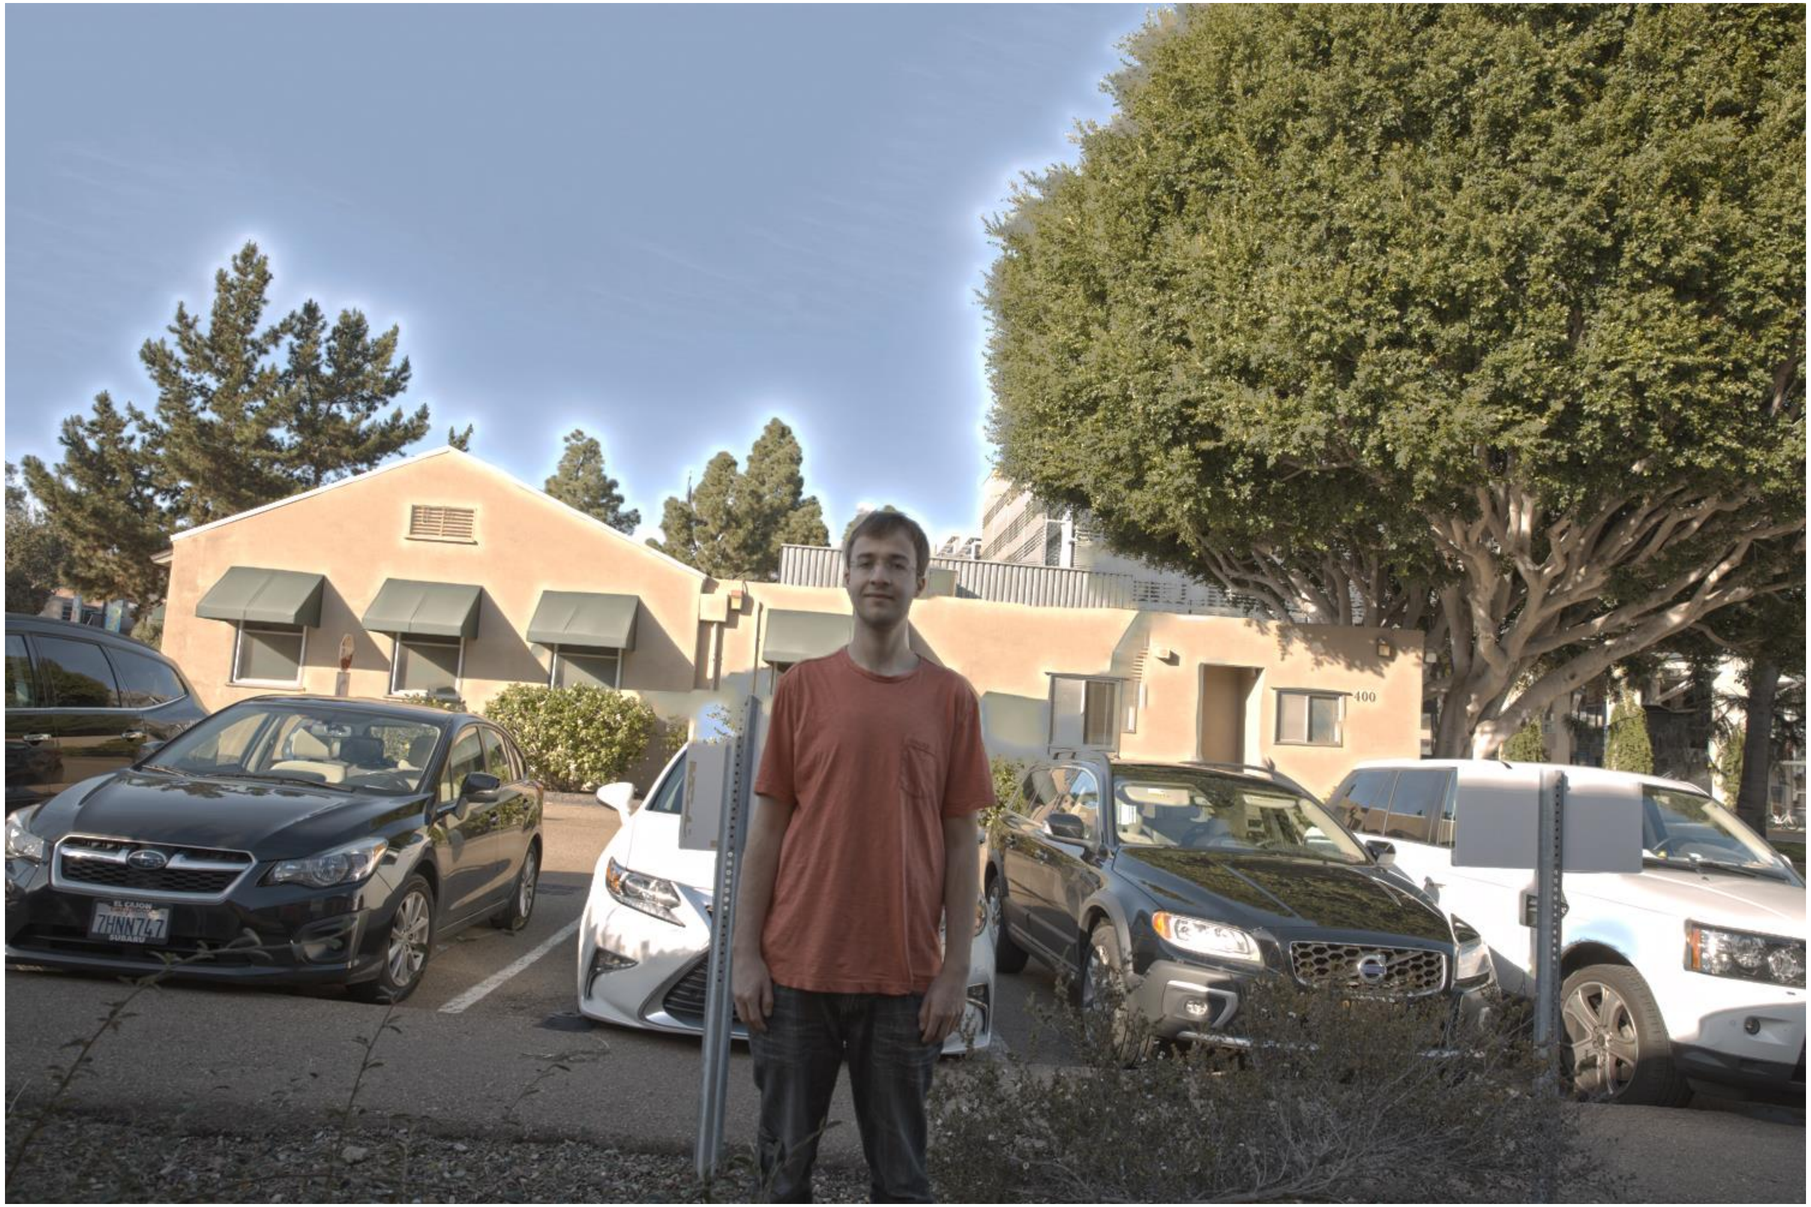

# HDR result
Kalantari et al. [2017]

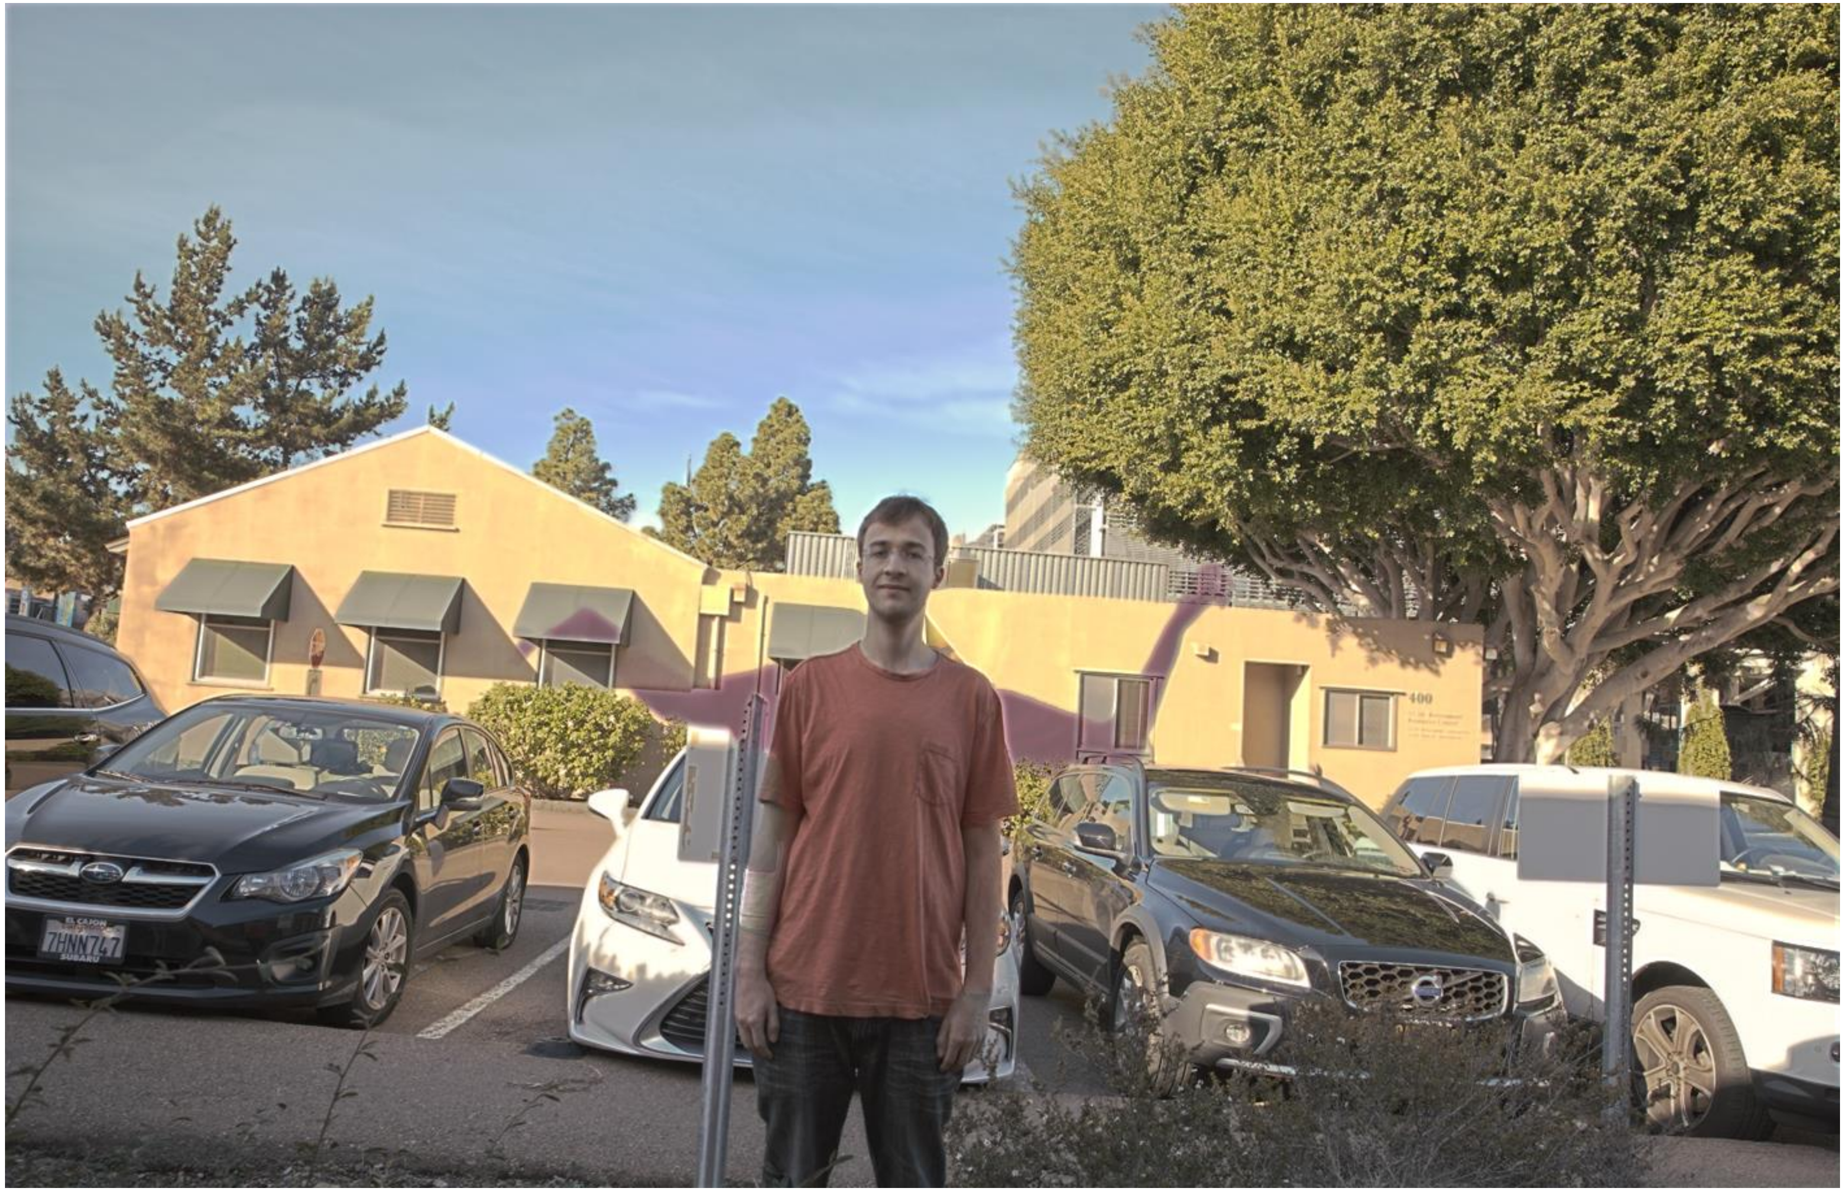

# HDR result
Wu et al. [2018]

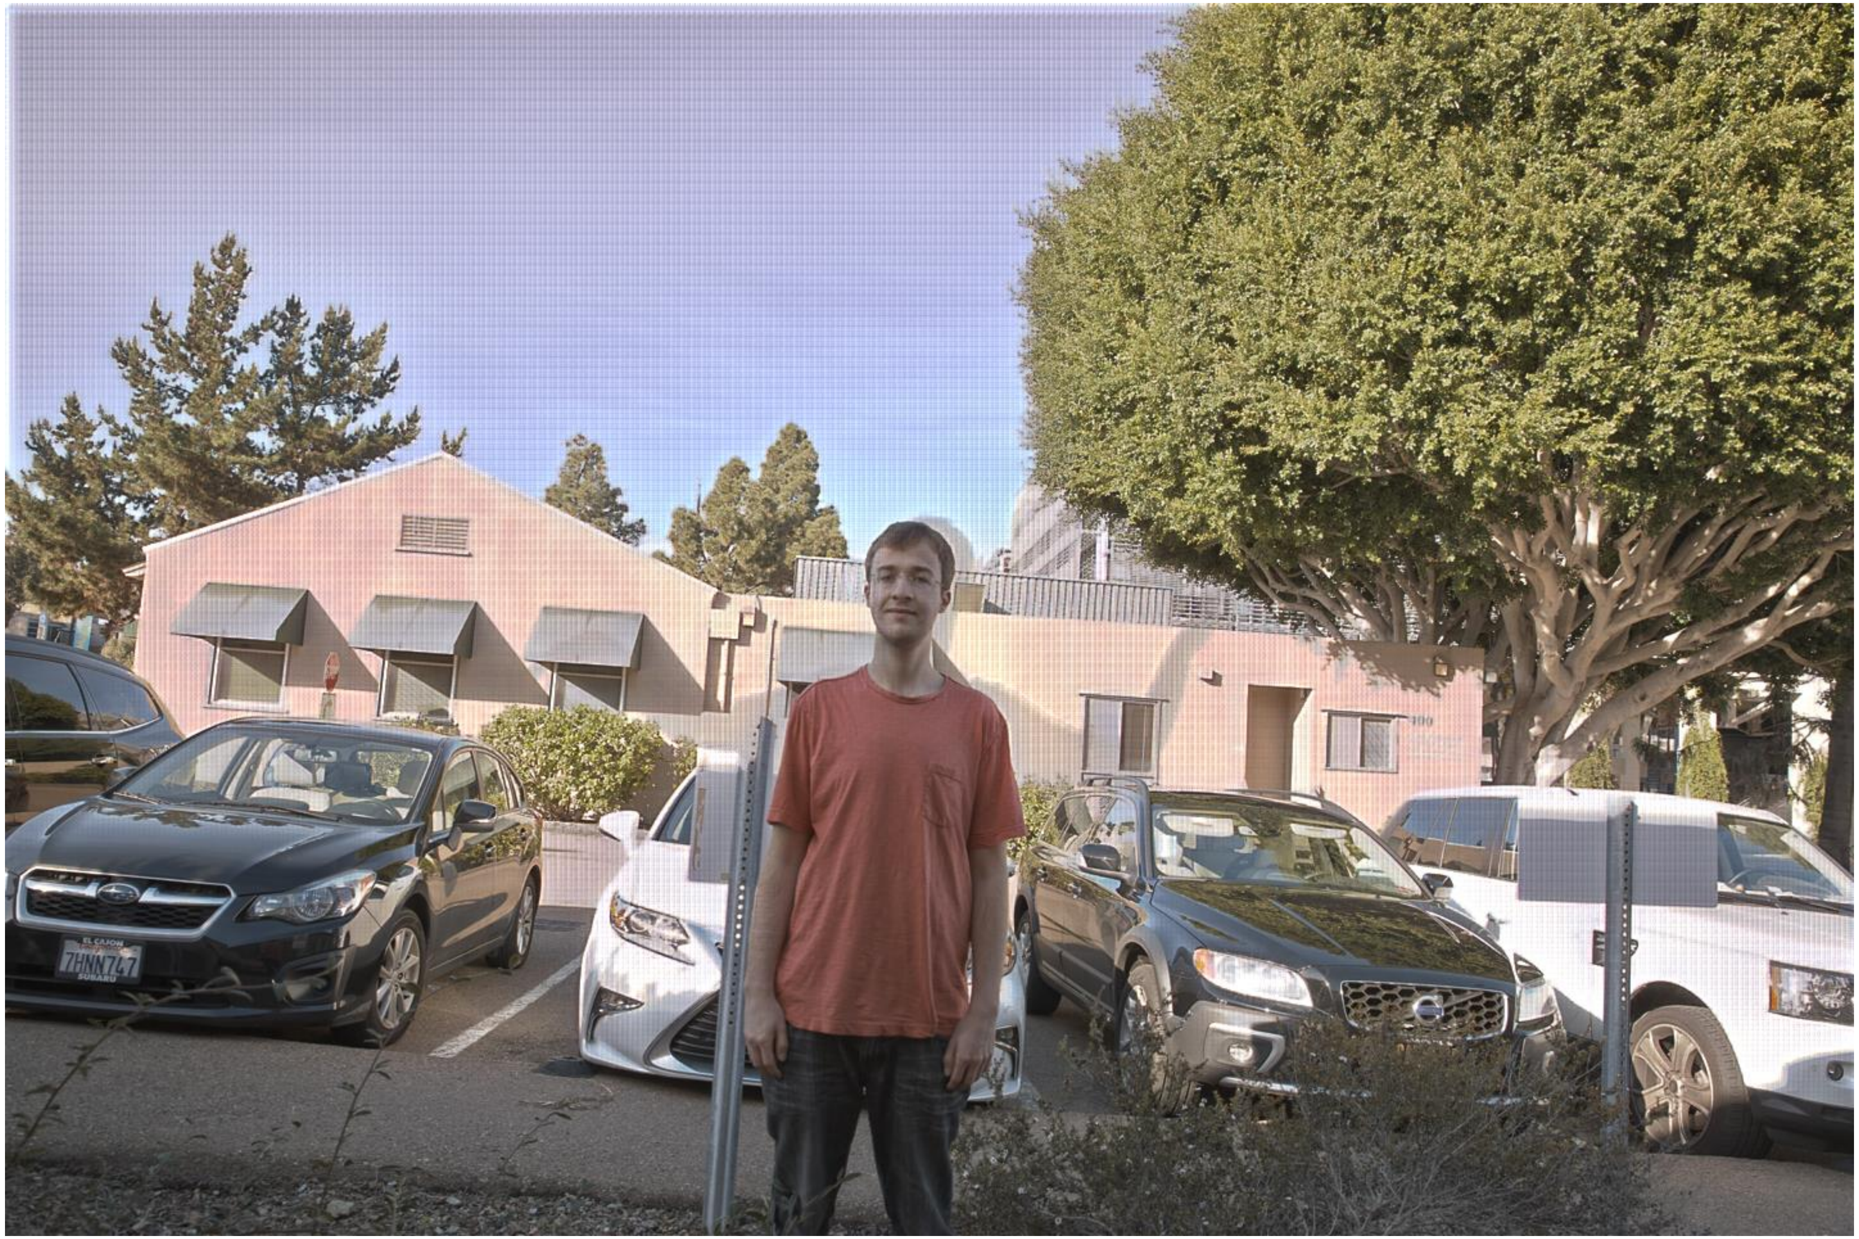

# HDR result

Yan et al. [2019]

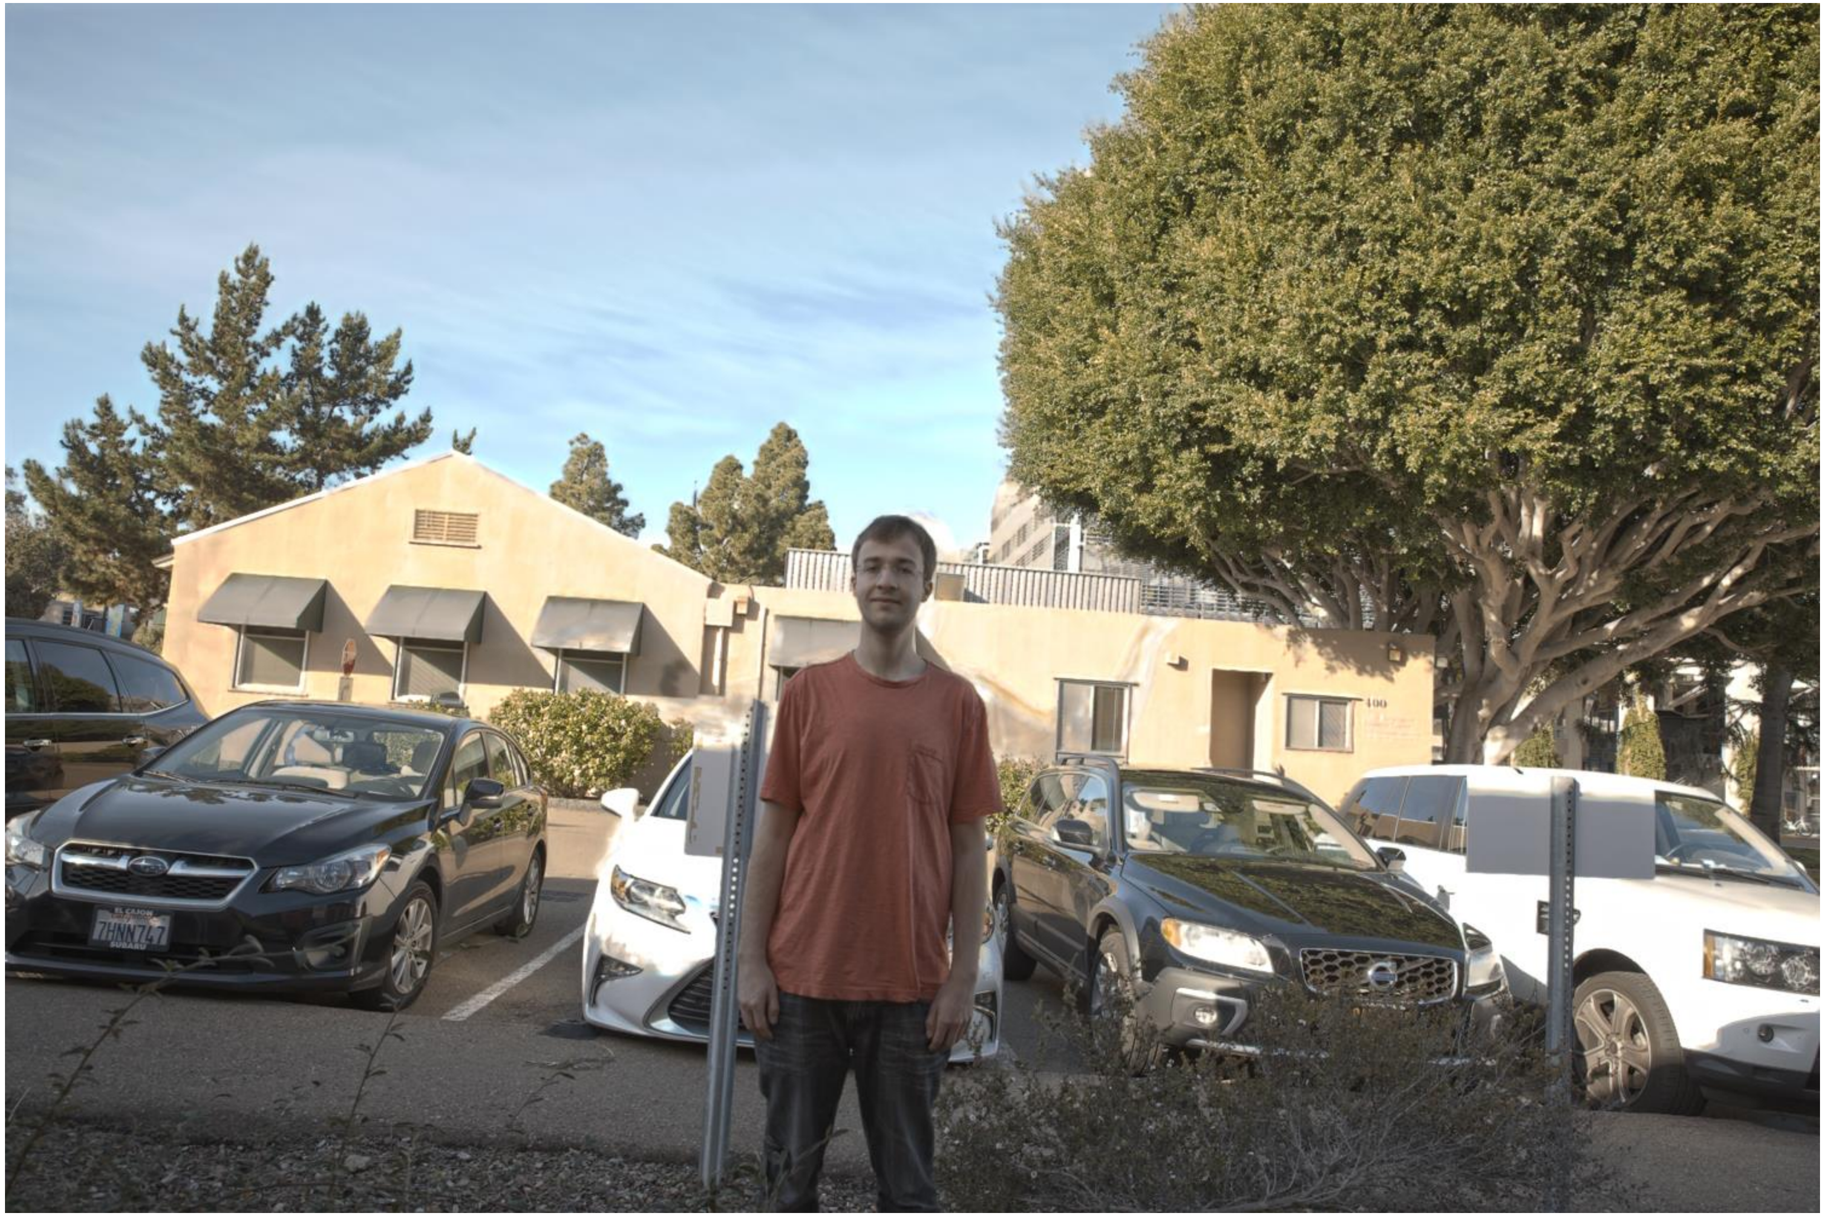

# HDR result
Li et al. [2020]

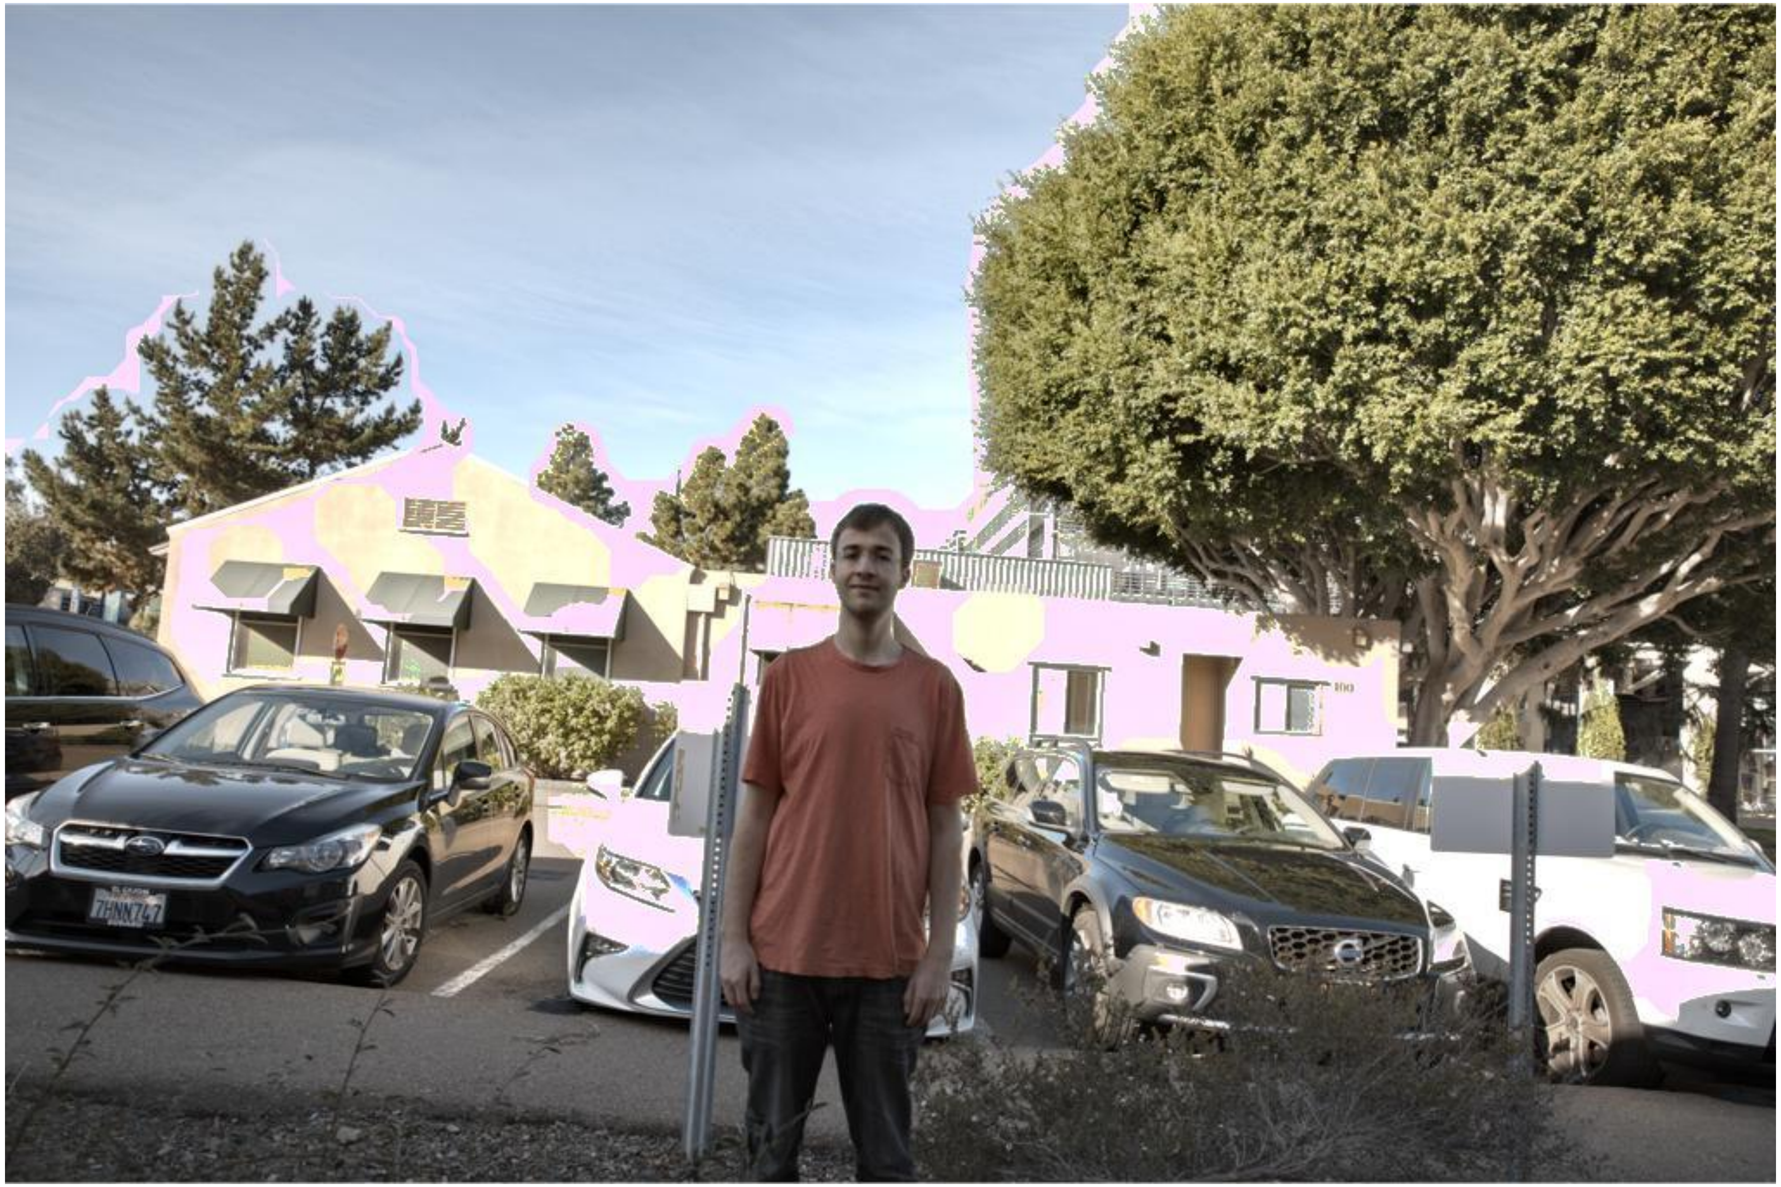

# HDR result
Niu et al. [2021]

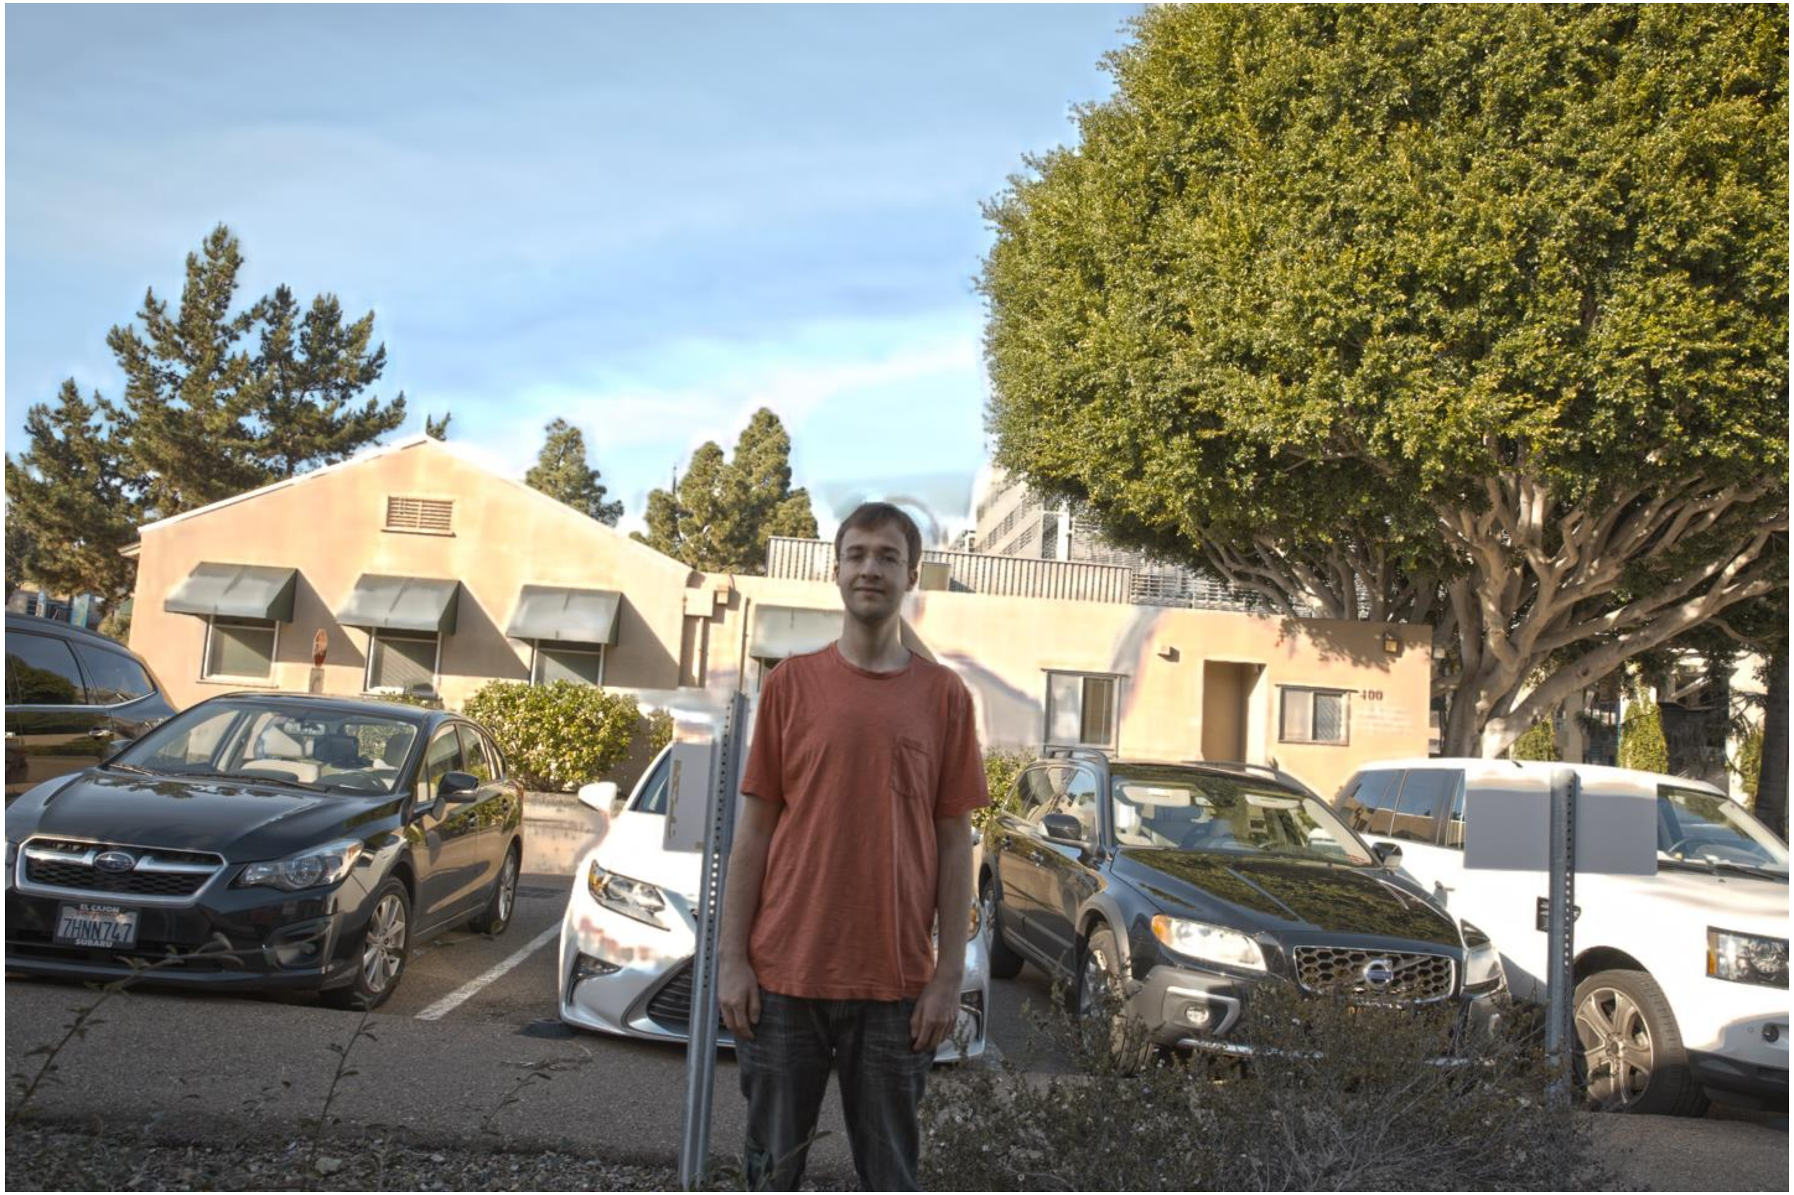

# HDR result
Ours

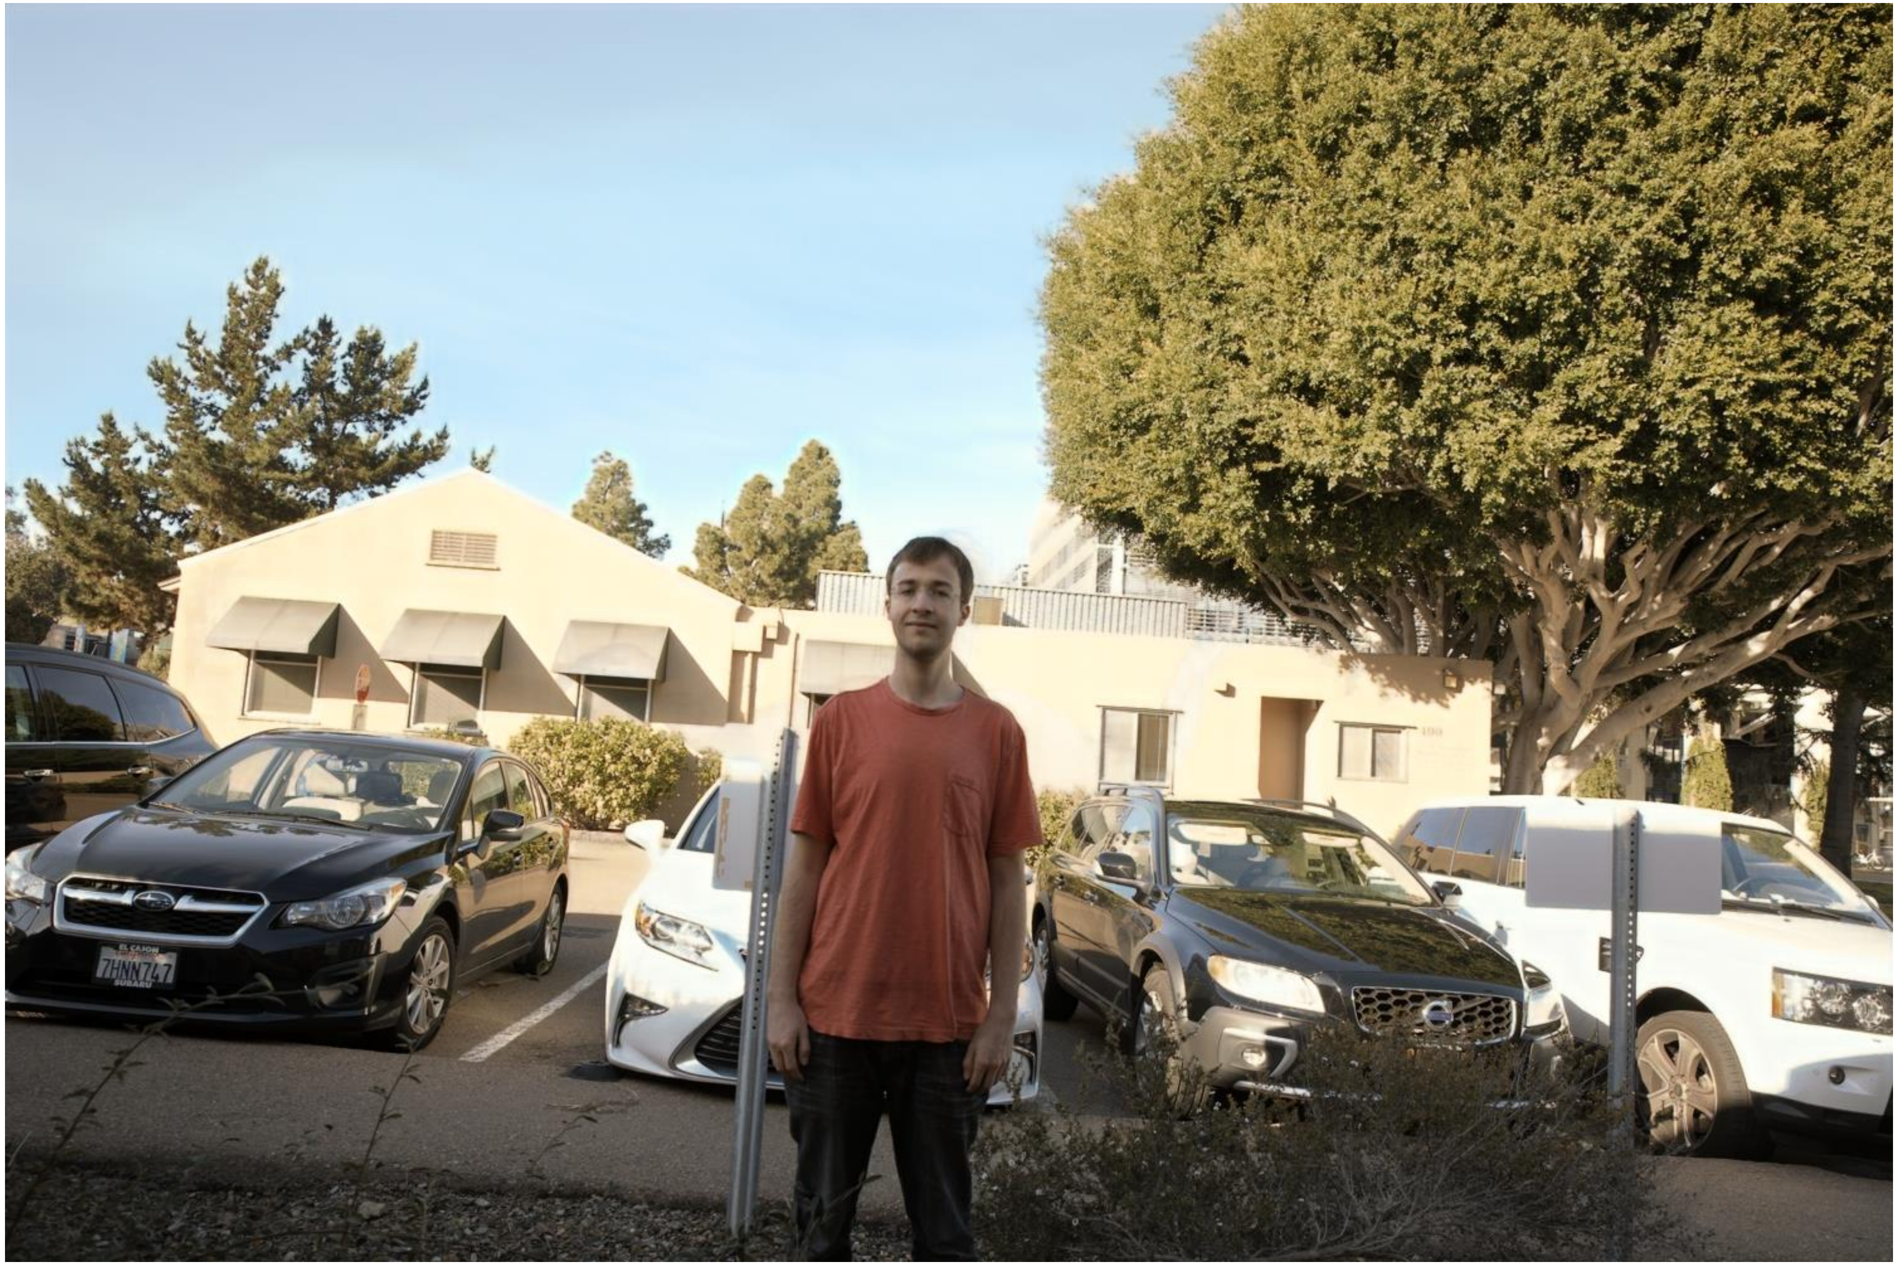

# HDR
## Ground Truth

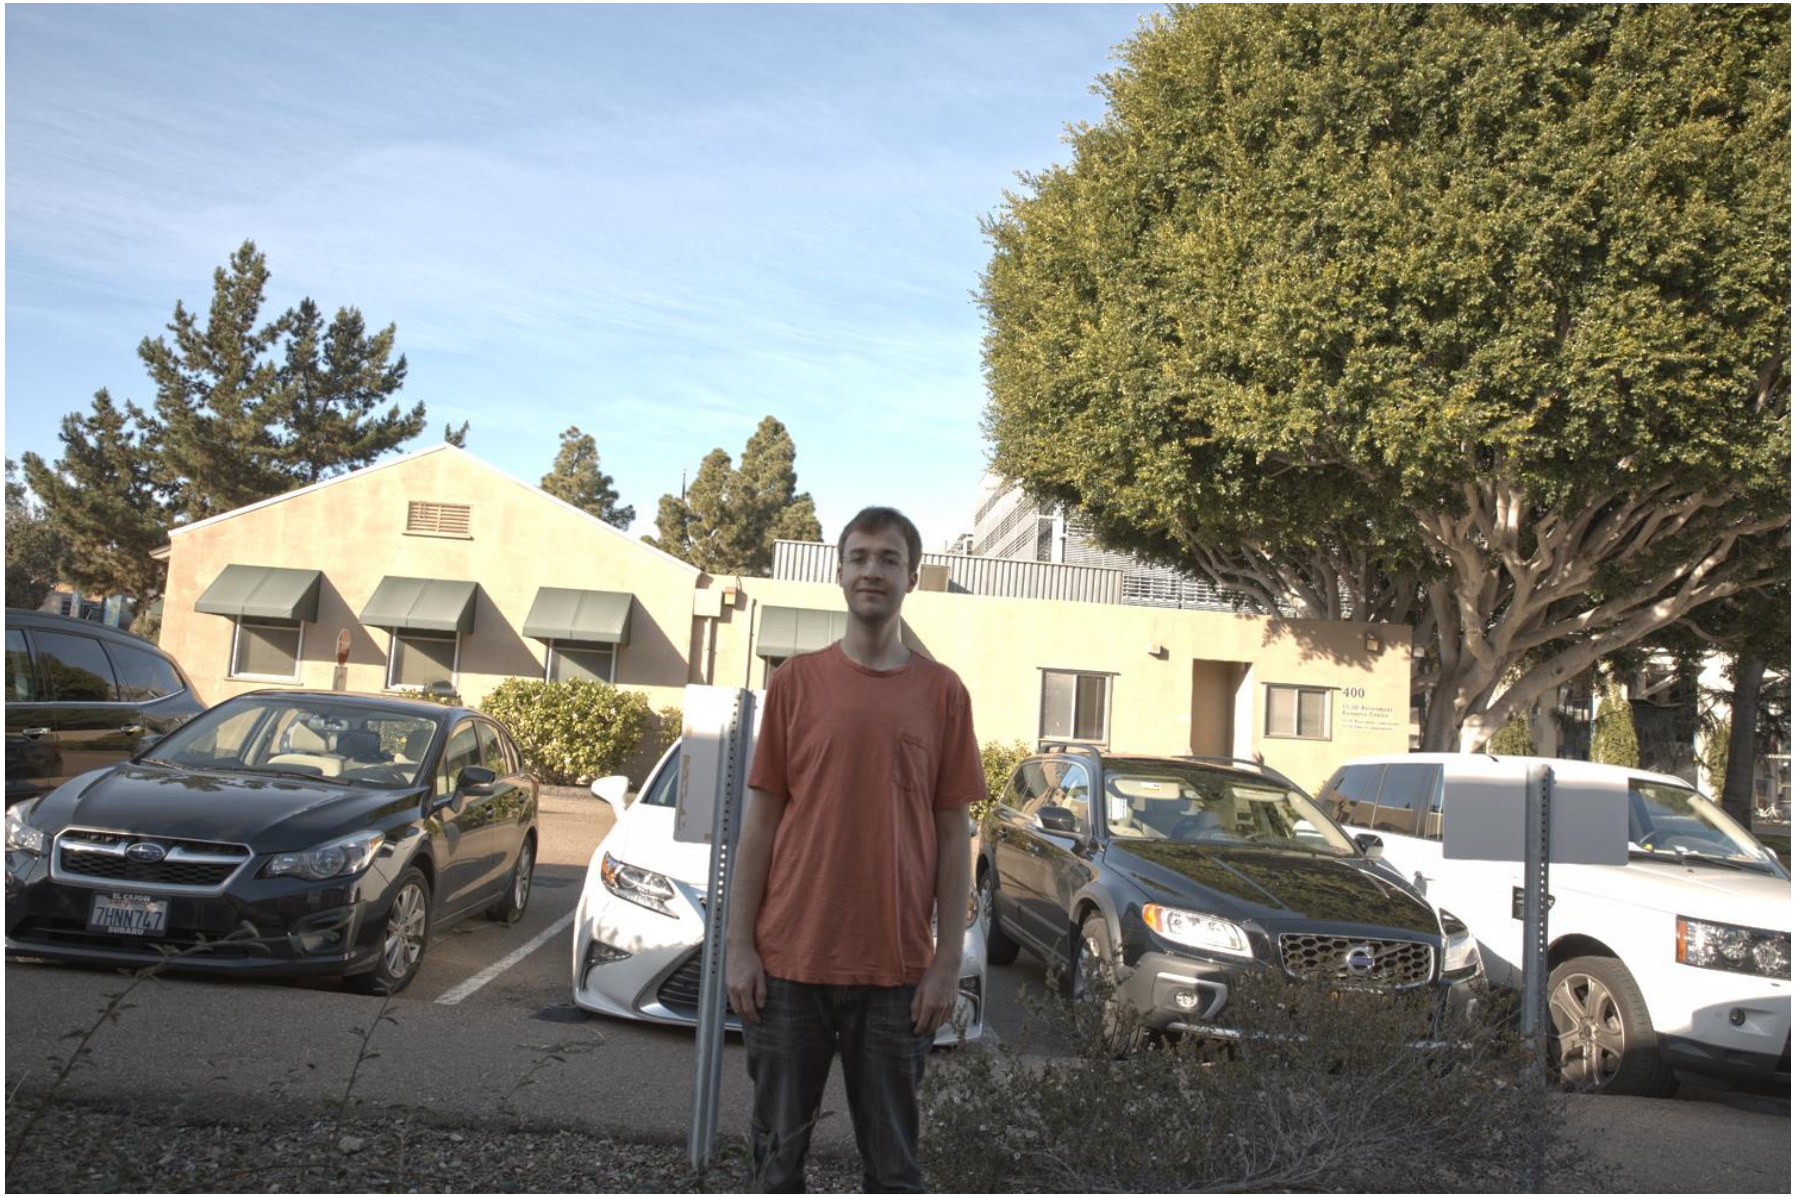

# 2. Comparison against state-of-the-art approaches (3 input LDR images)

# Scene No.1

# Input LDR image 1

Exposure Value: -2.0

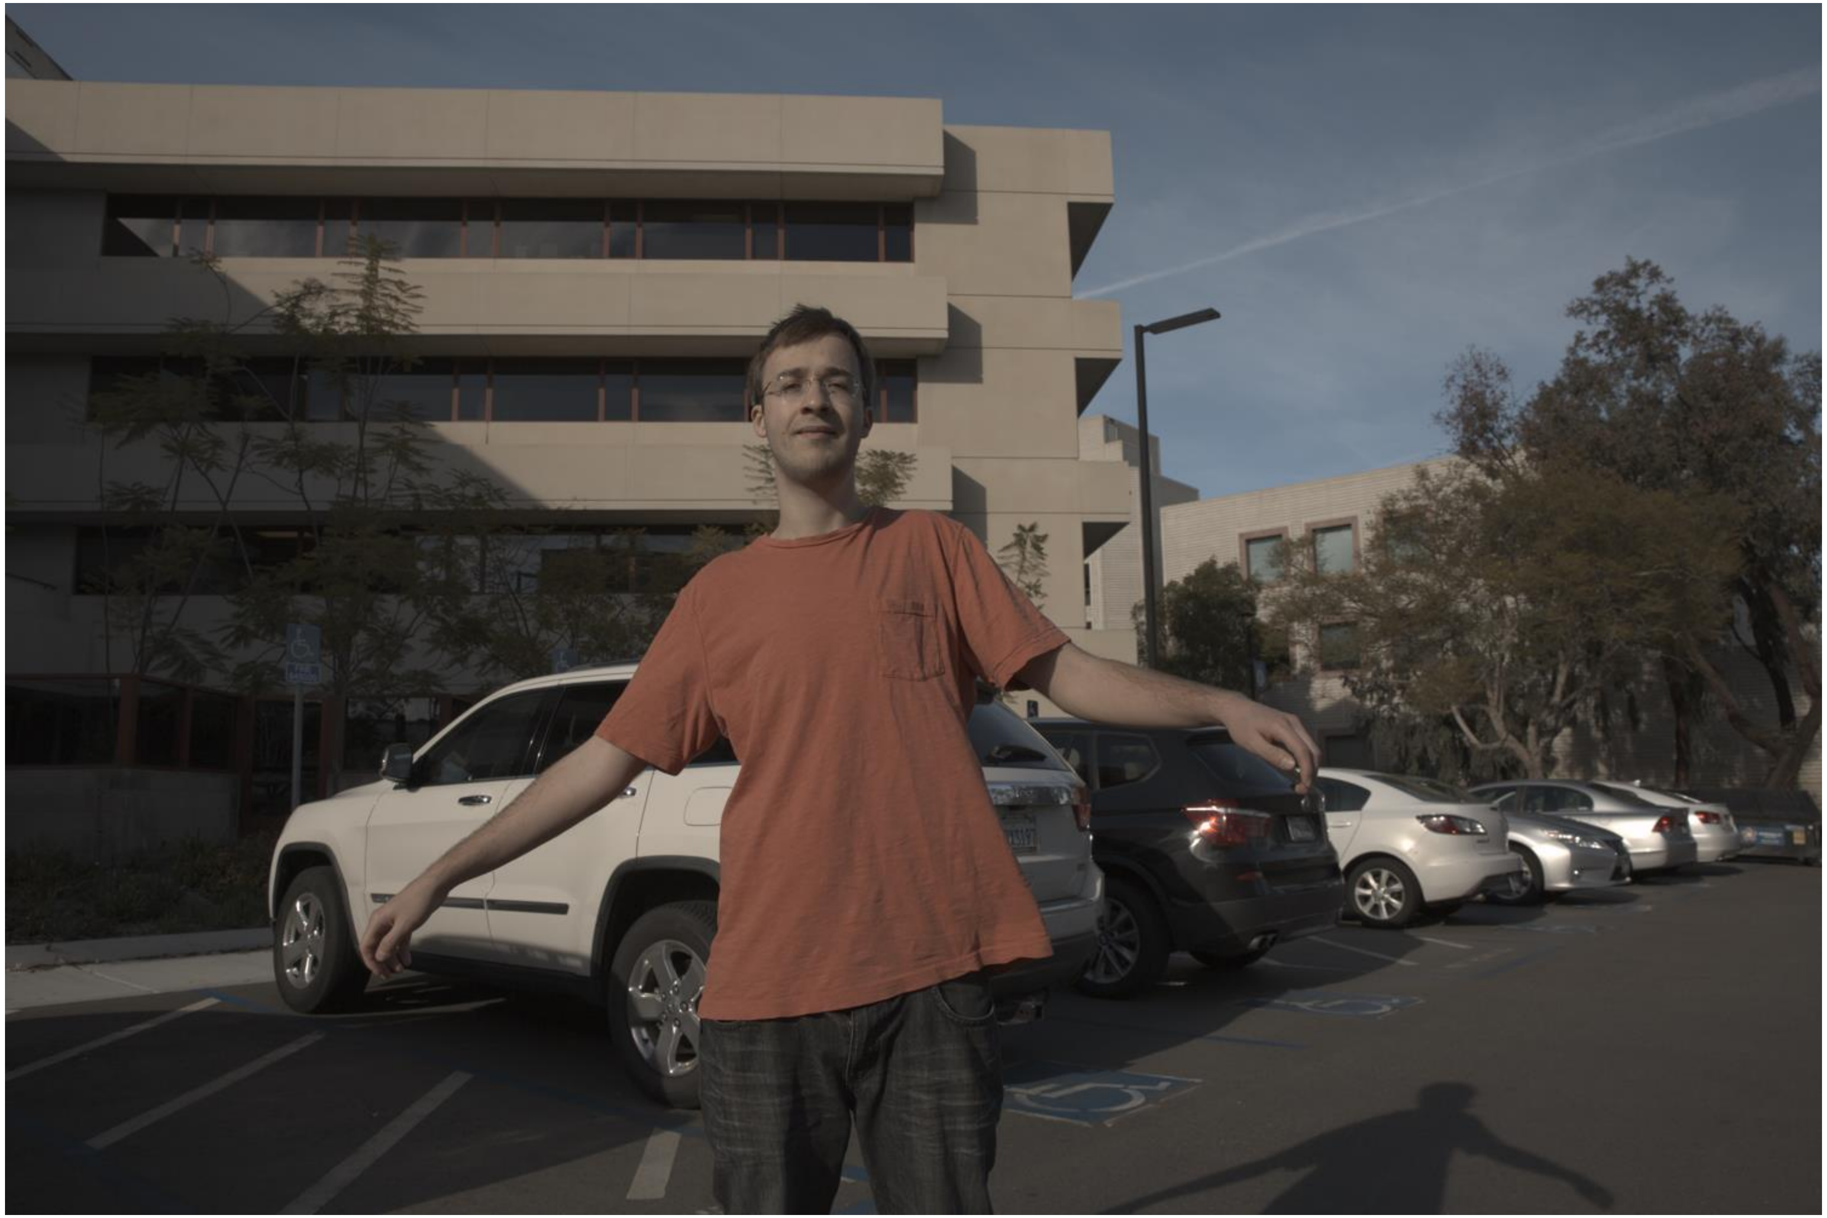

# Input LDR image 2

Exposure Value: 0.0

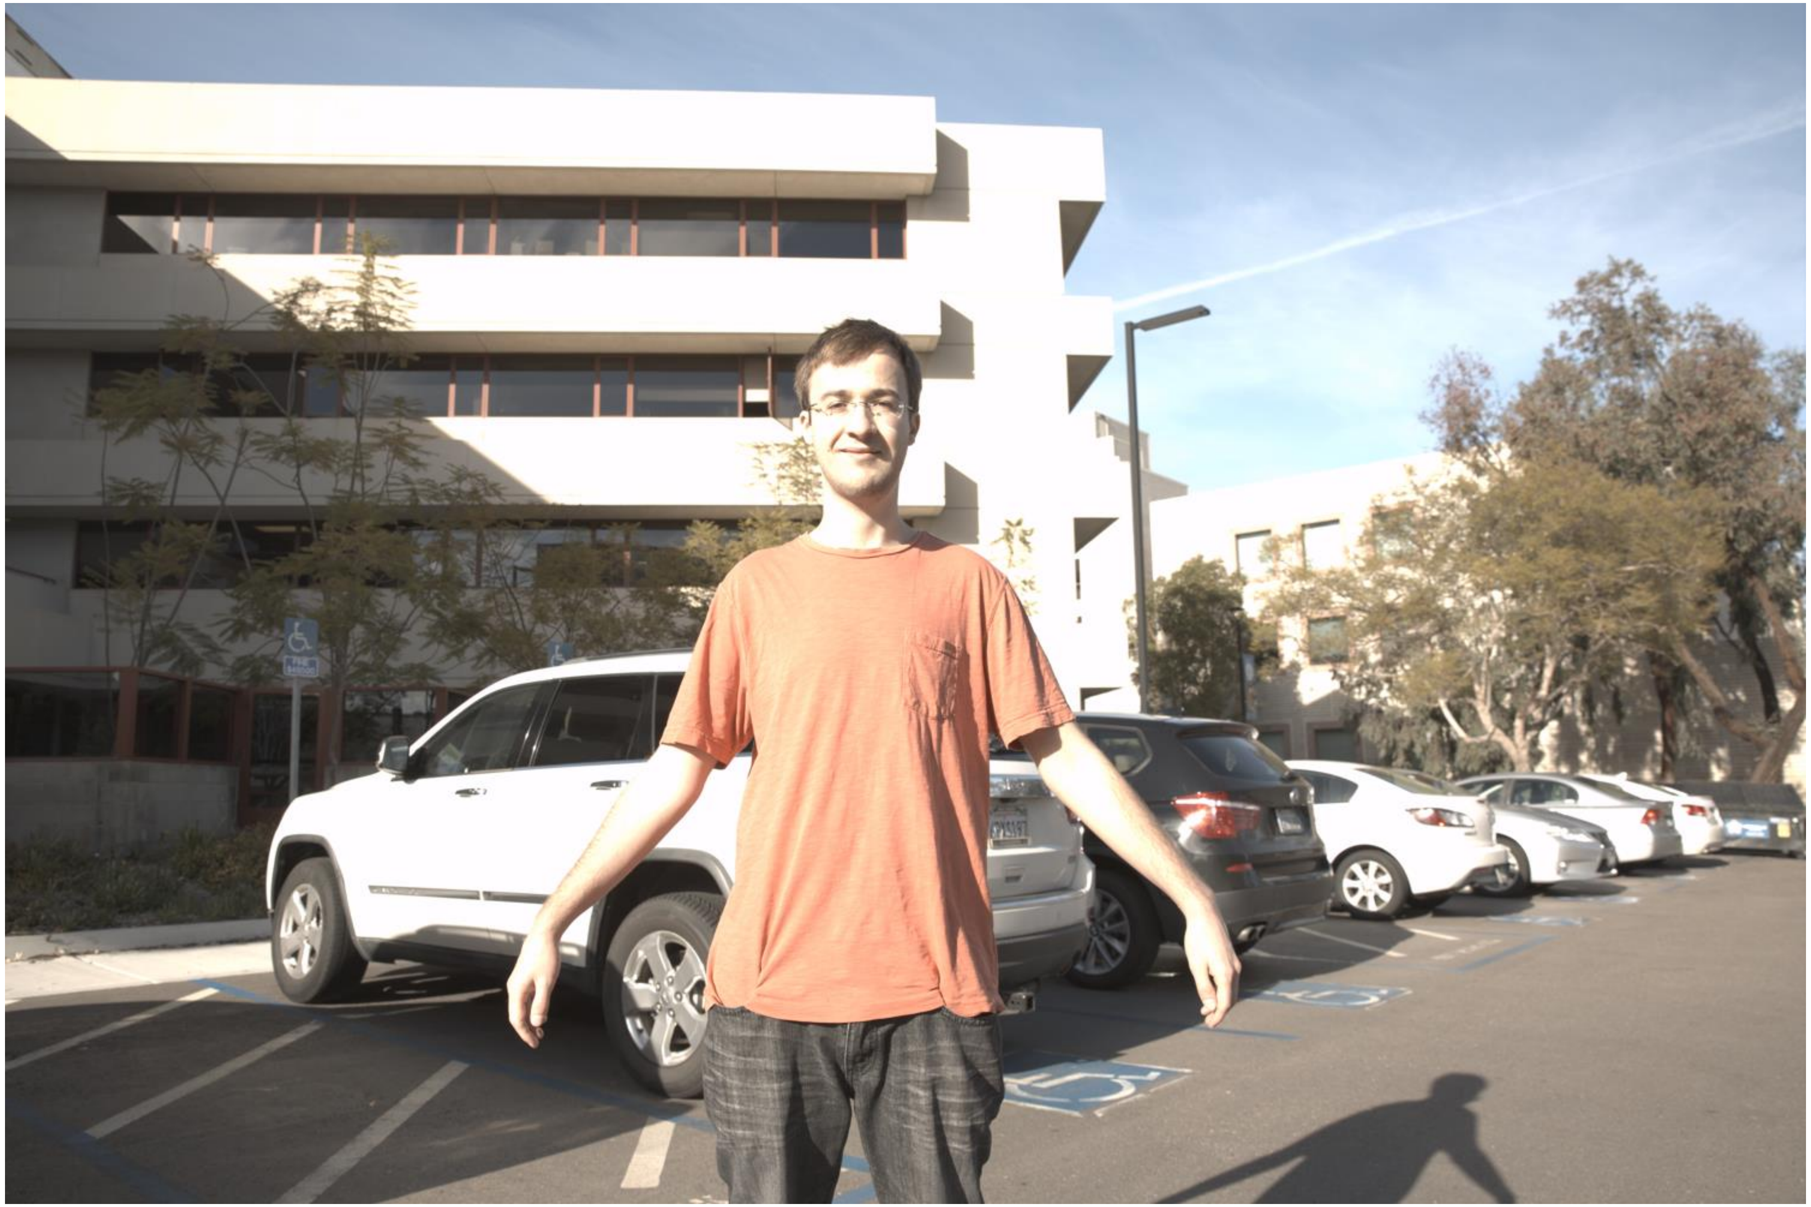

# Input LDR image 3

Exposure Value: +2.0

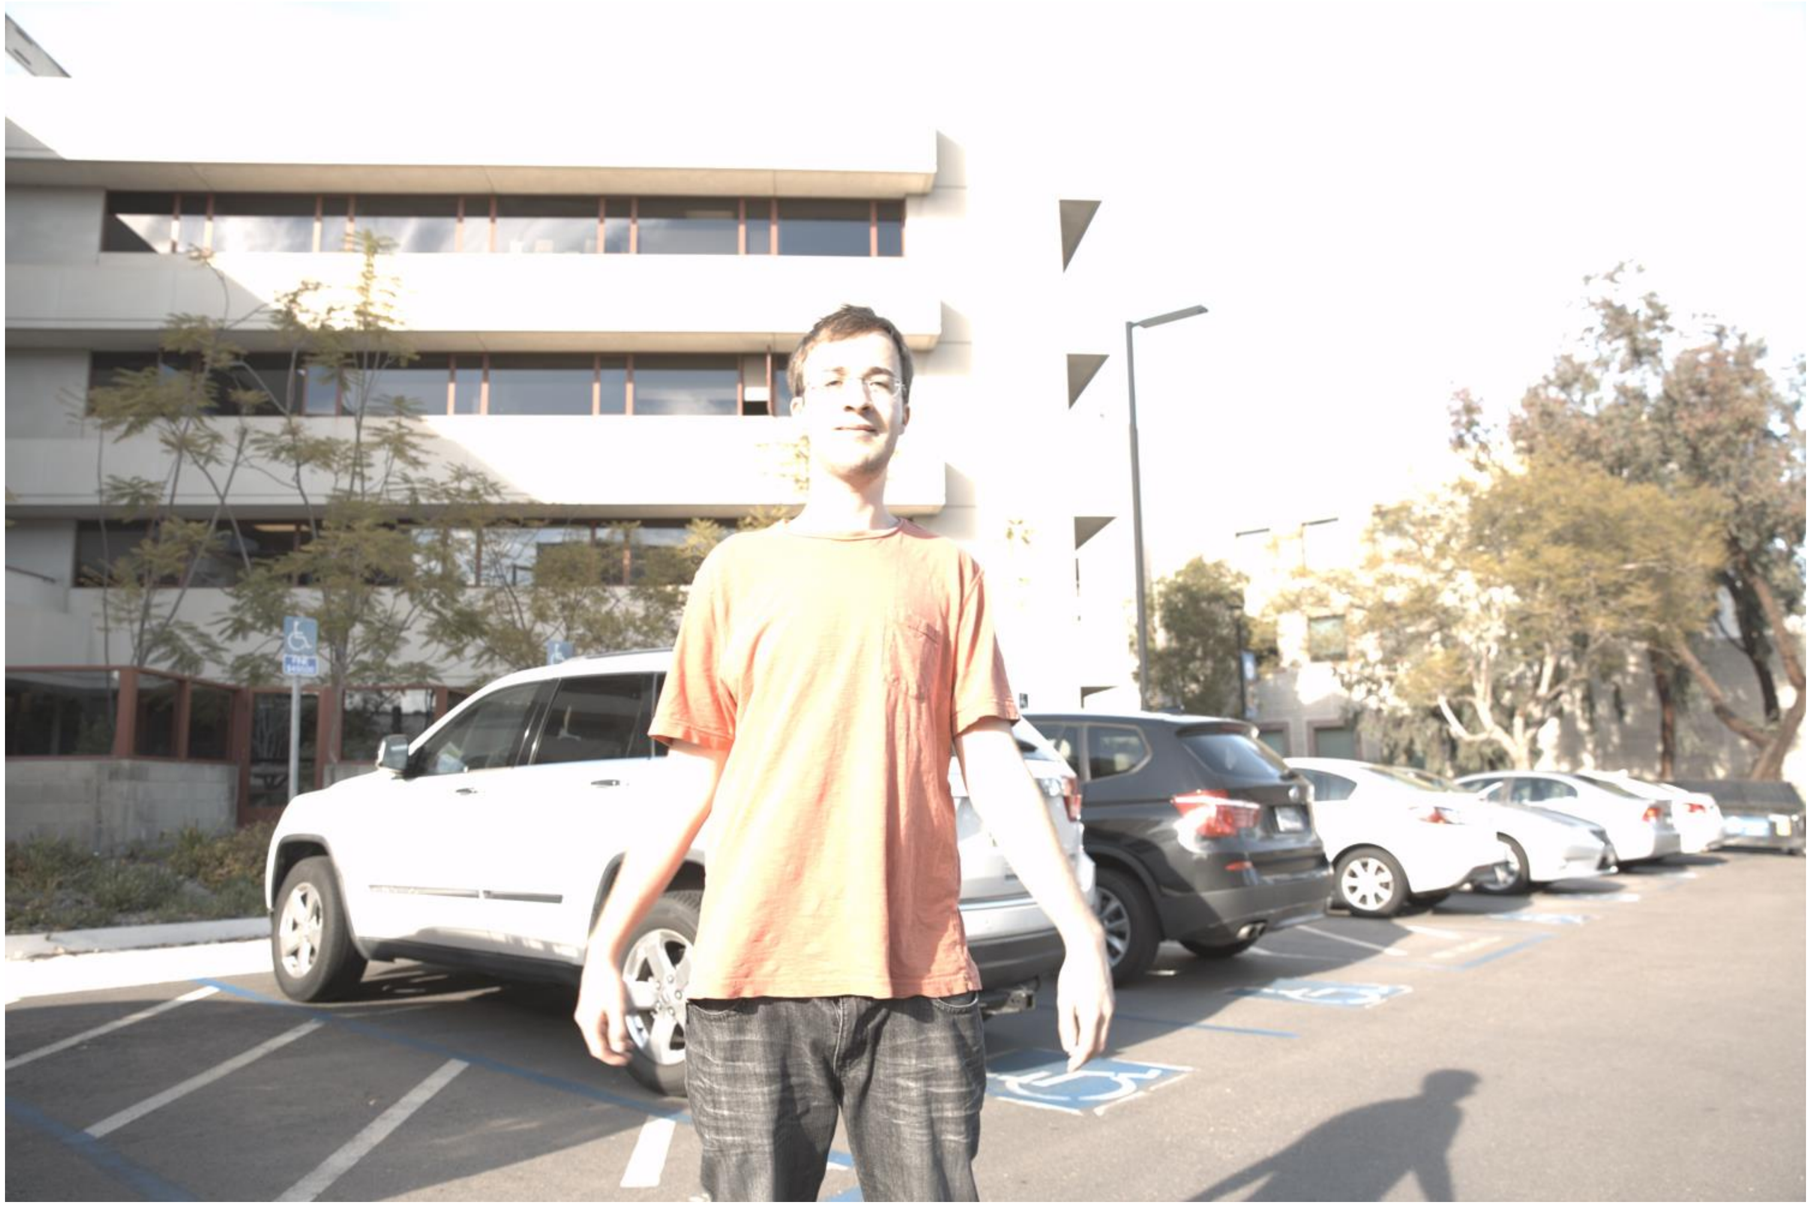

# HDR result
Sen et al. [2012]

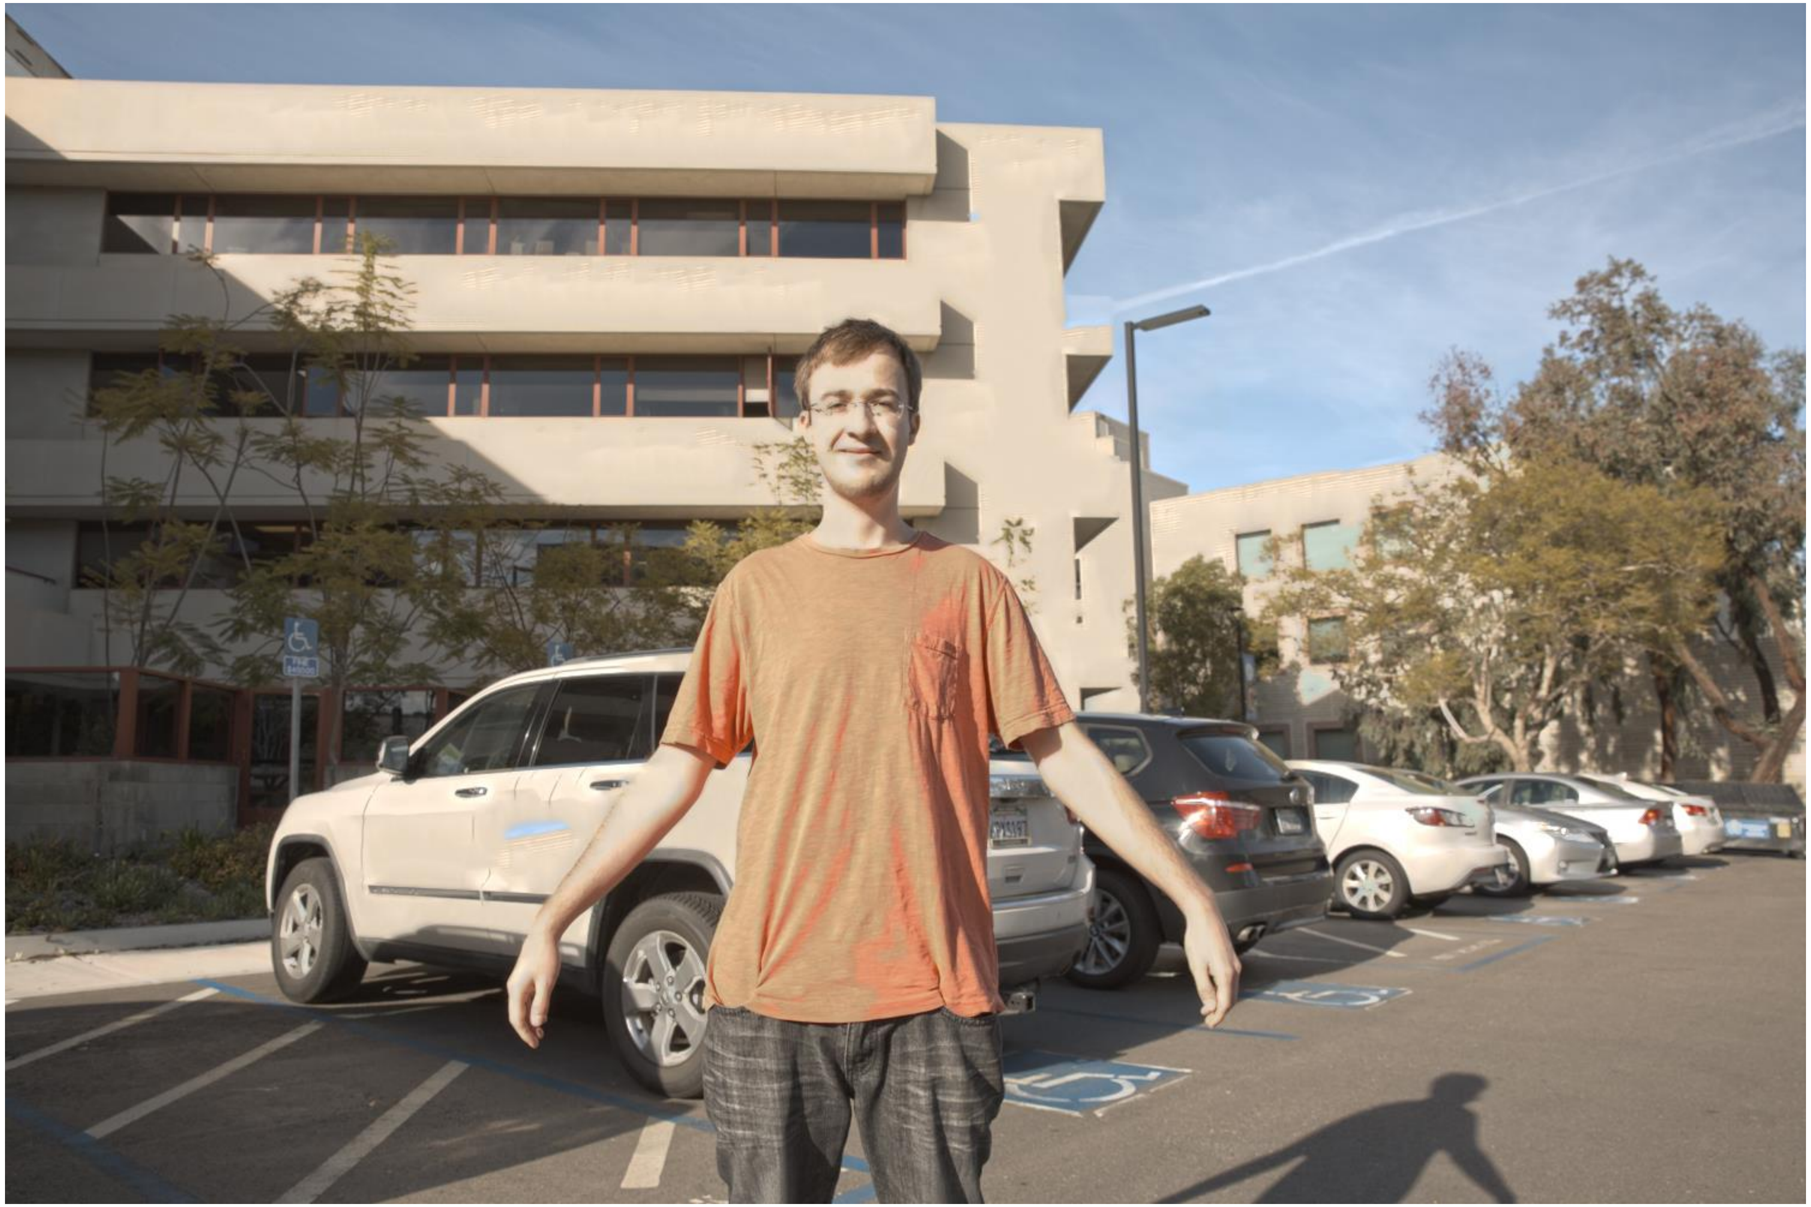

# HDR result

Kalantari et al. [2017]

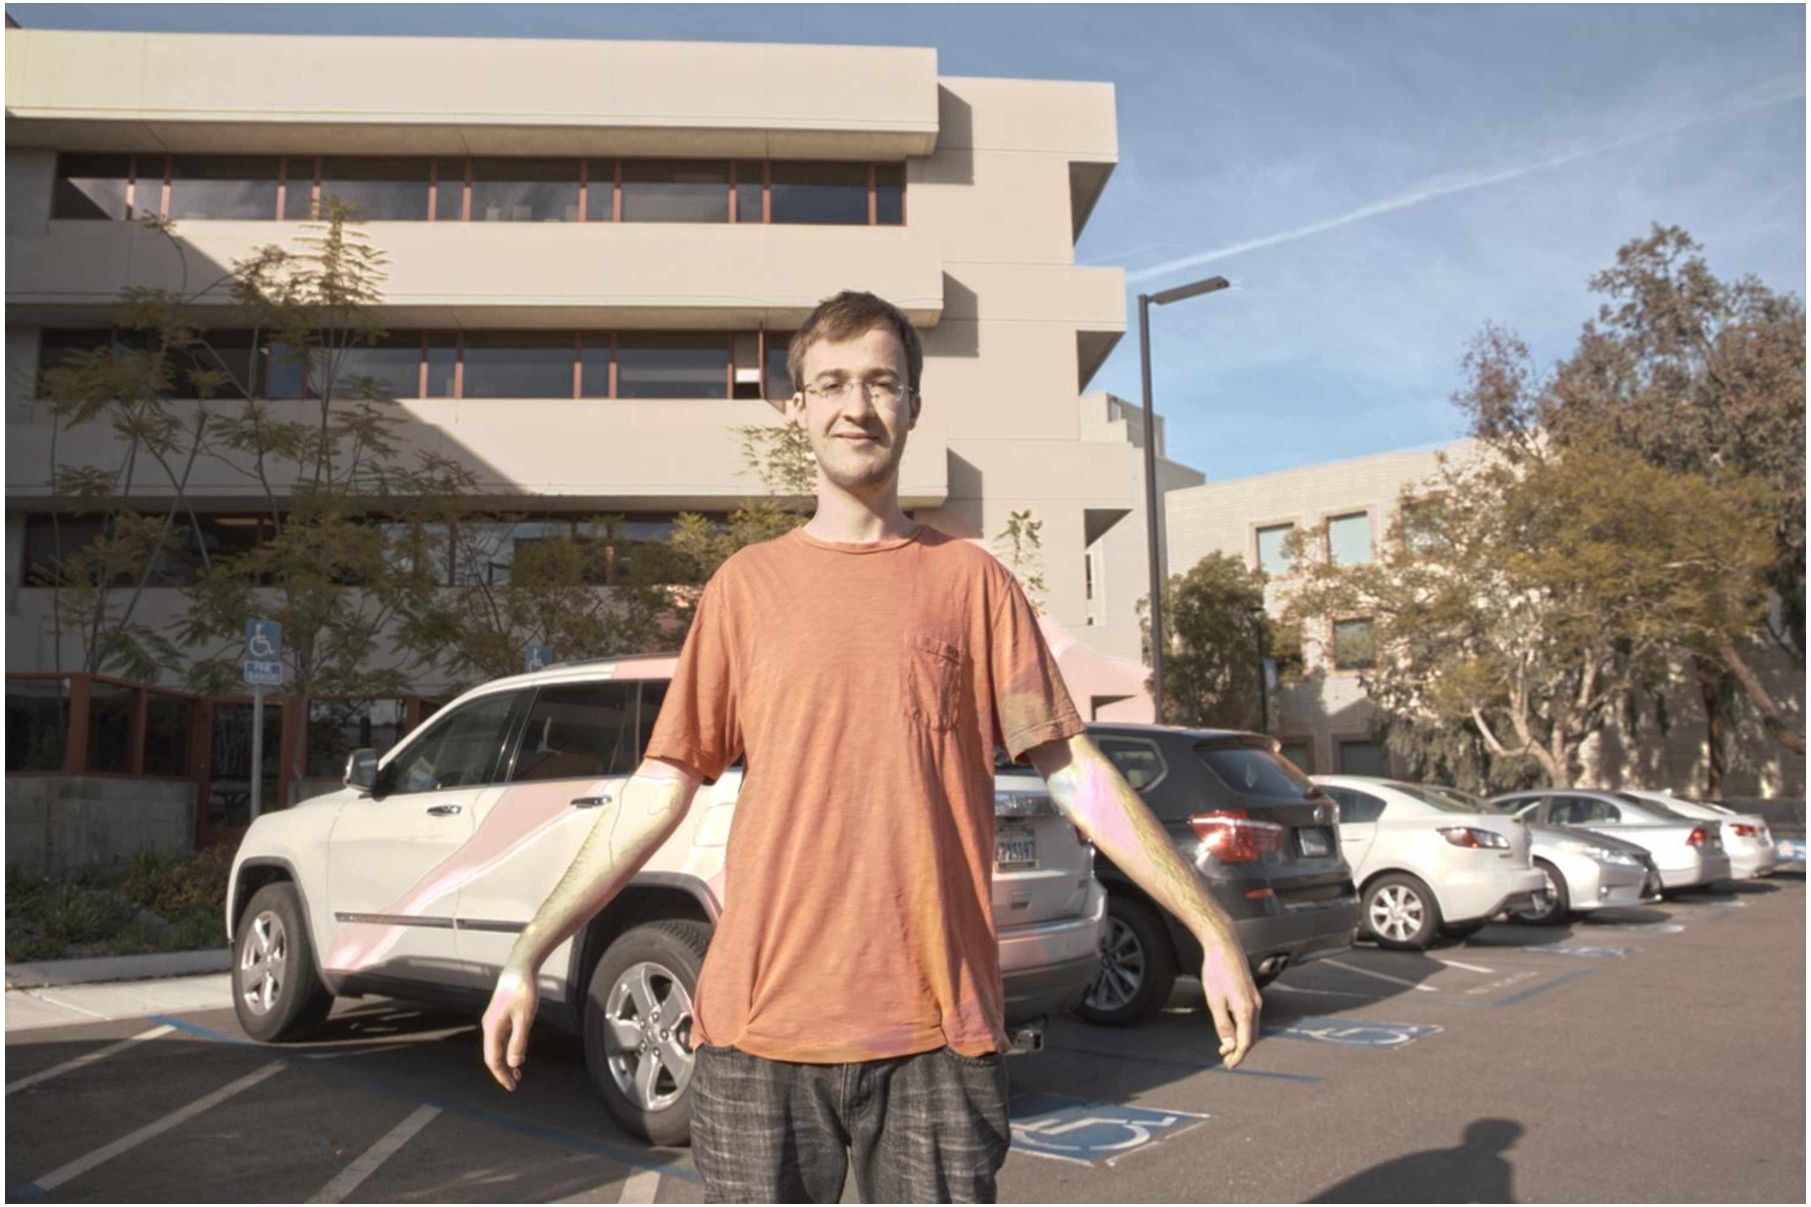

# HDR result
Wu et al. [2018]

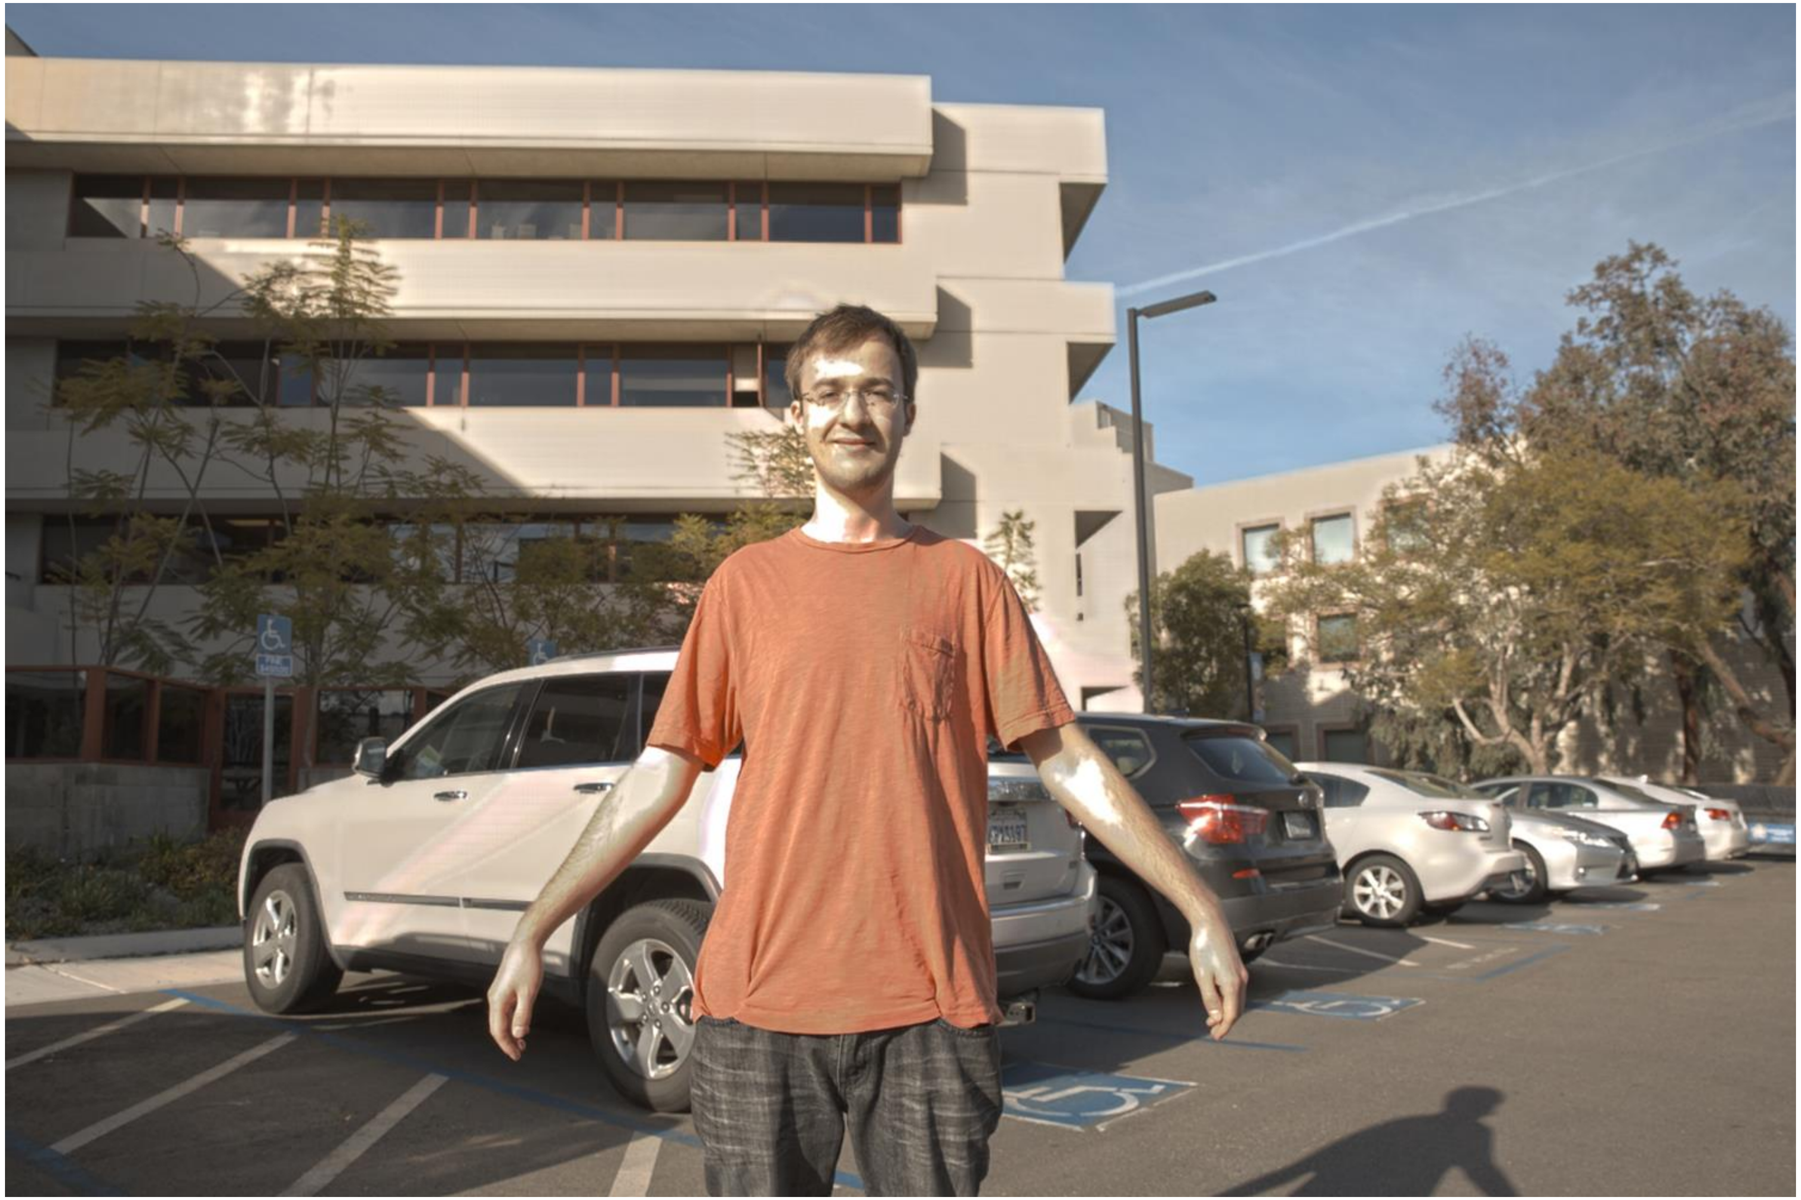

# HDR result
Yan et al. [2019]

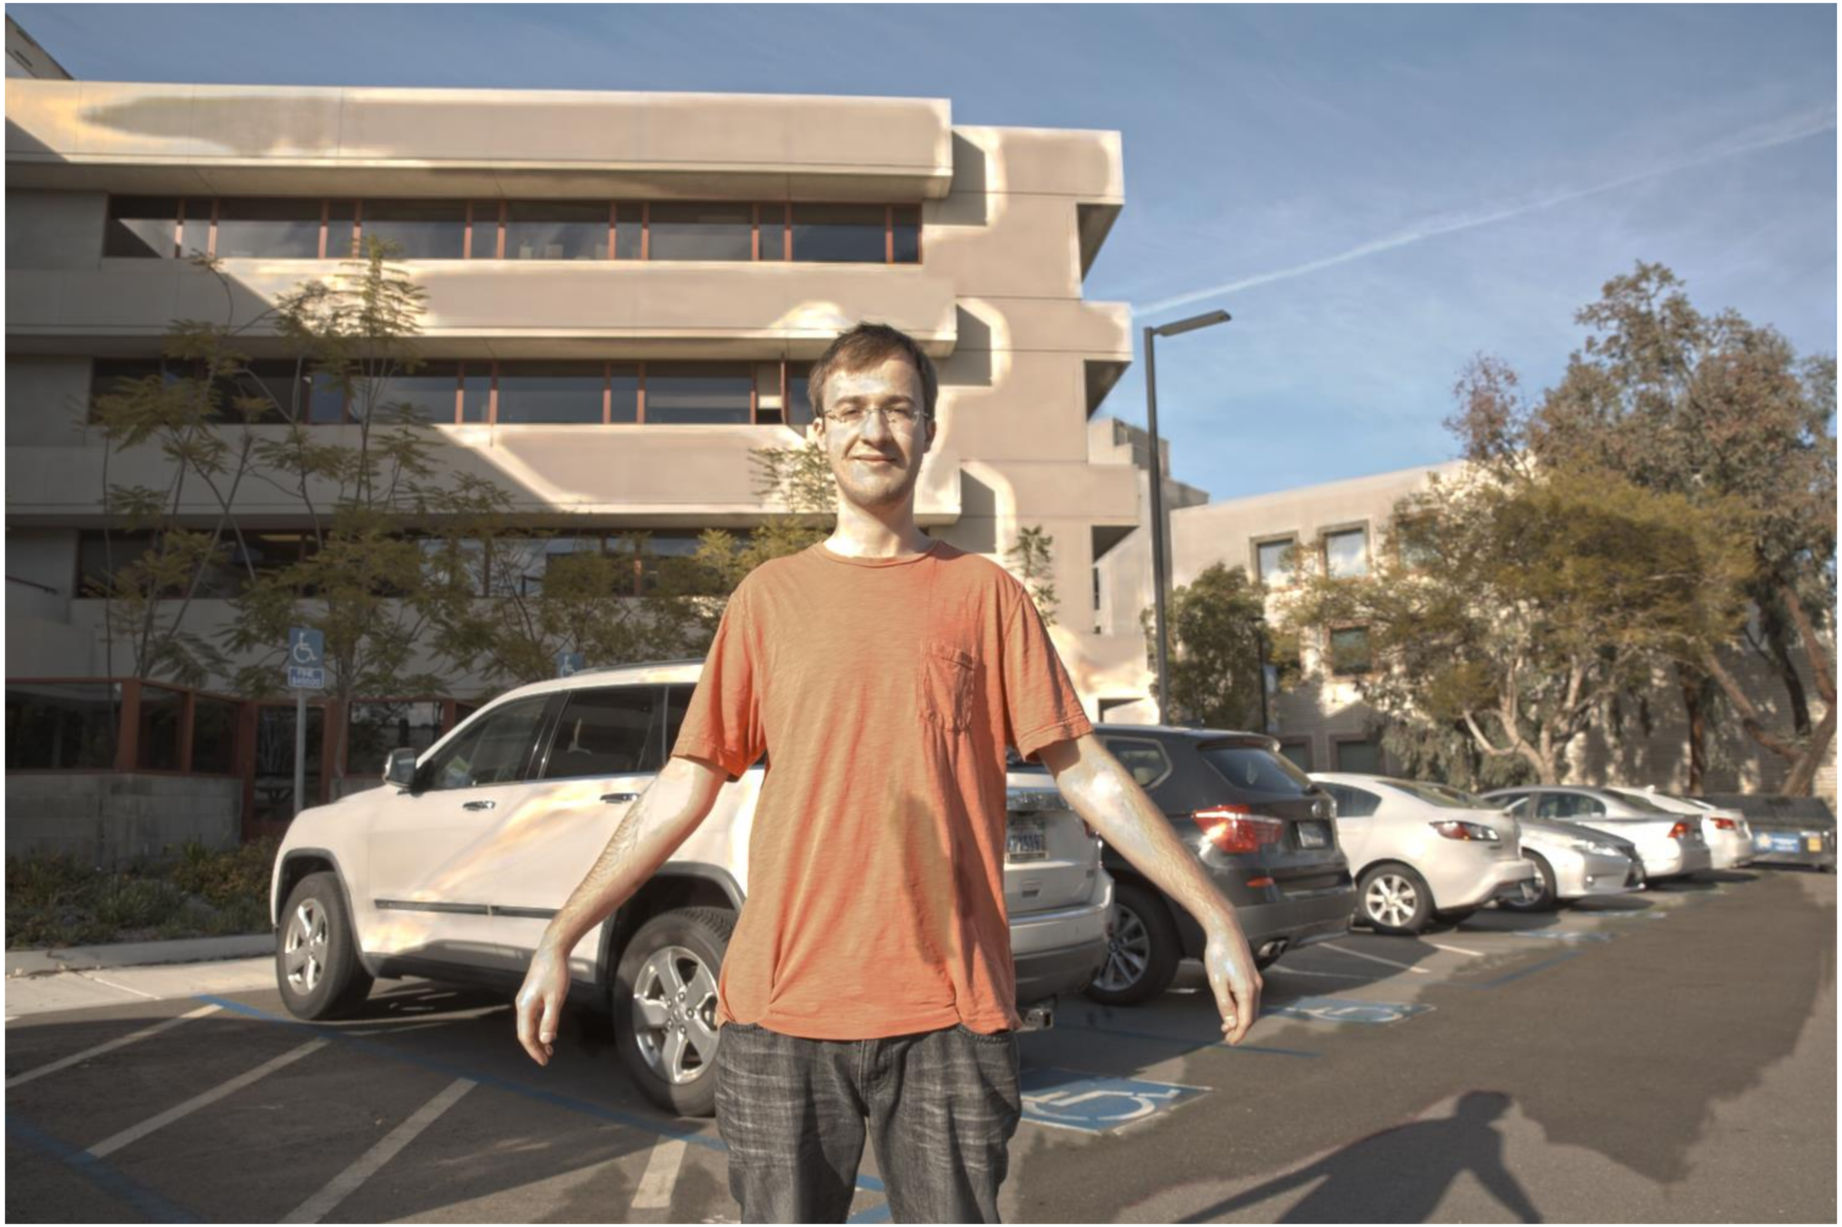

# HDR result

Li et al. [2020]

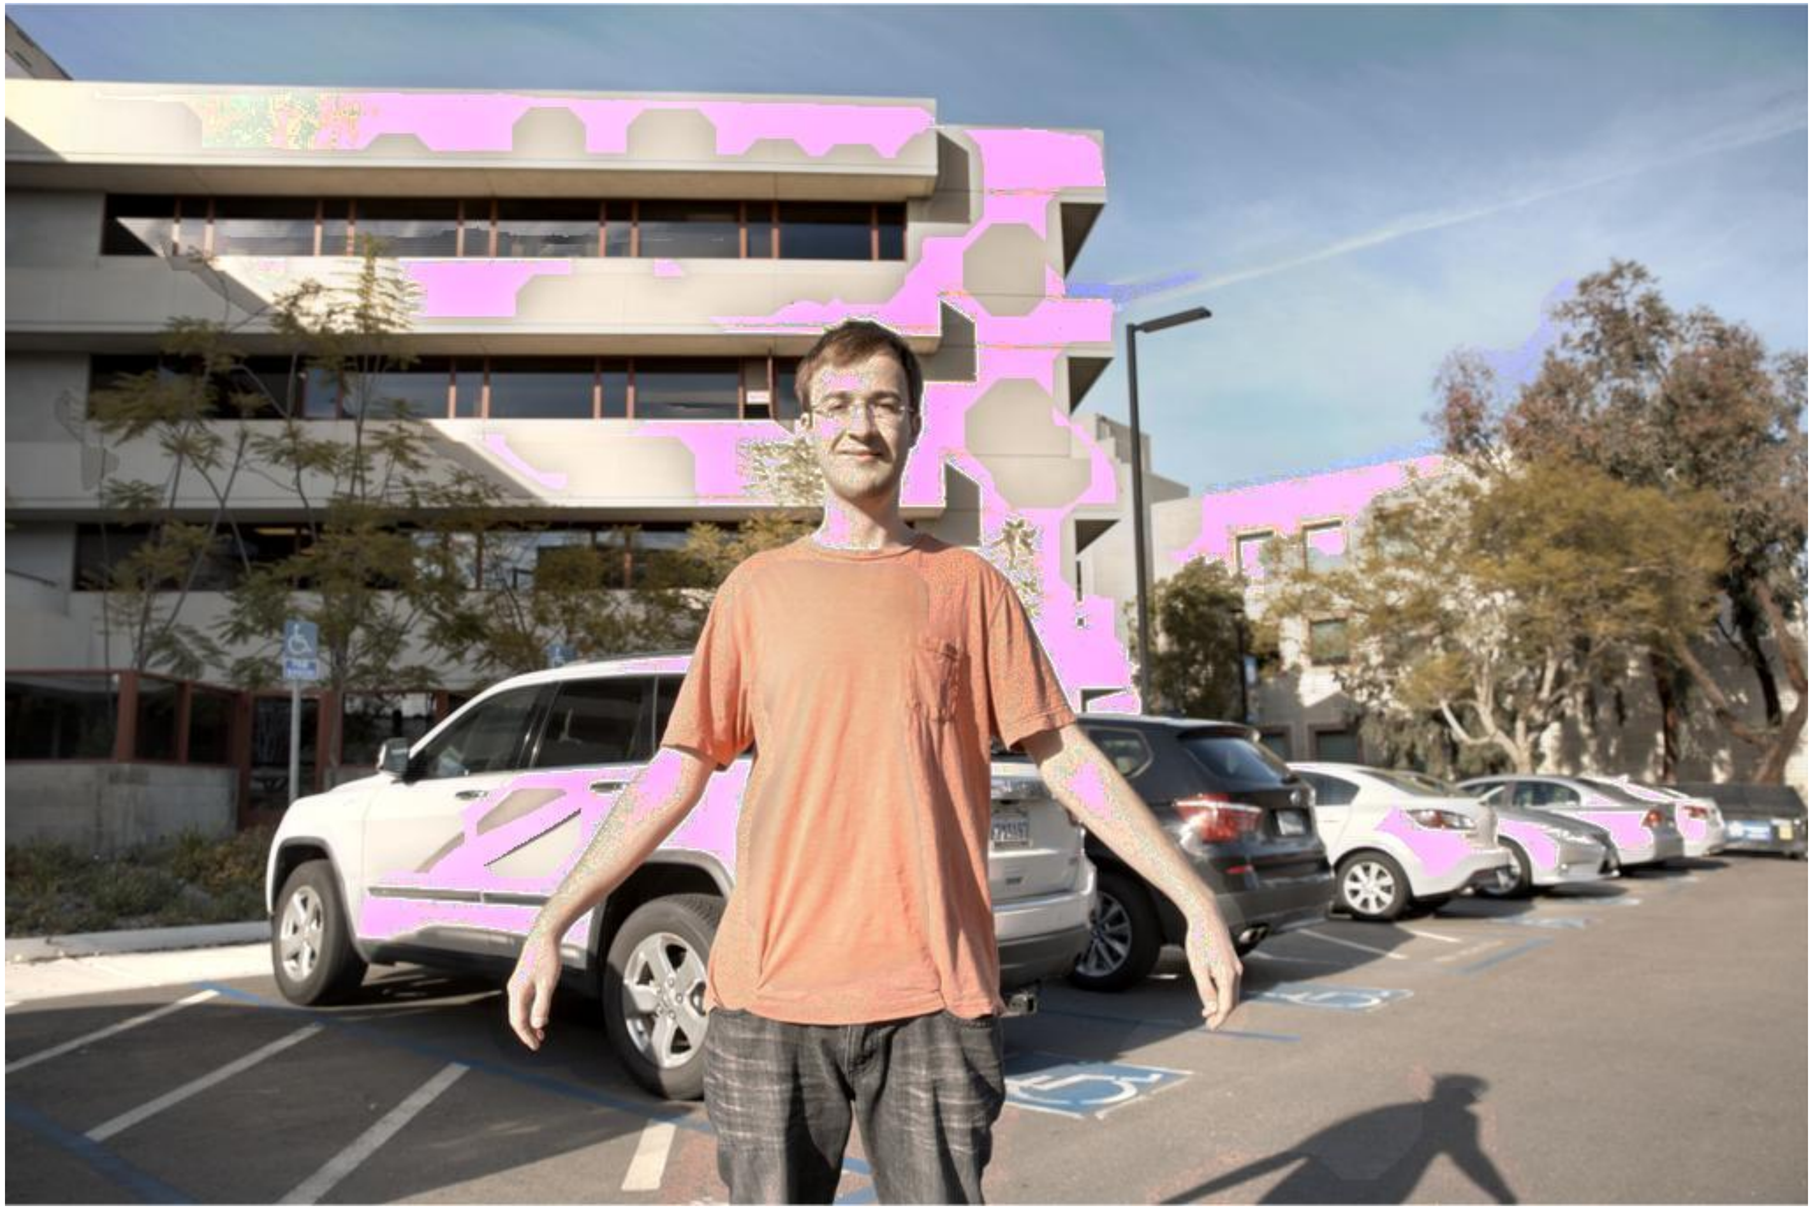

# HDR result

Niu et al. [2021]

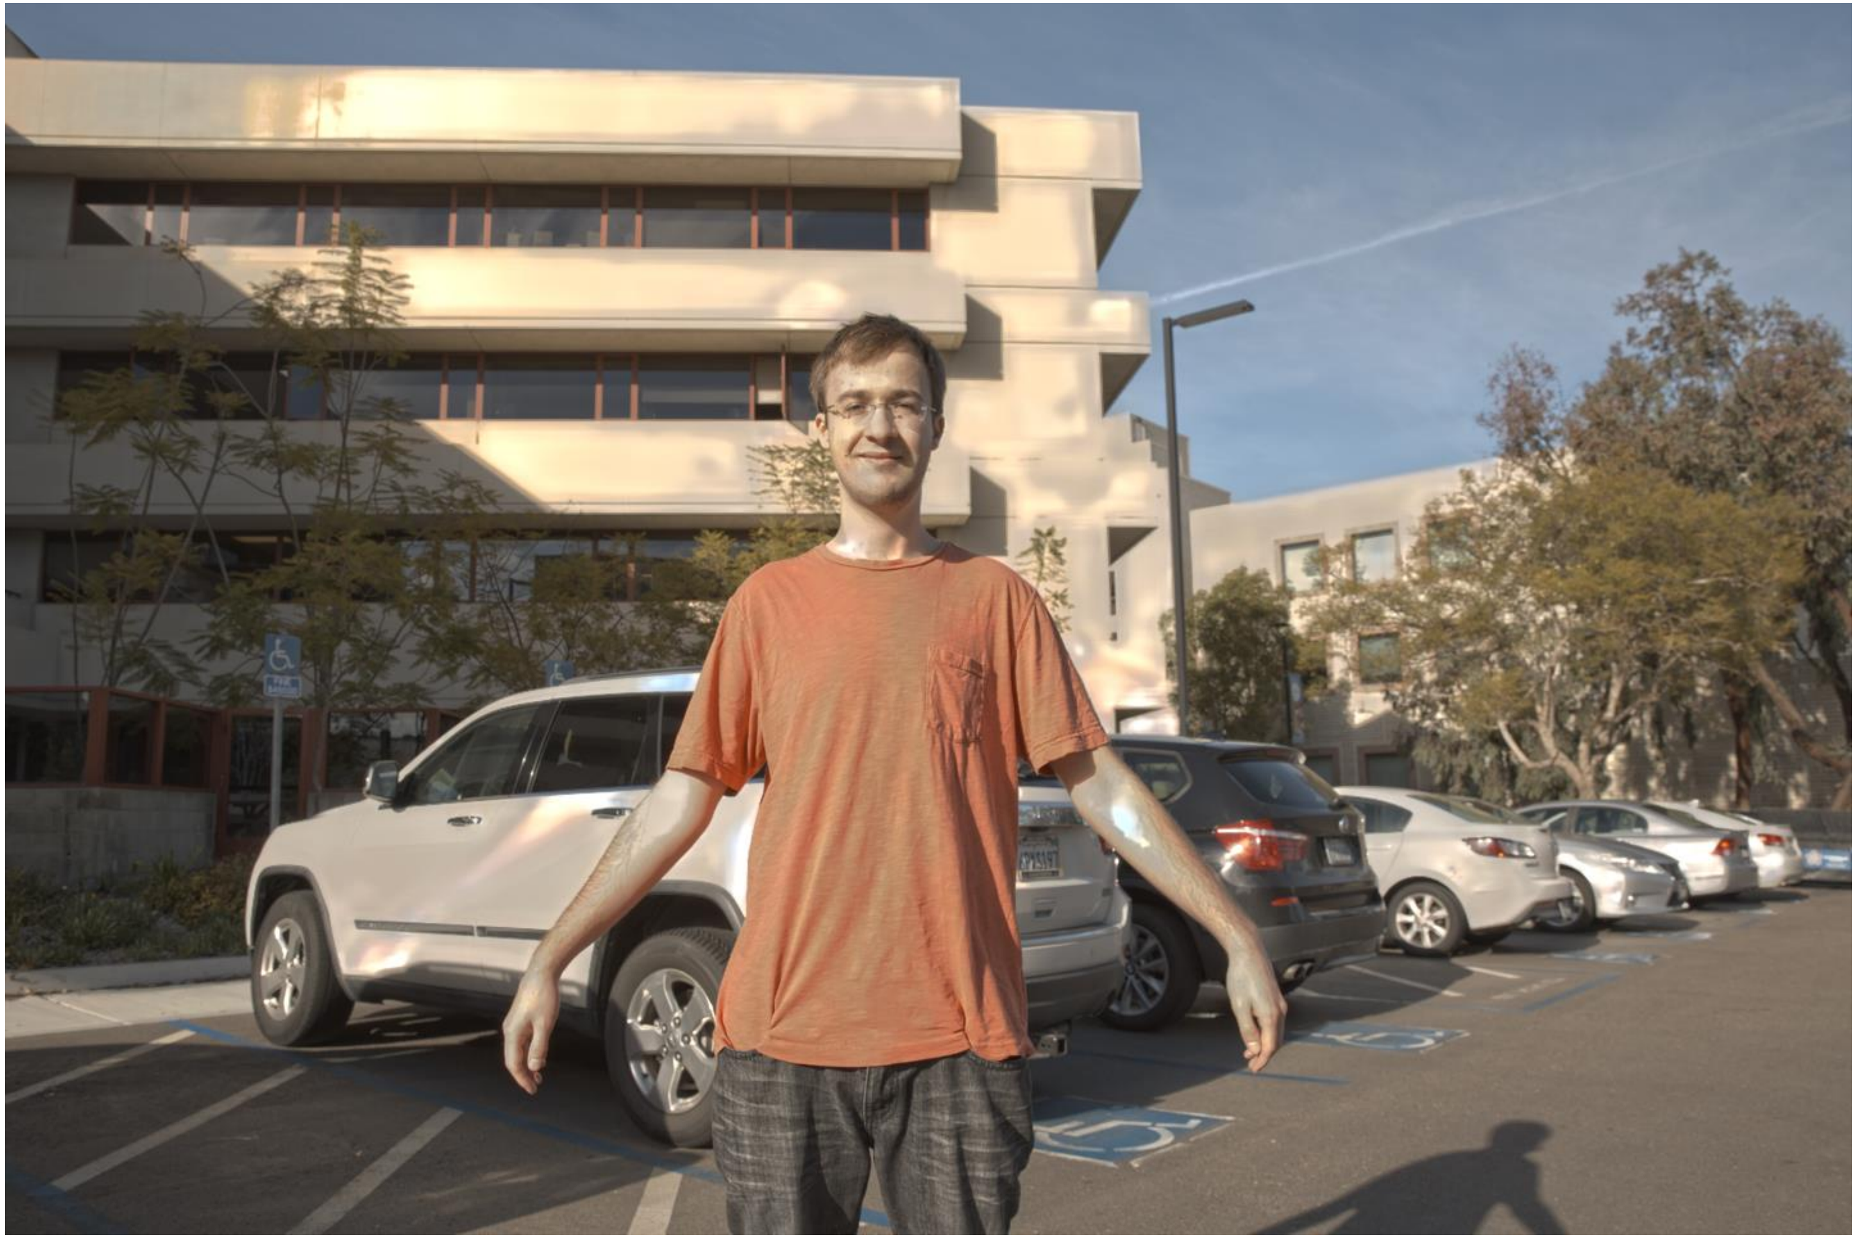

# HDR result
Ours

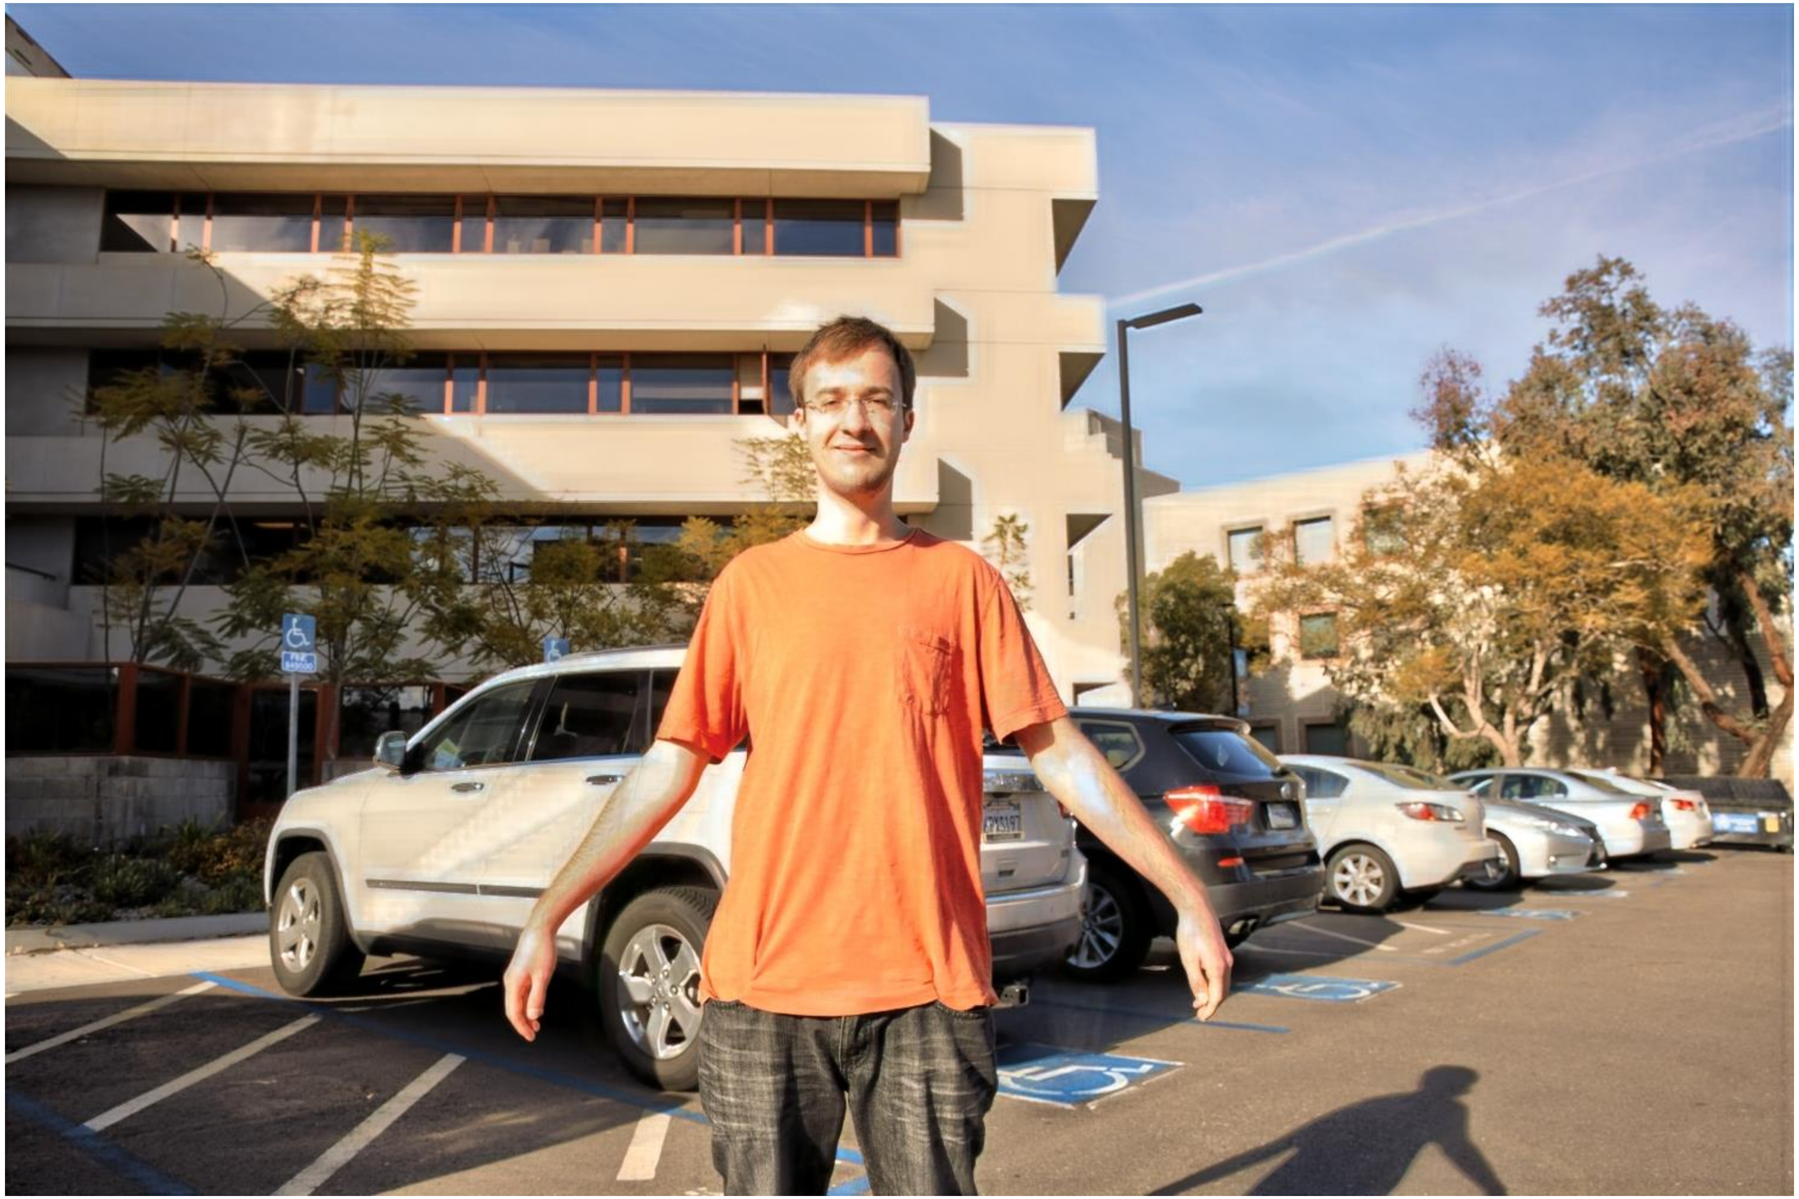

# HDR
Ground Truth

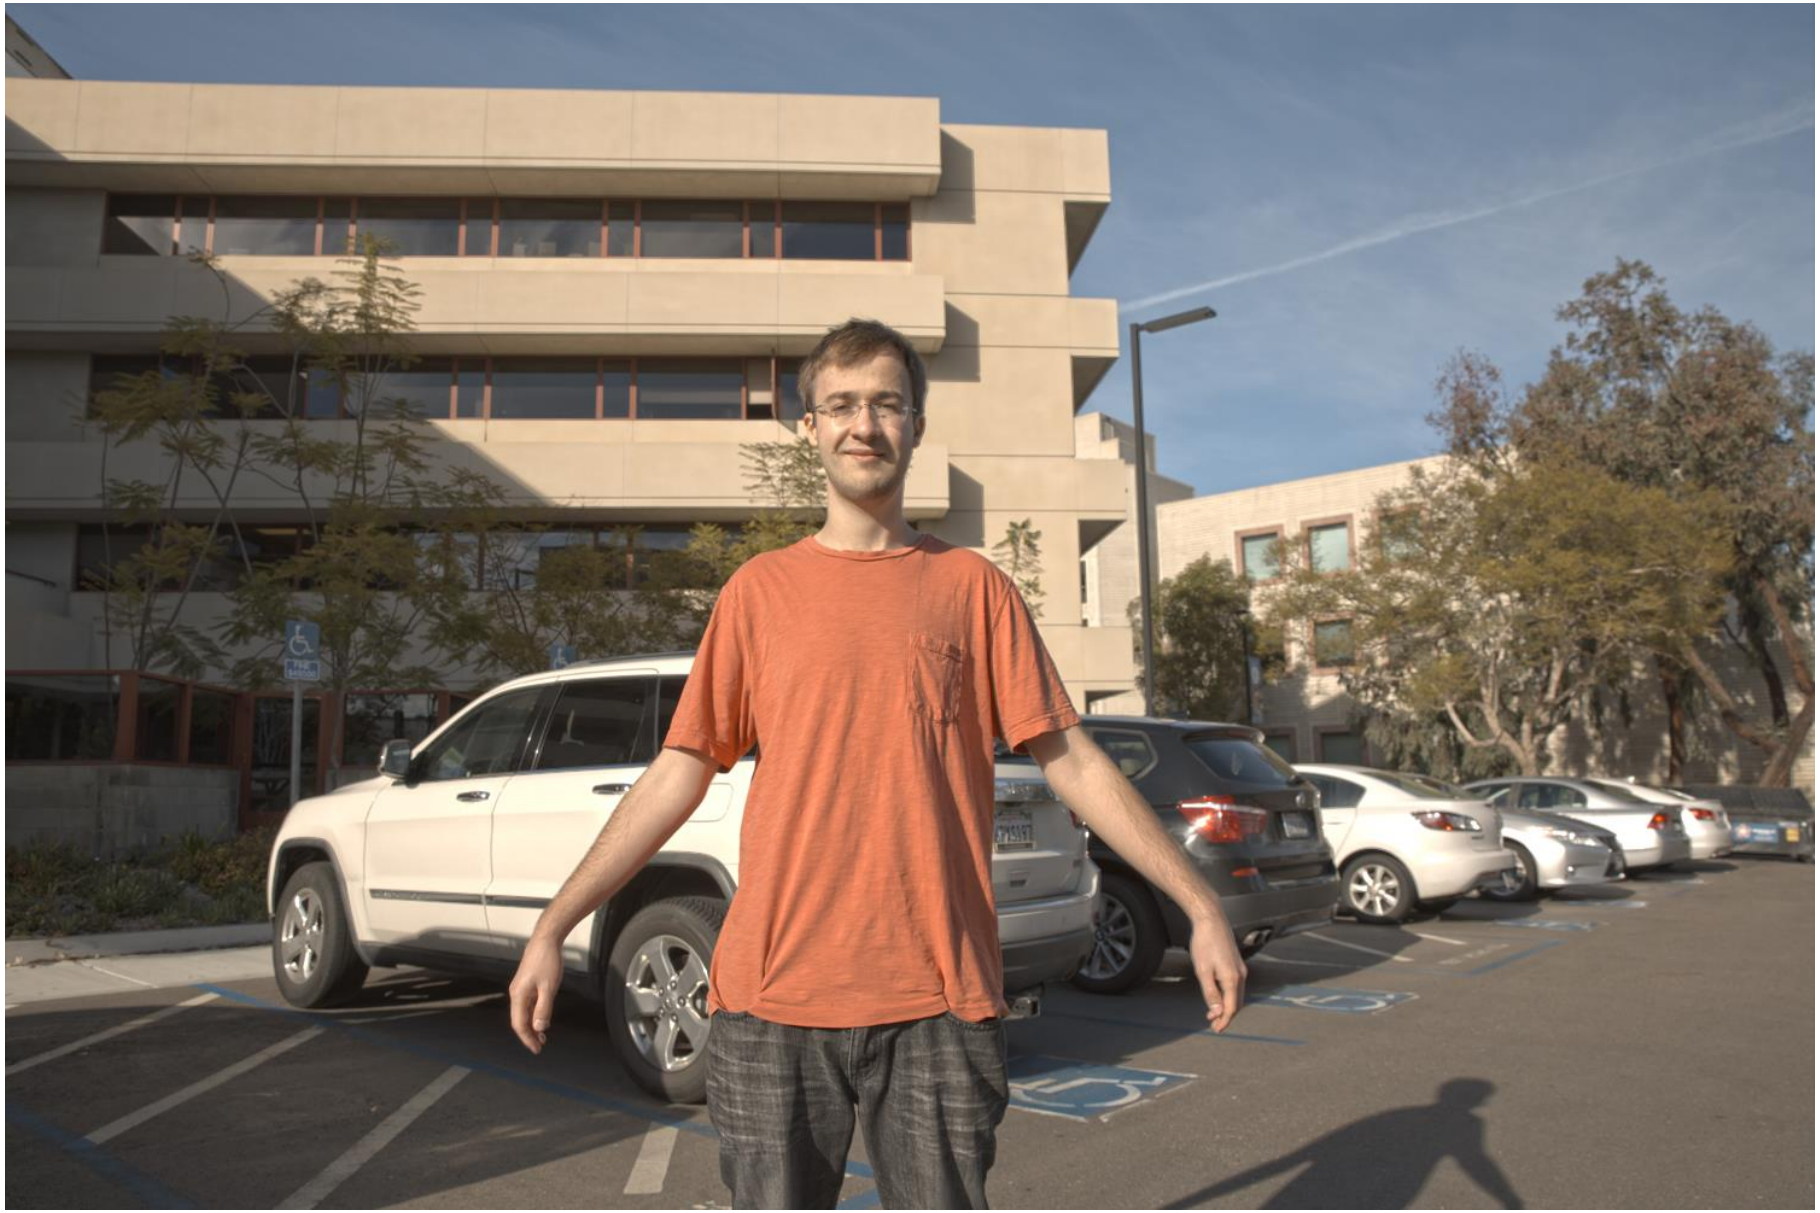

# Scene No.2

# Input LDR image 1
Exposure Value: -2.0

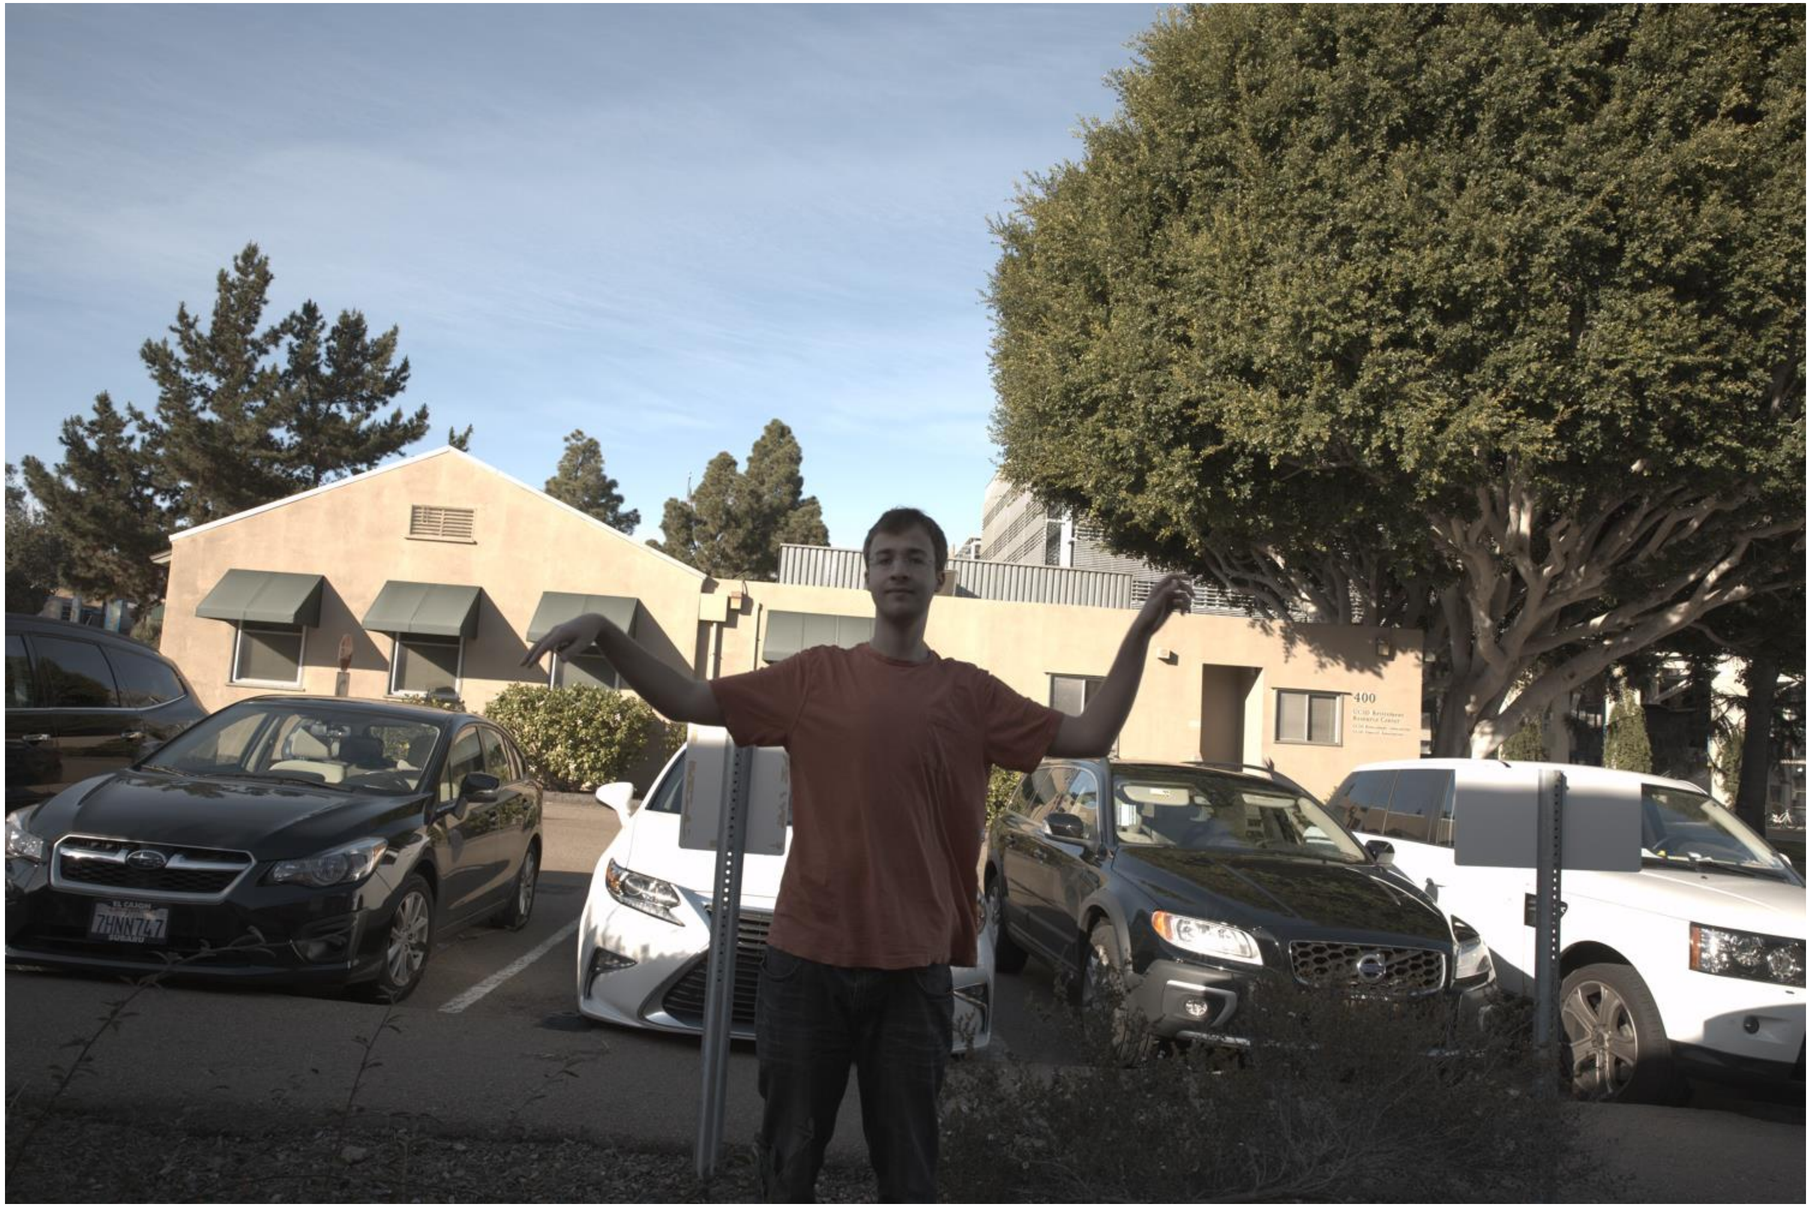

# Input LDR image 2

Exposure Value: 0.0

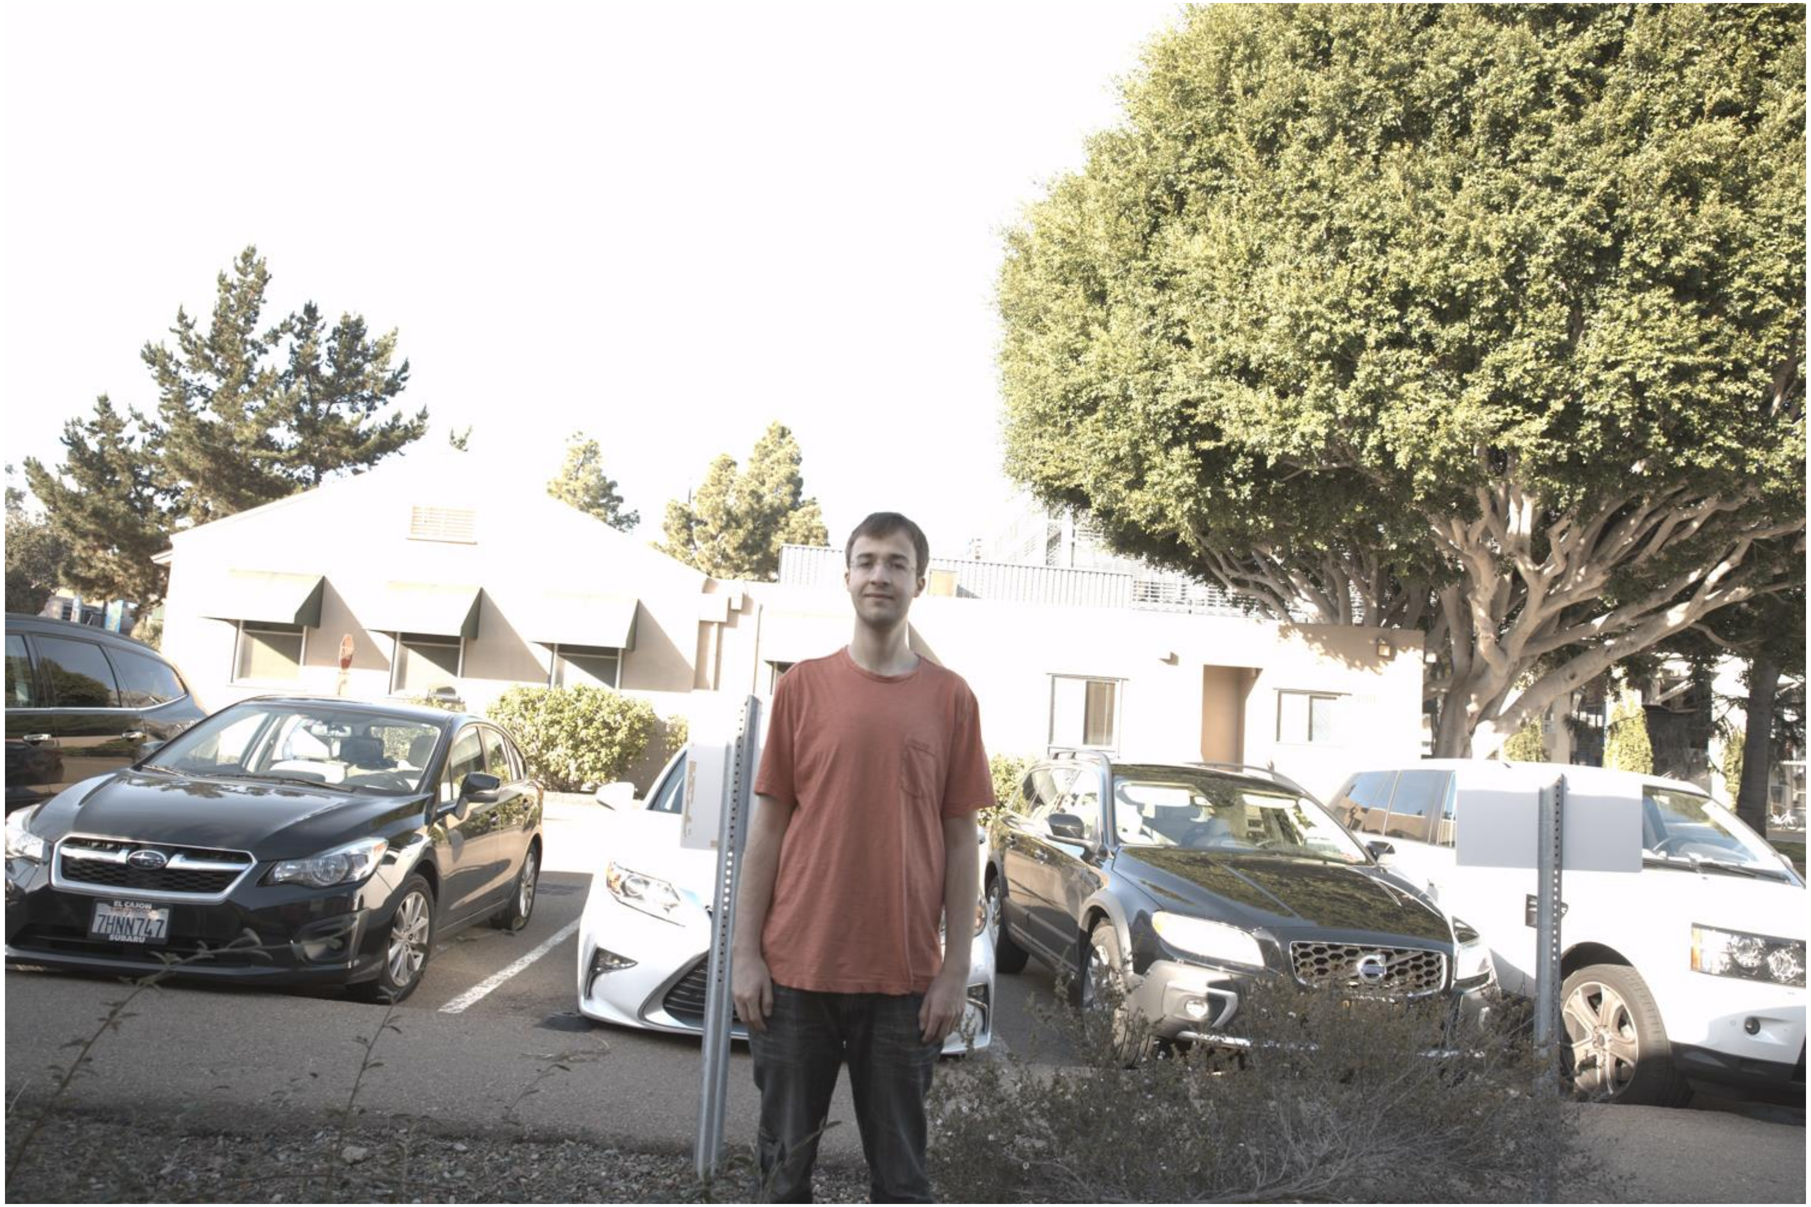

# Input LDR image 3
Exposure Value: +2.0

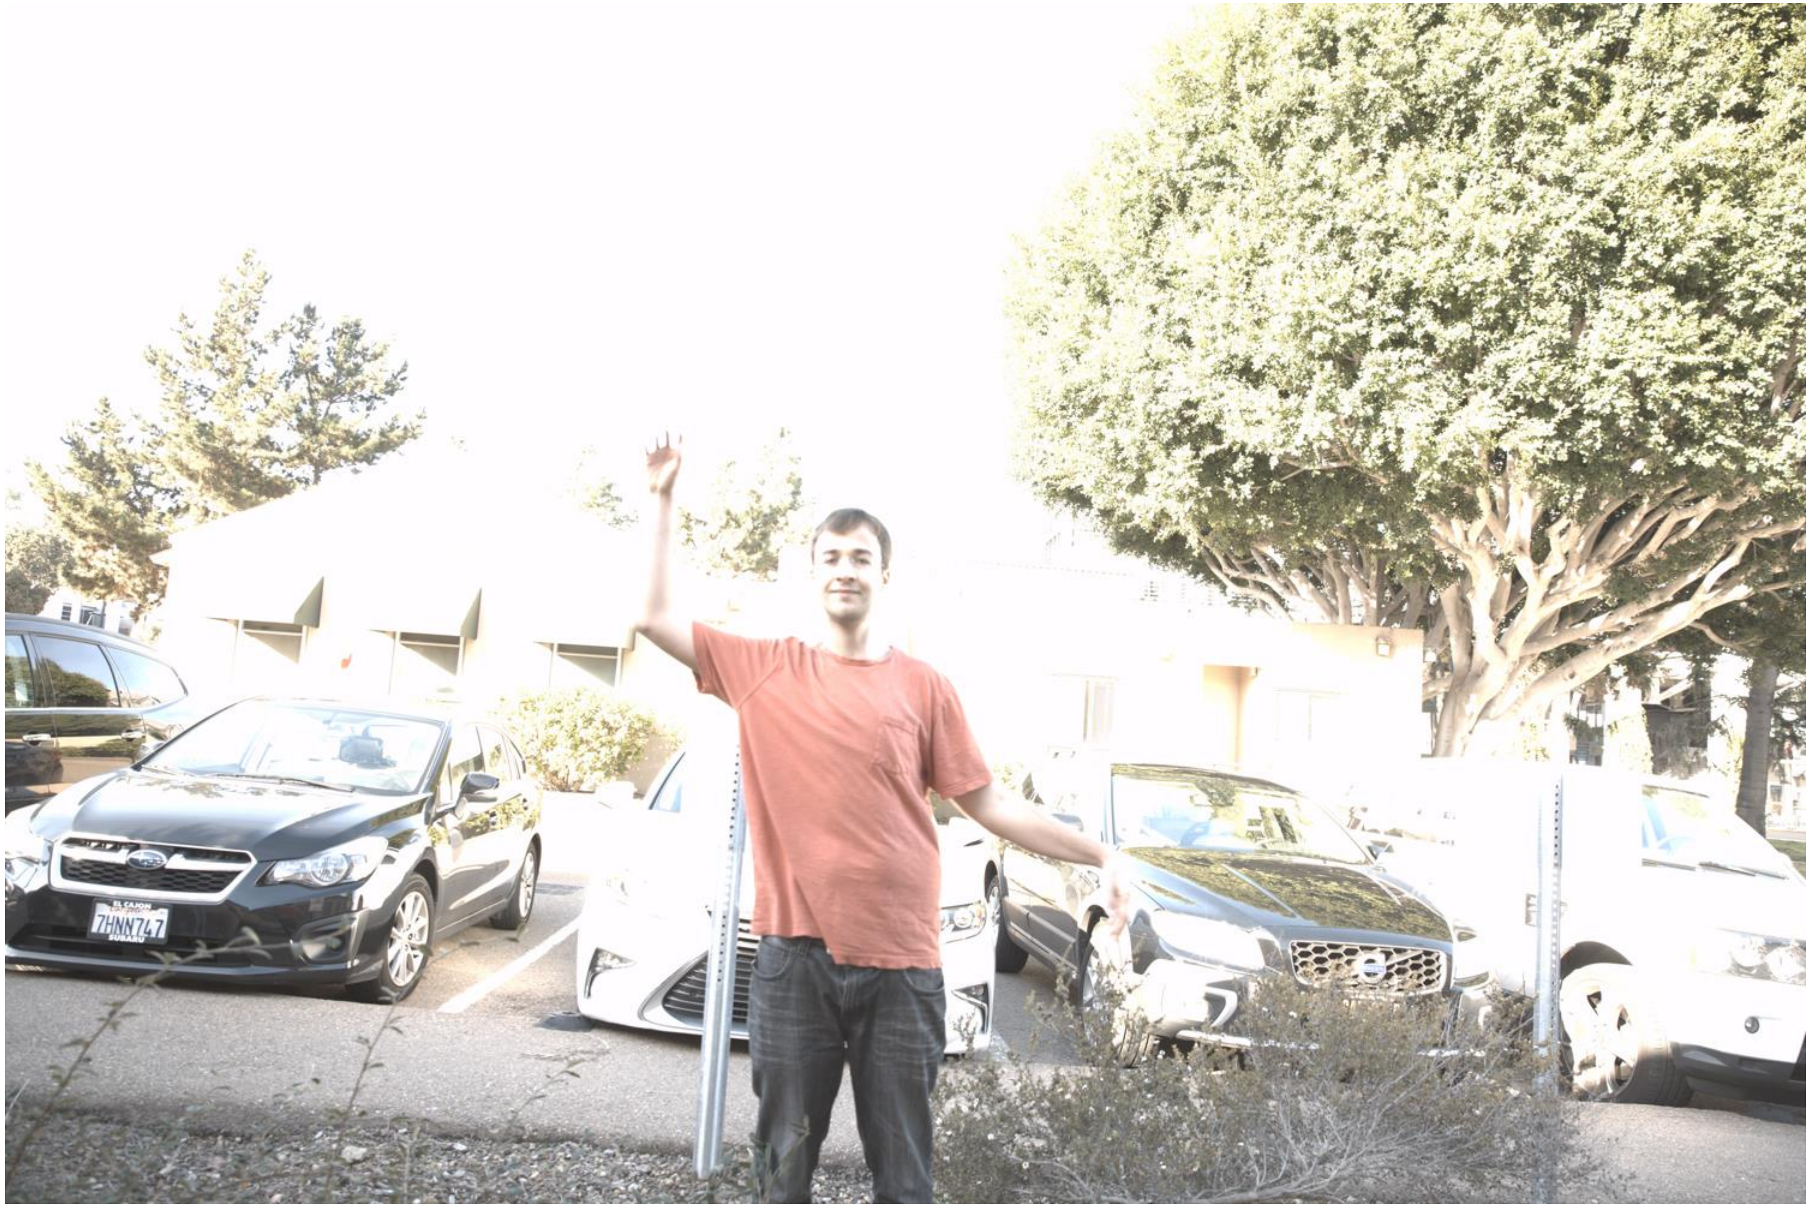

# HDR result
Sen et al. [2012]

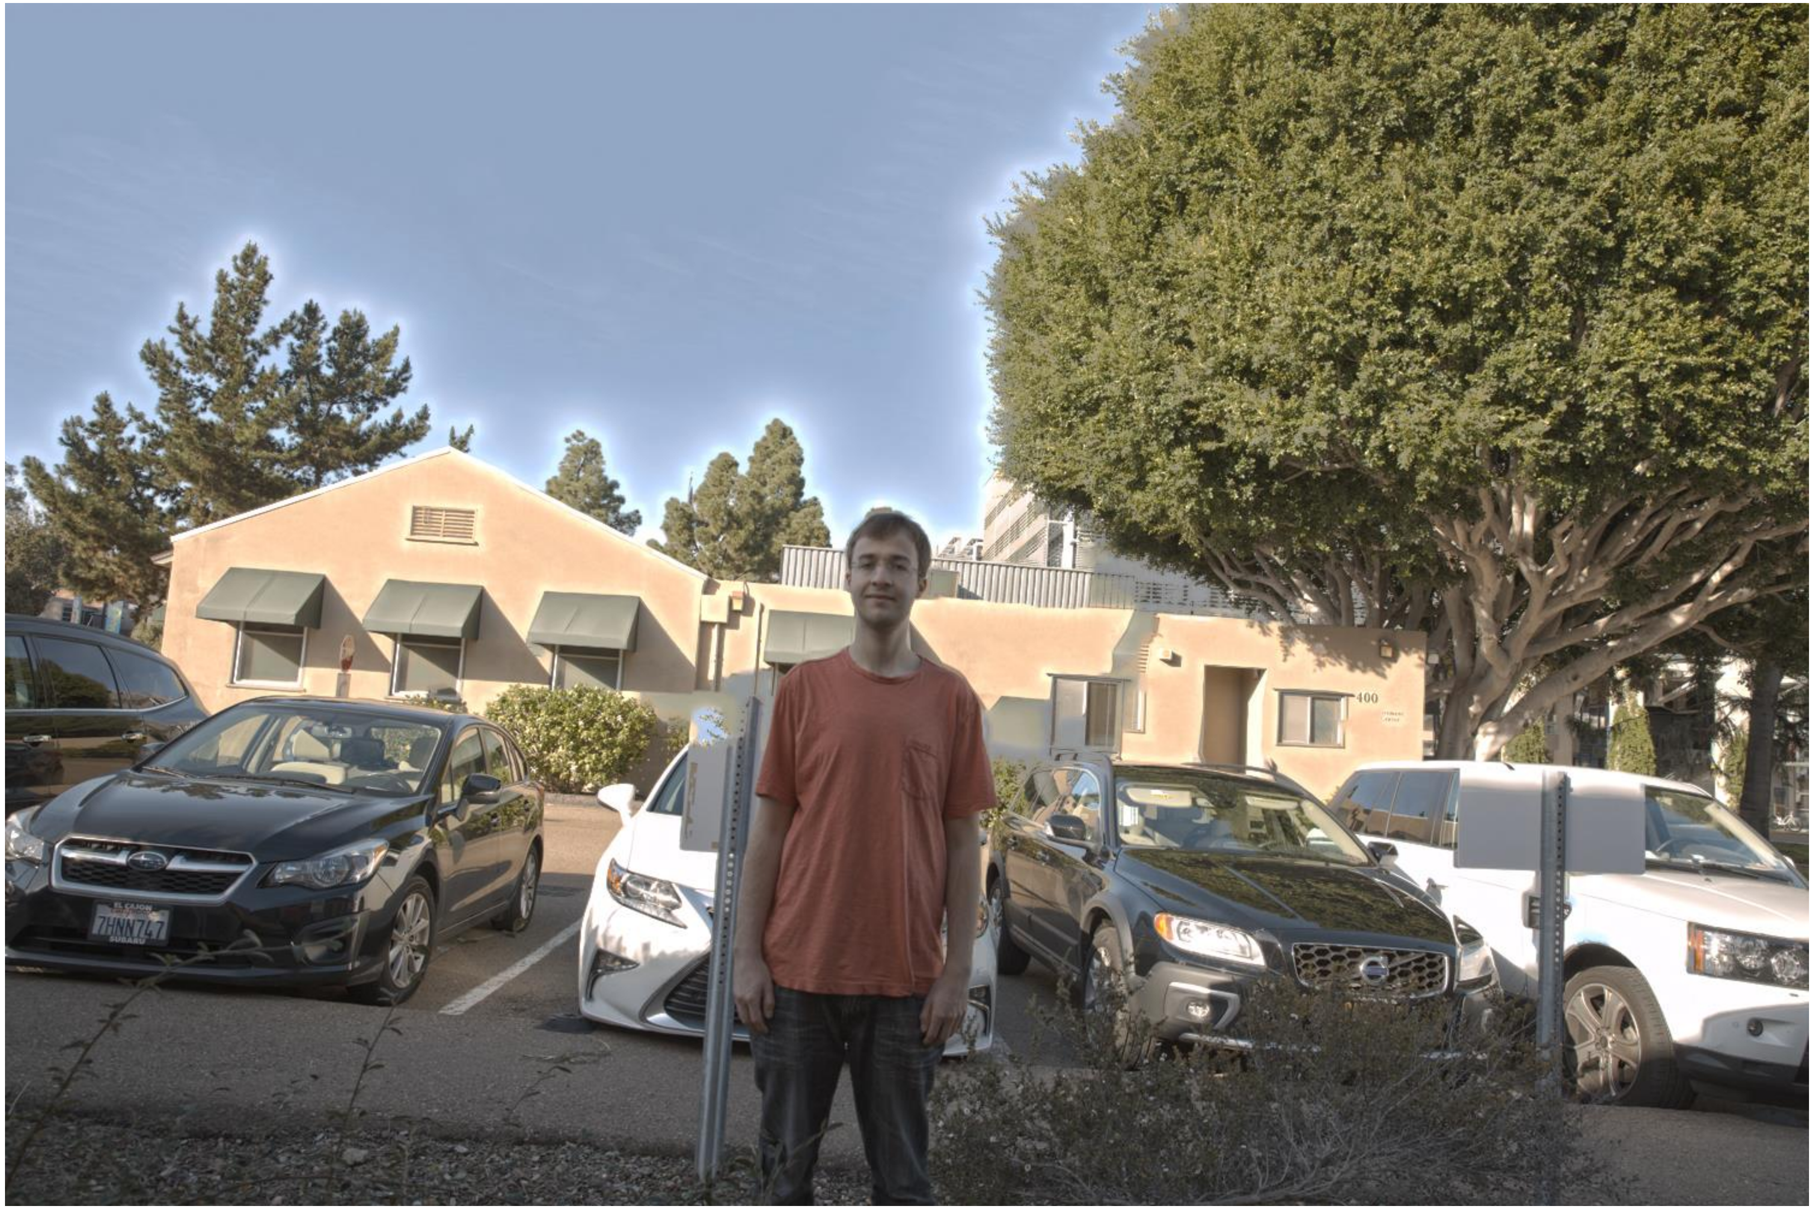

# HDR result
Kalantari et al. [2017]

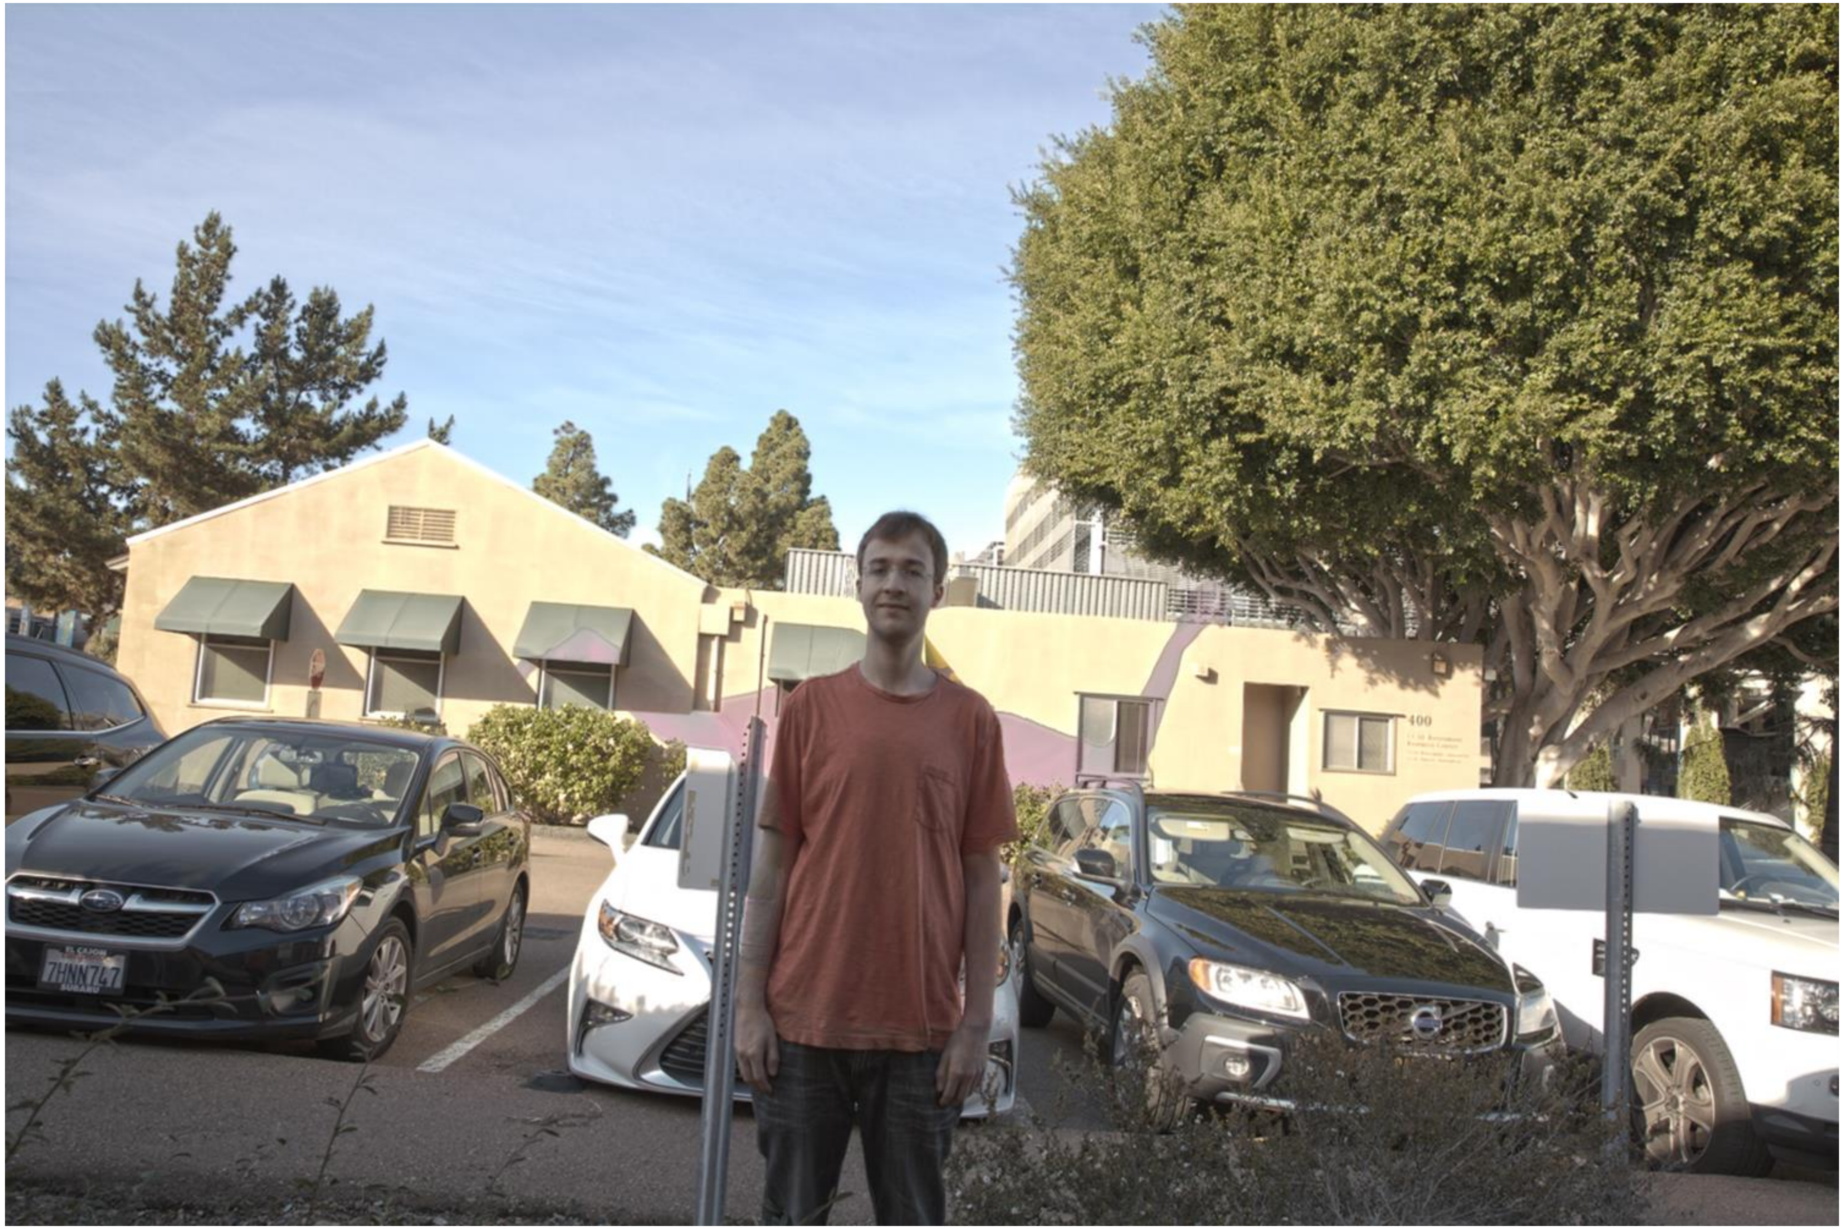

# HDR result
Wu et al. [2018]

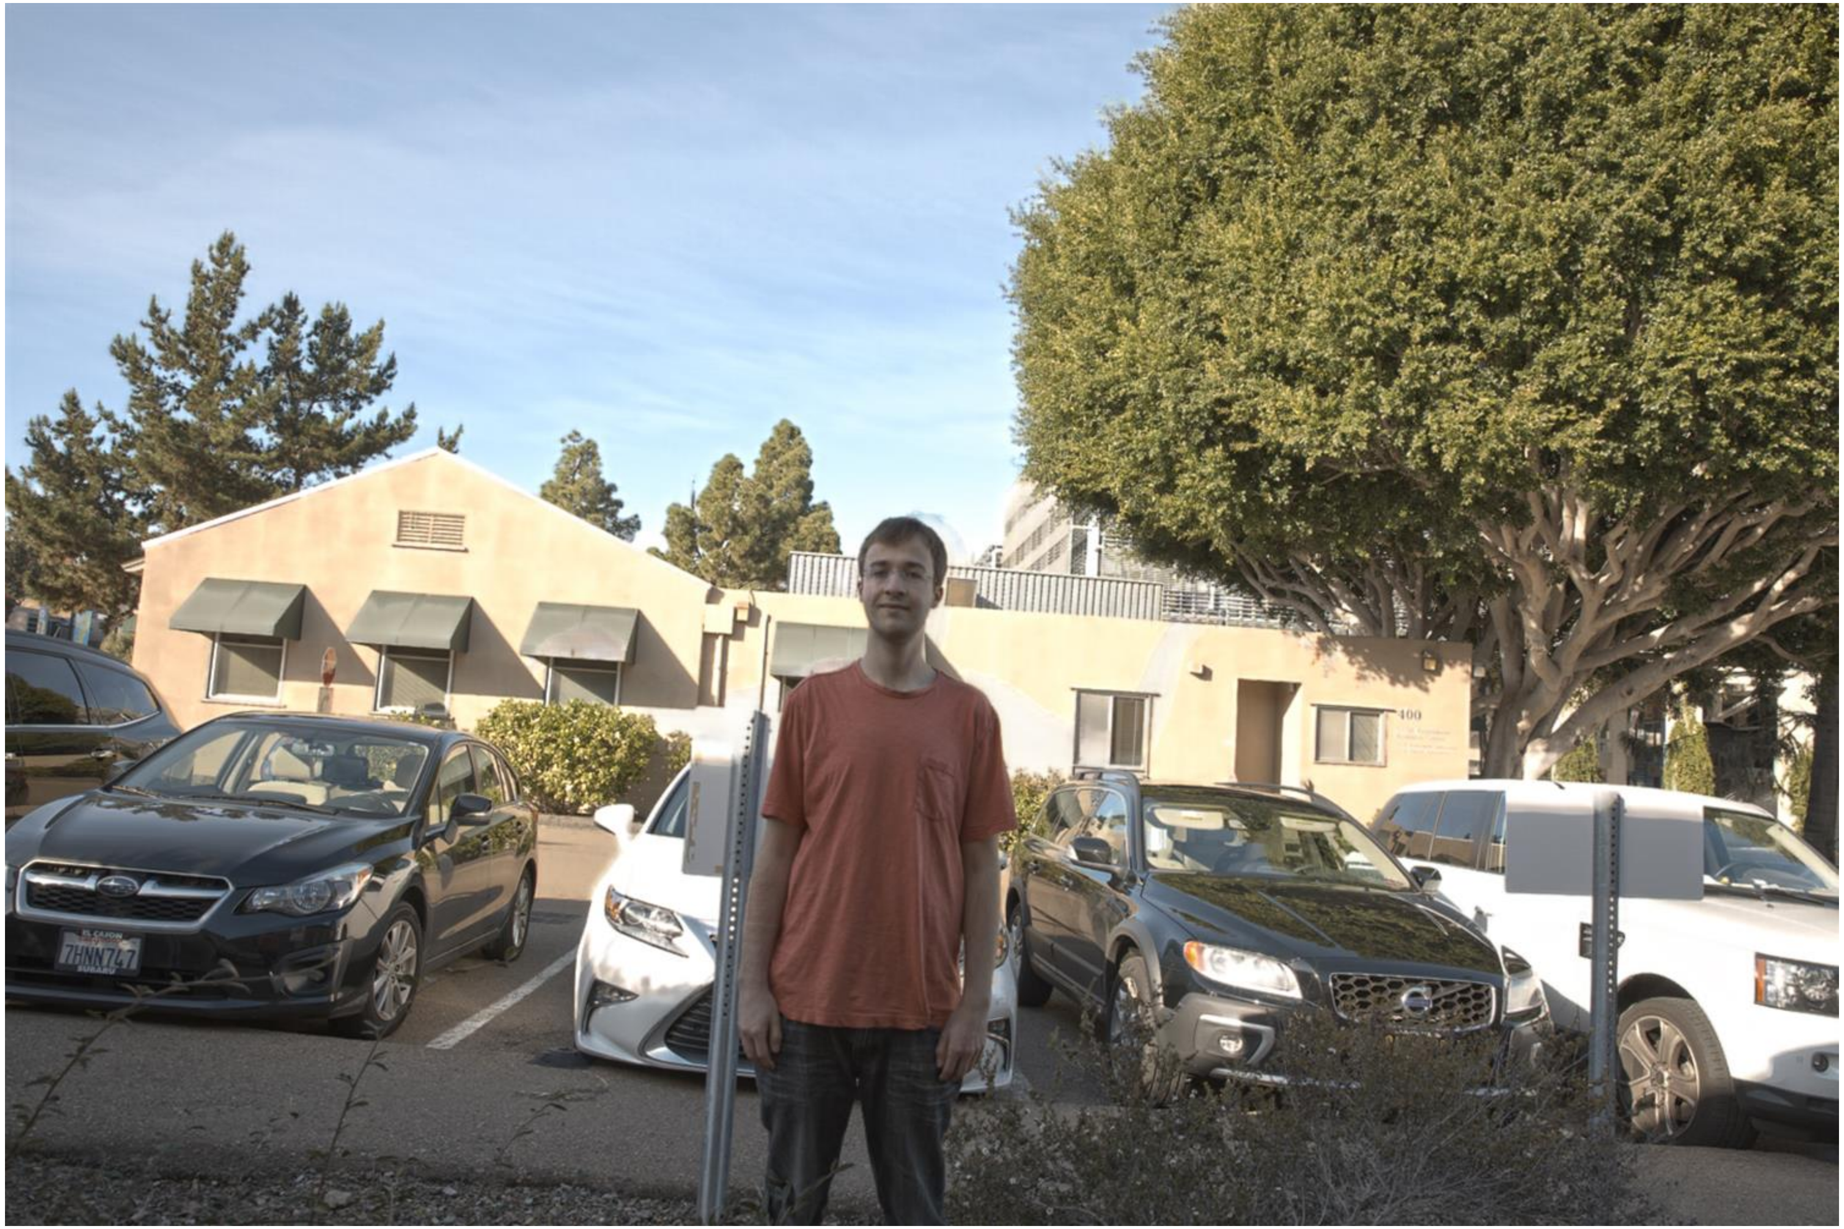

# HDR result
Yan et al. [2019]

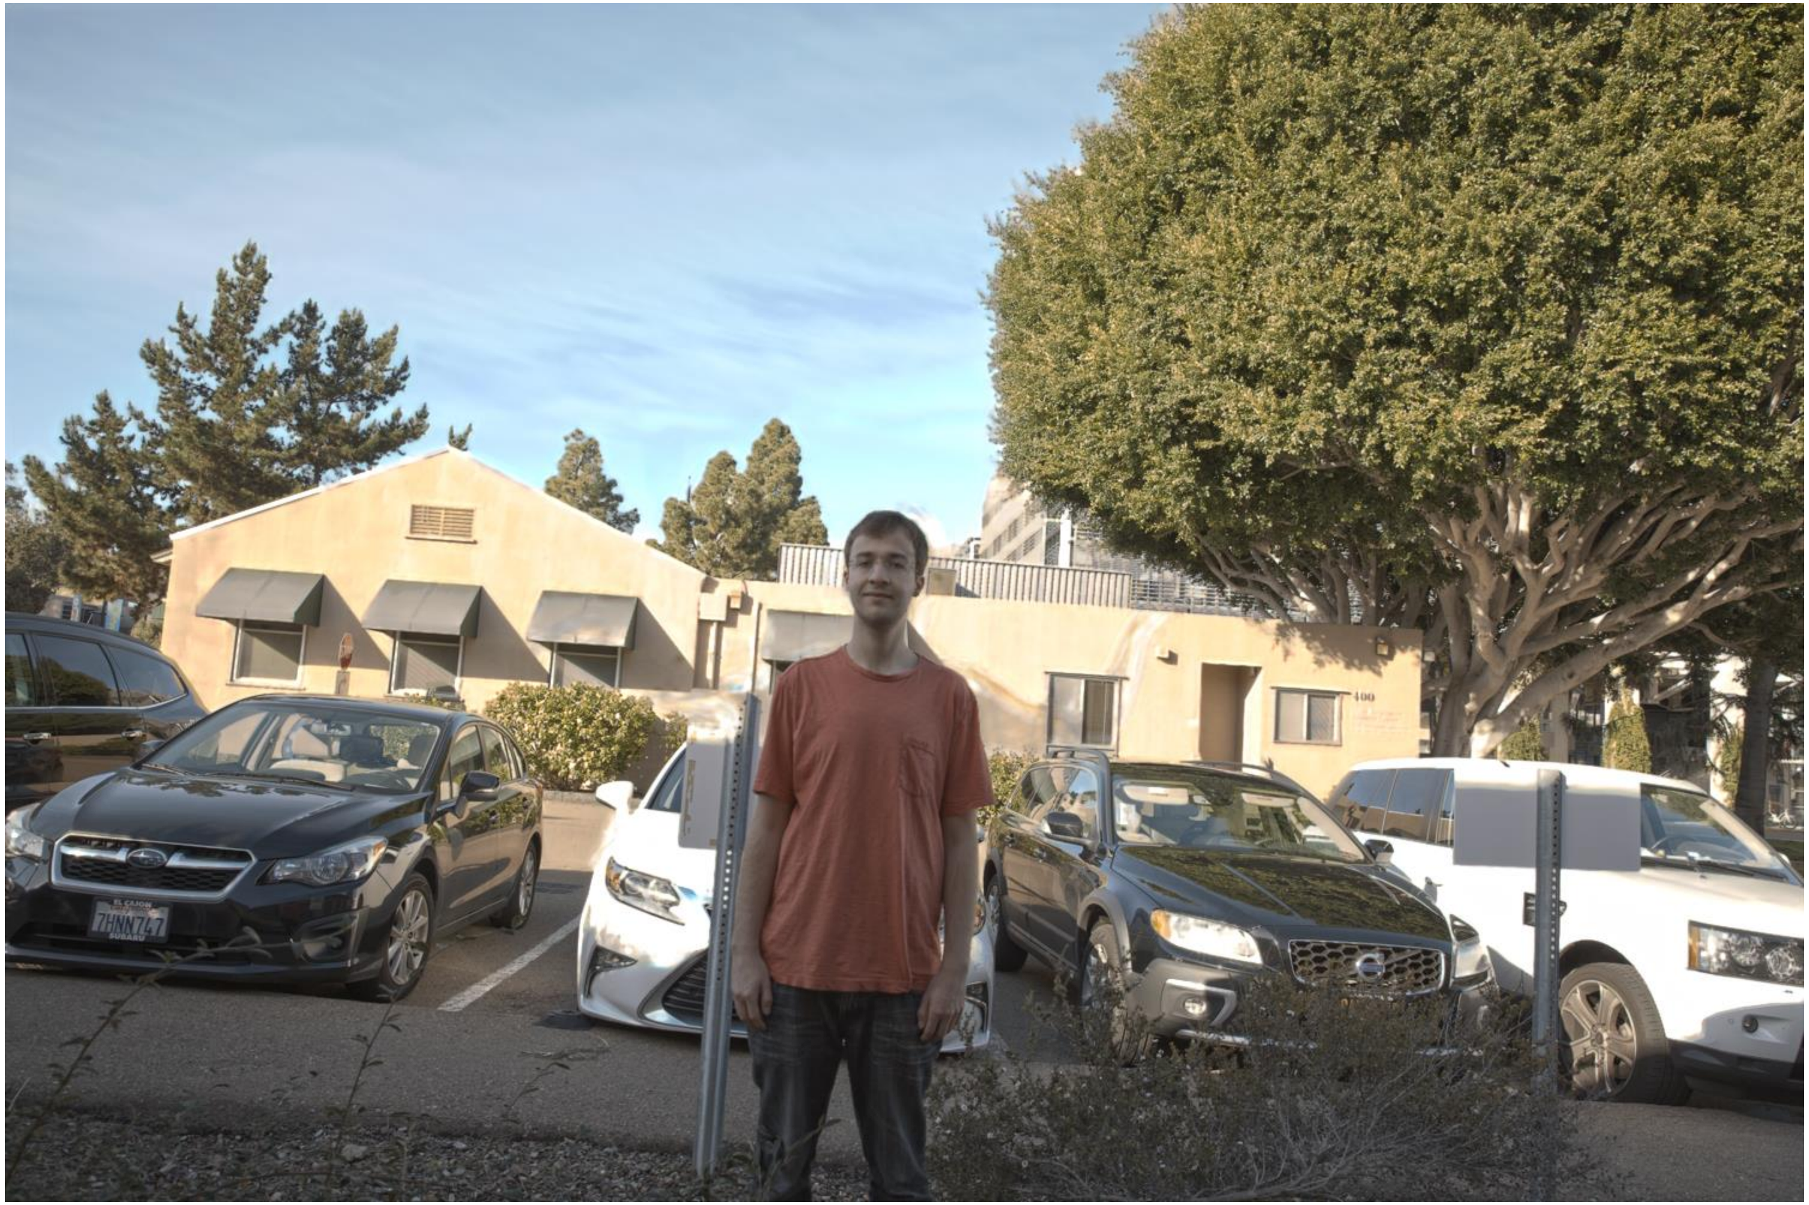

# HDR result
Li et al. [2020]

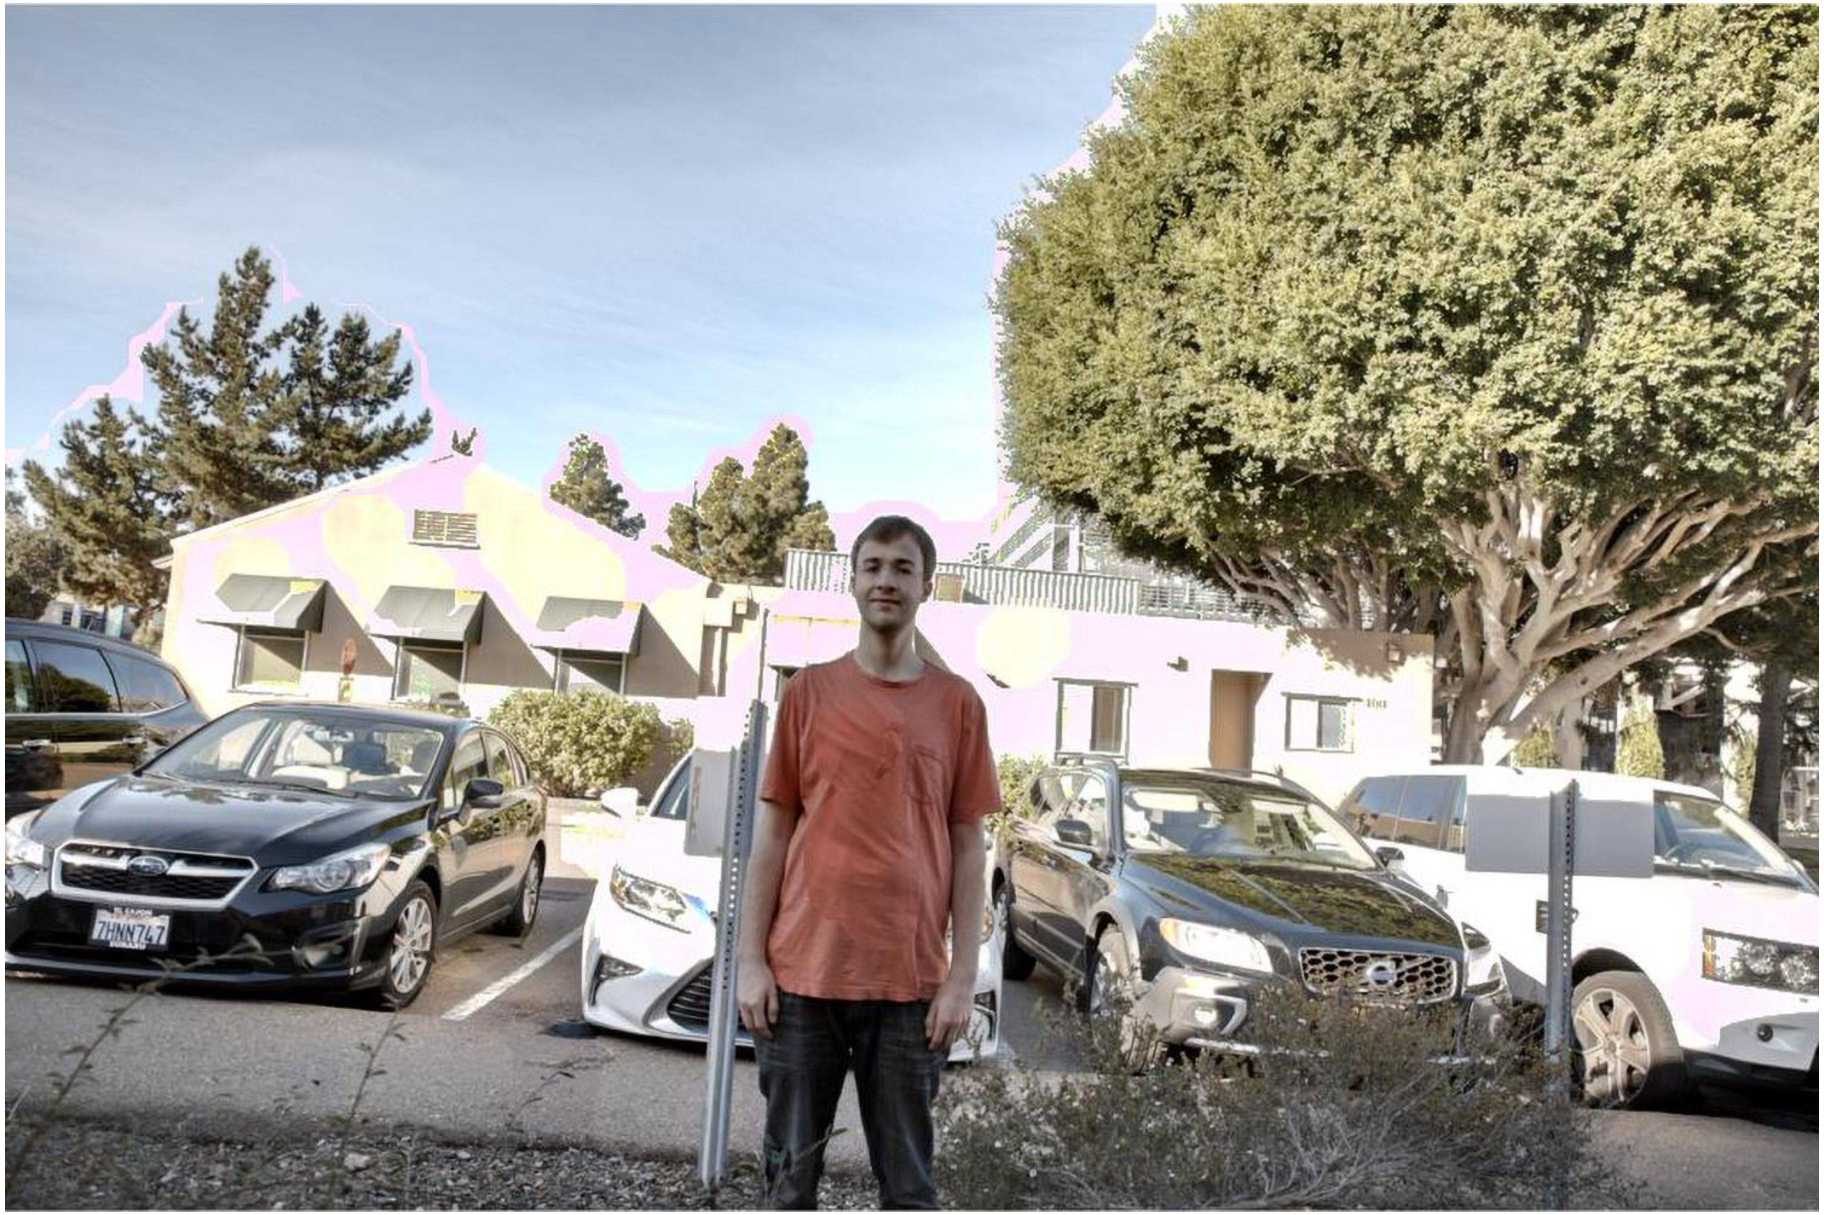

# HDR result
Niu et al. [2021]

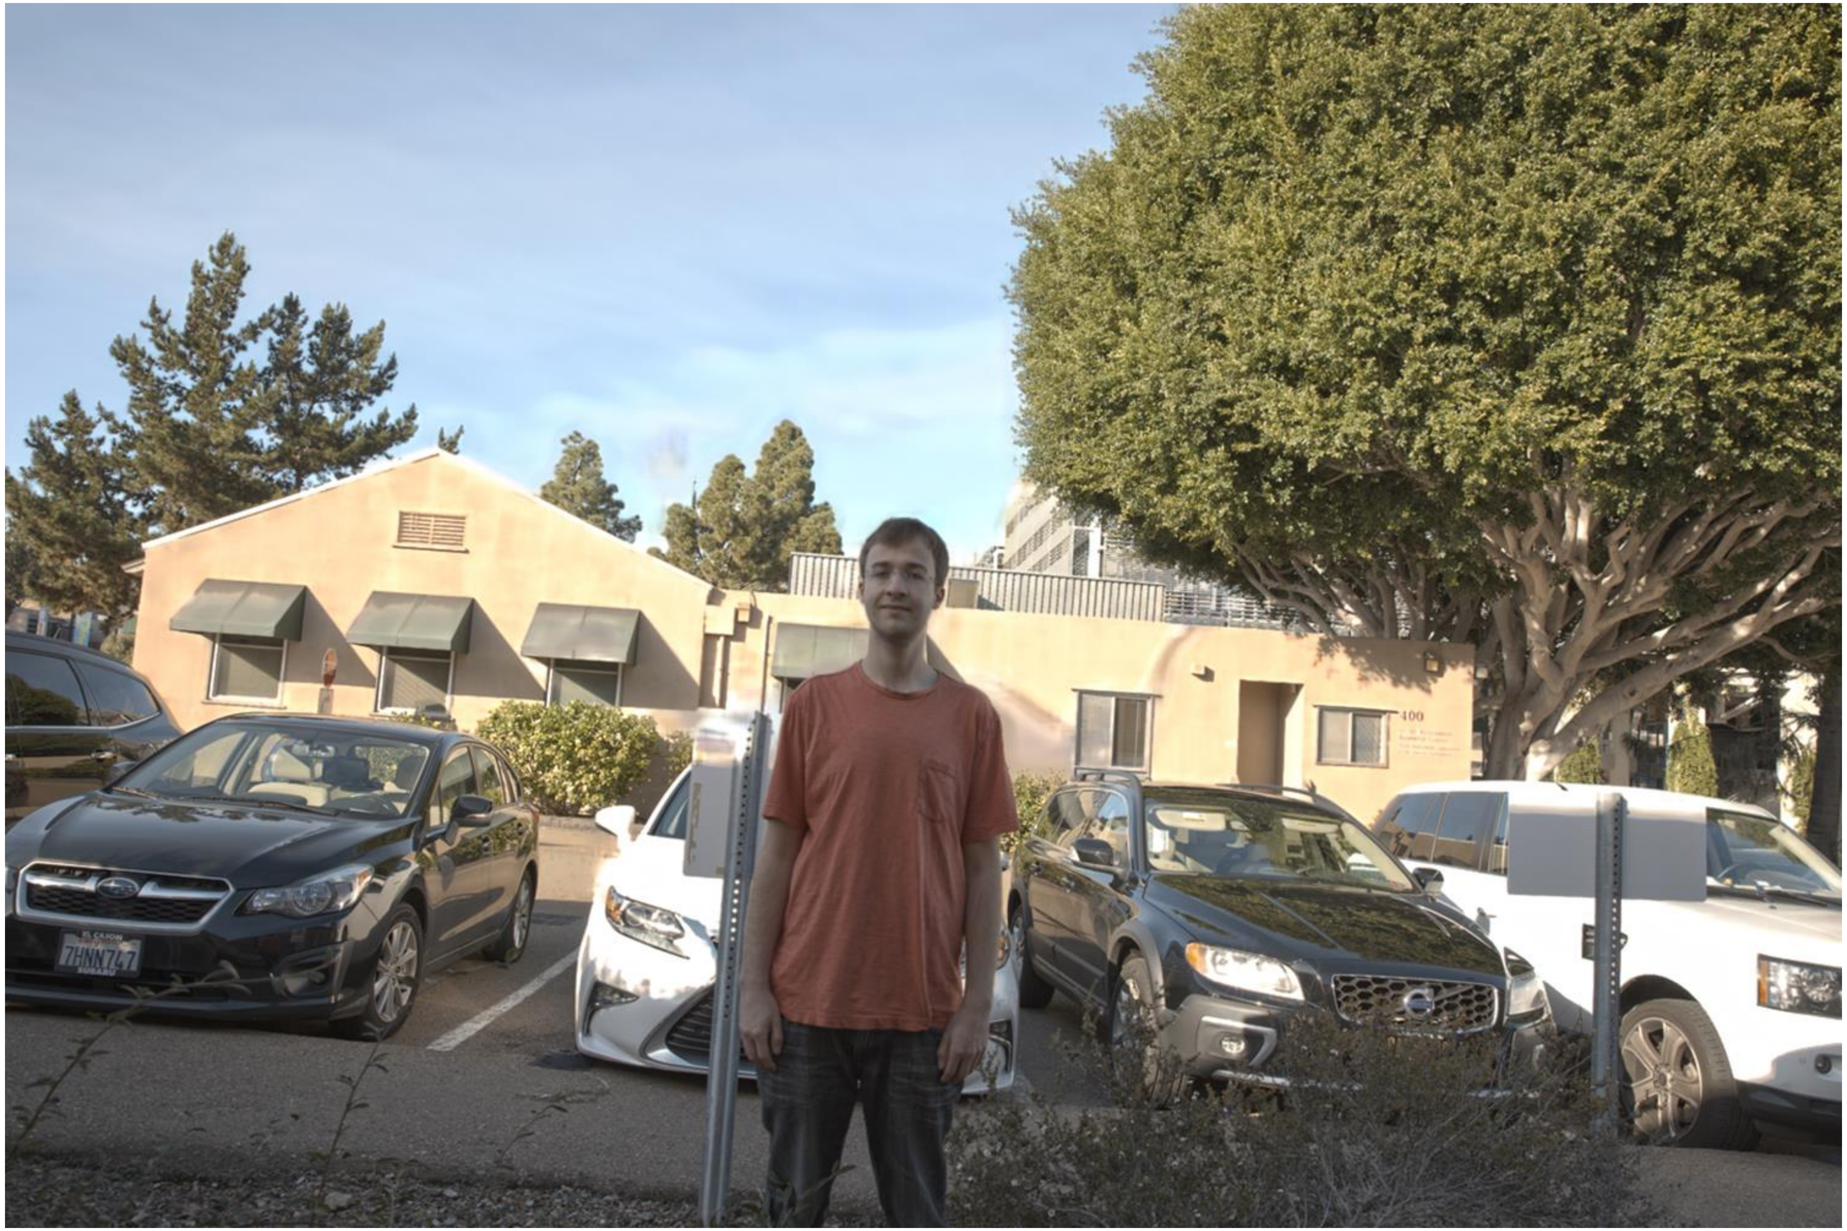

# HDR result
## Ours

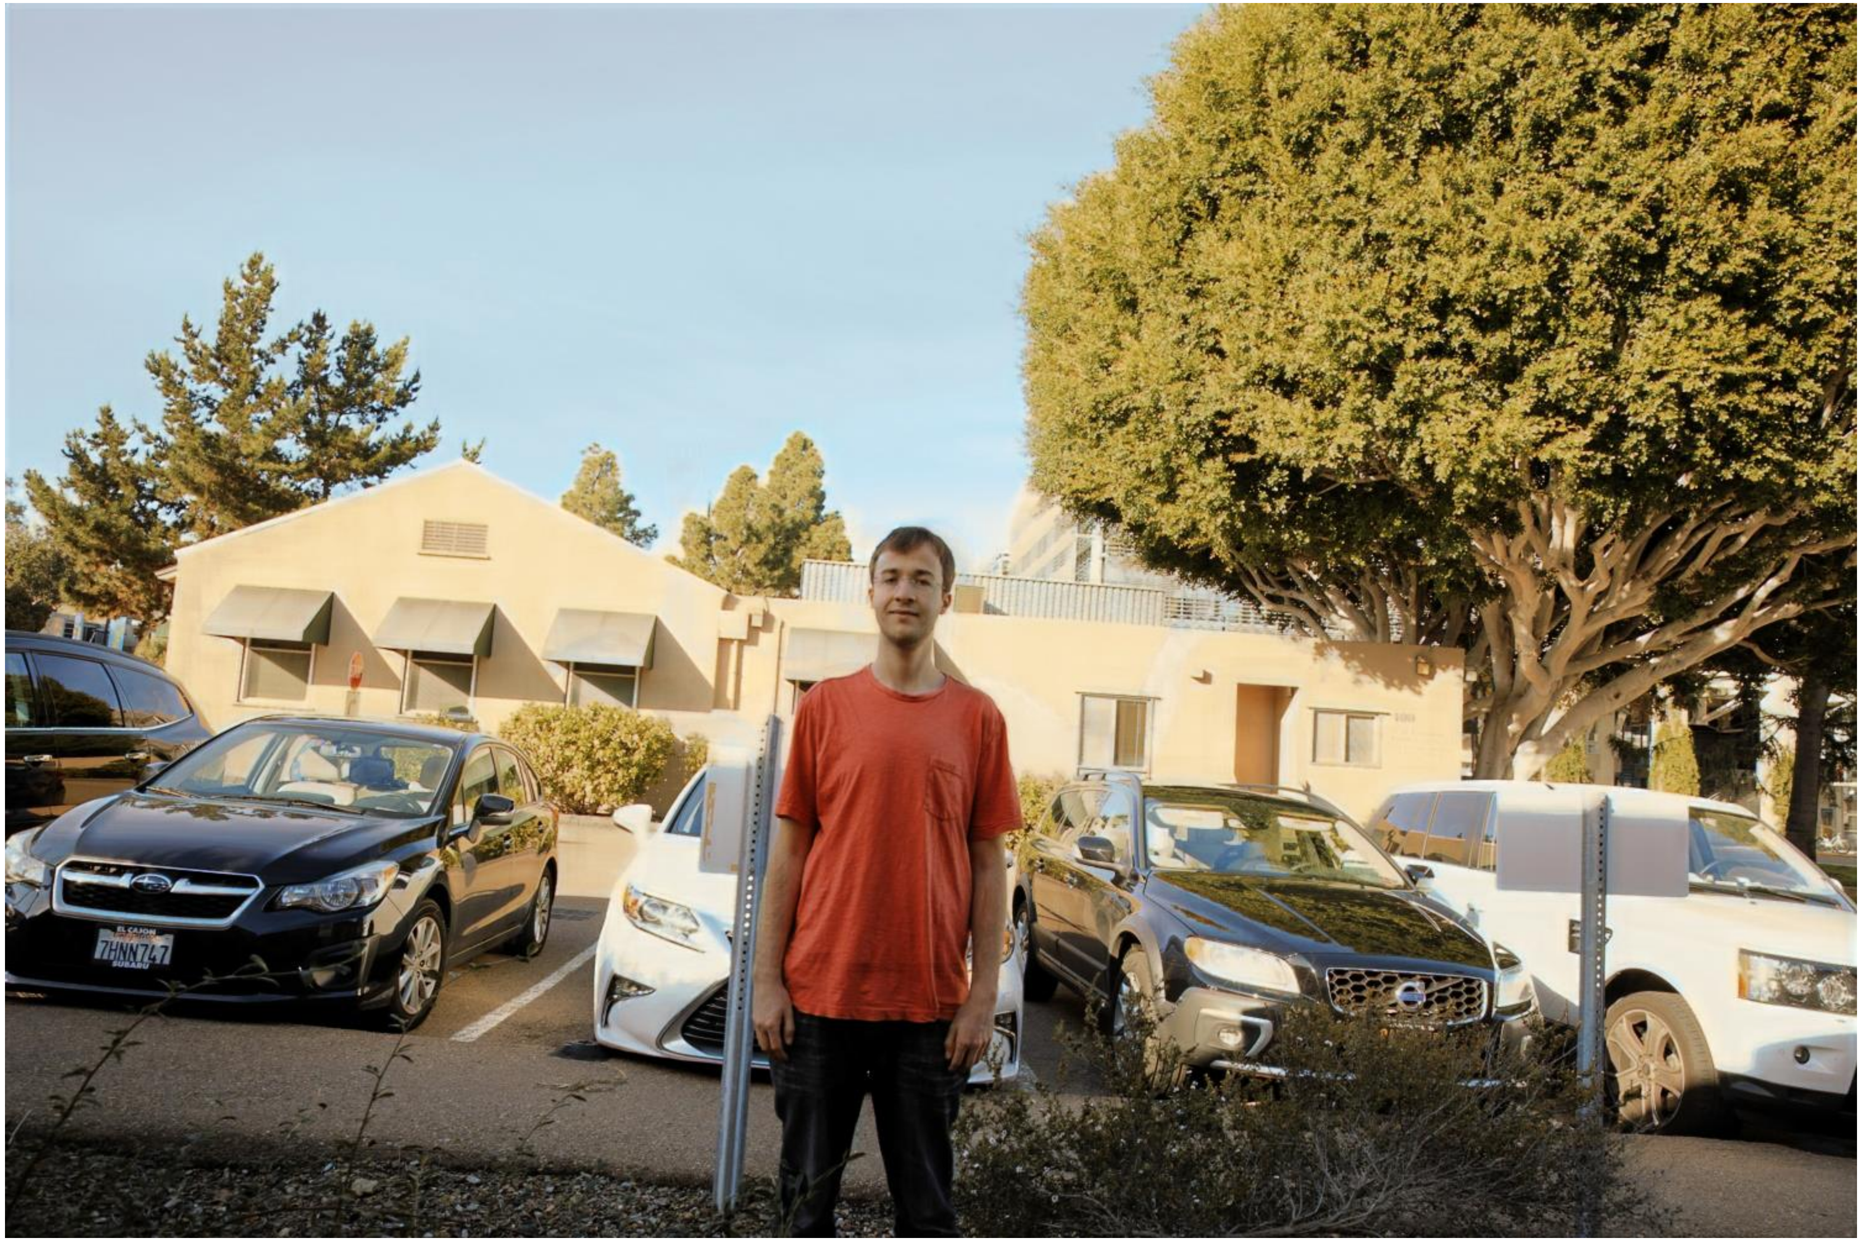

# 3. Comparison Between Gradient and Structure Tensor

# Input LDR image 1
Exposure Value: -2.0

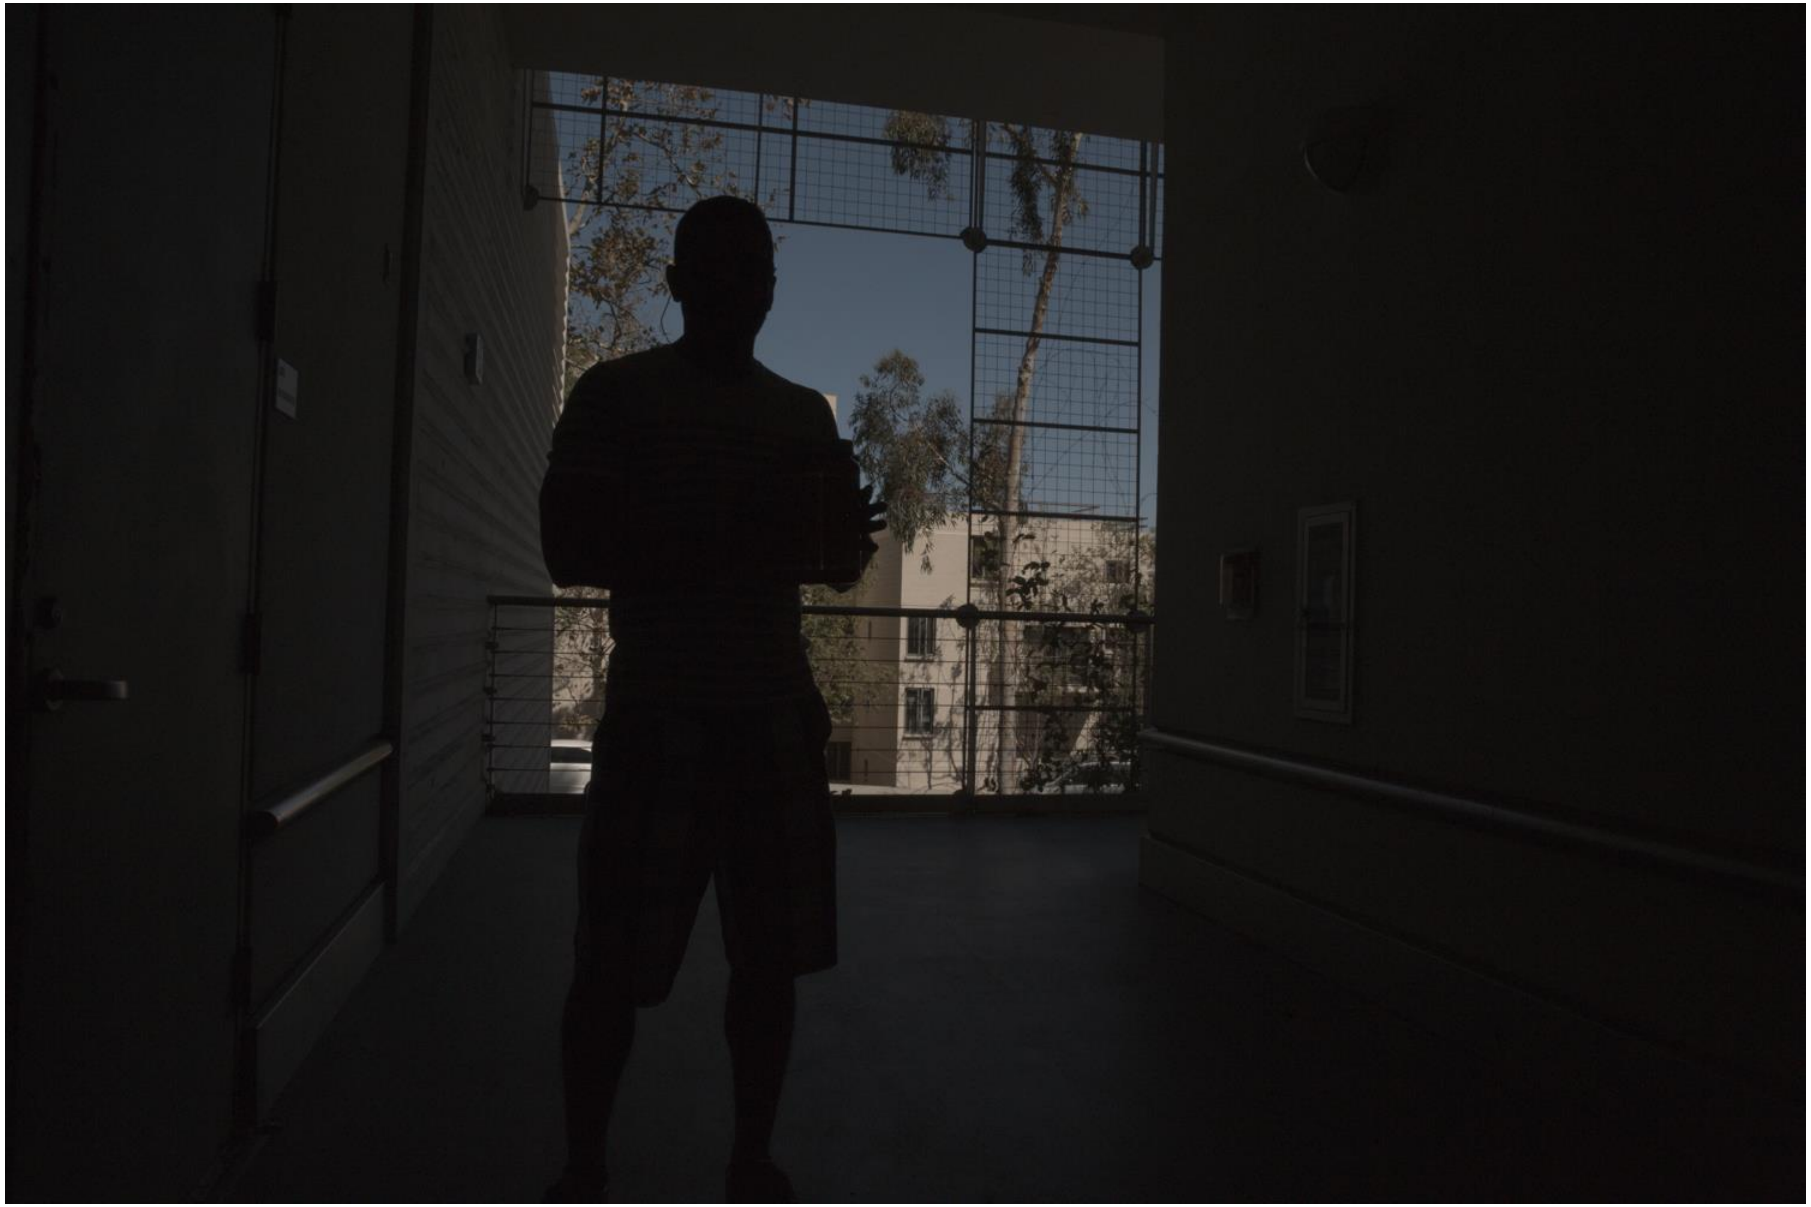

# Gradient map of Input LDR image 1

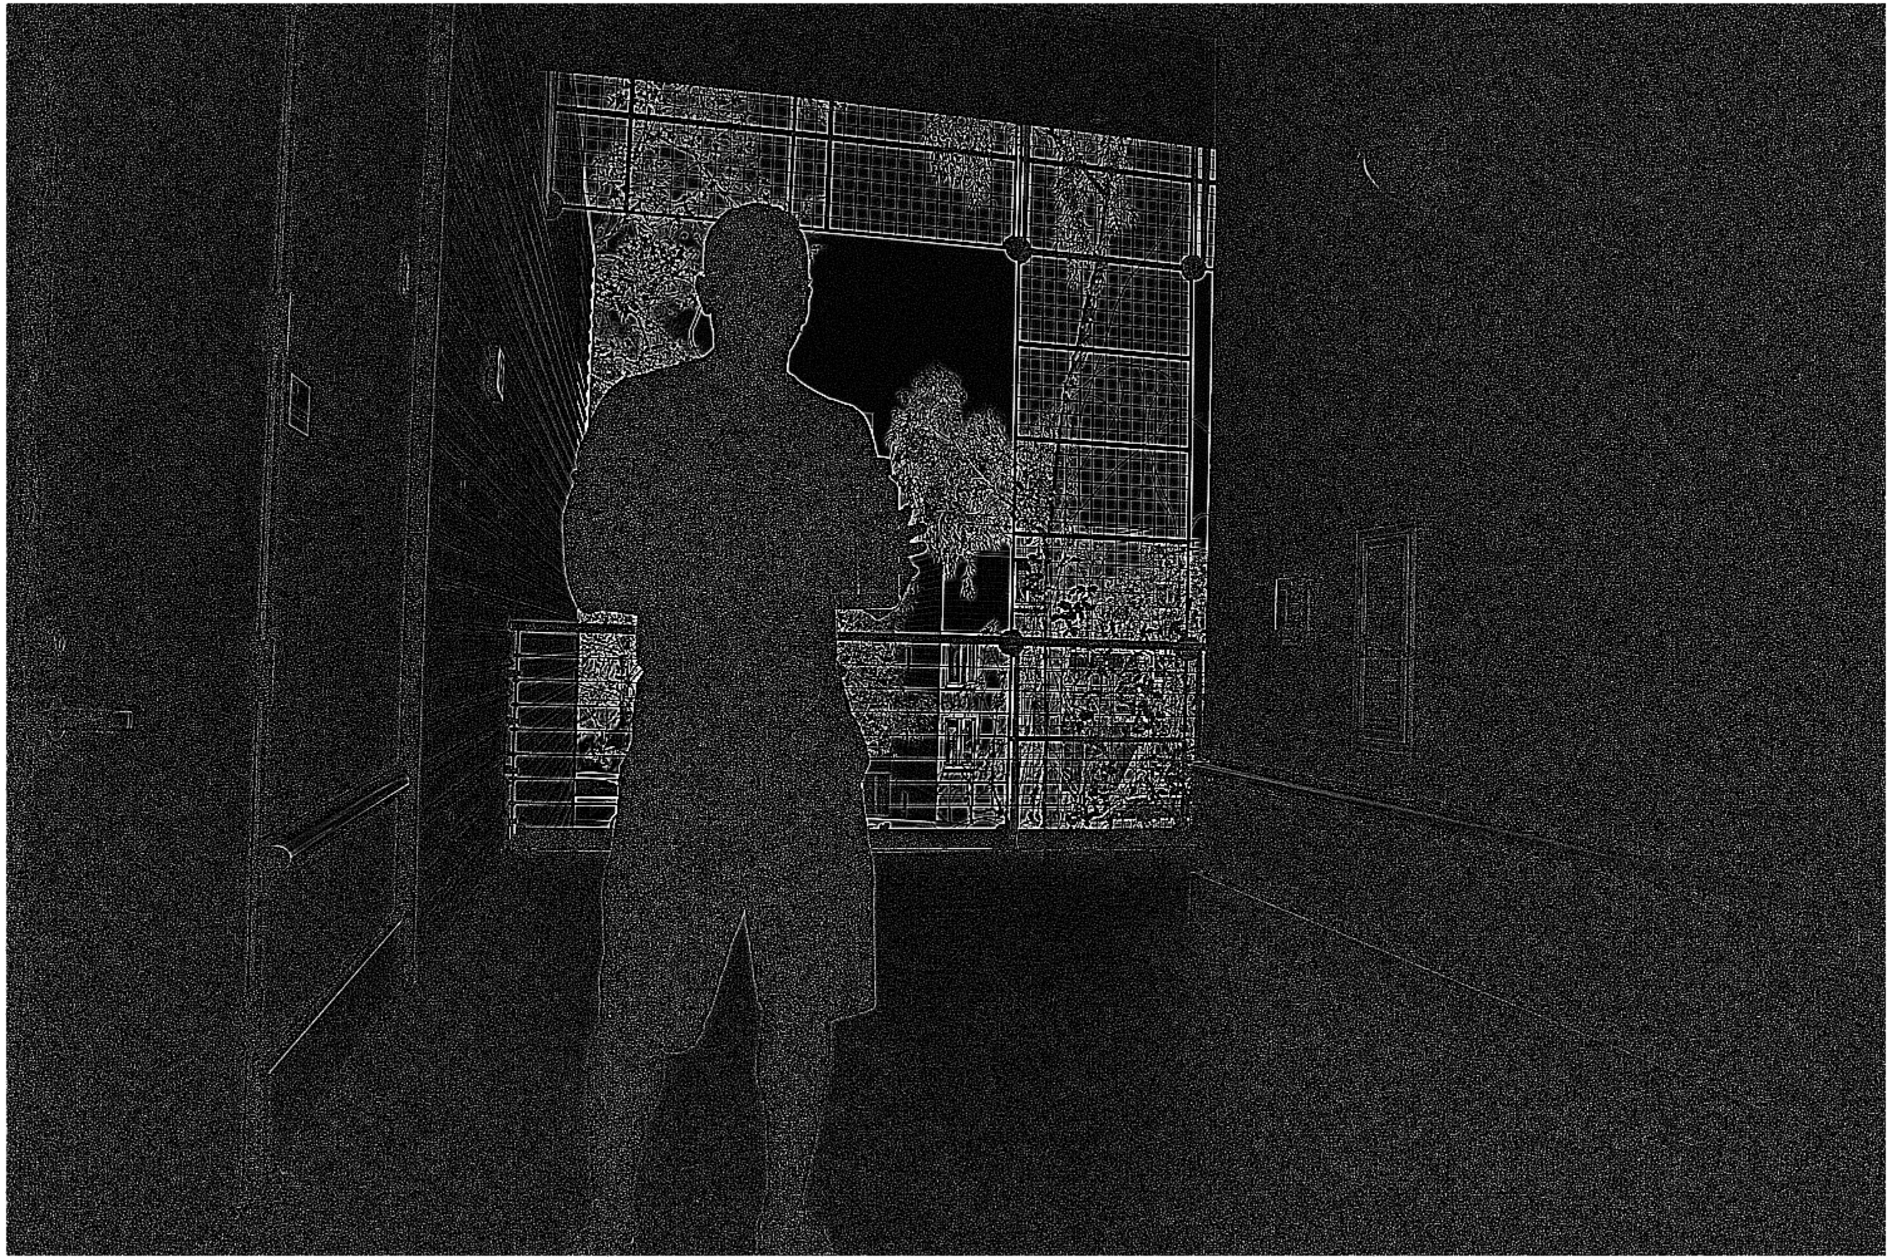

# Structure Tensor map of Input LDR image 1

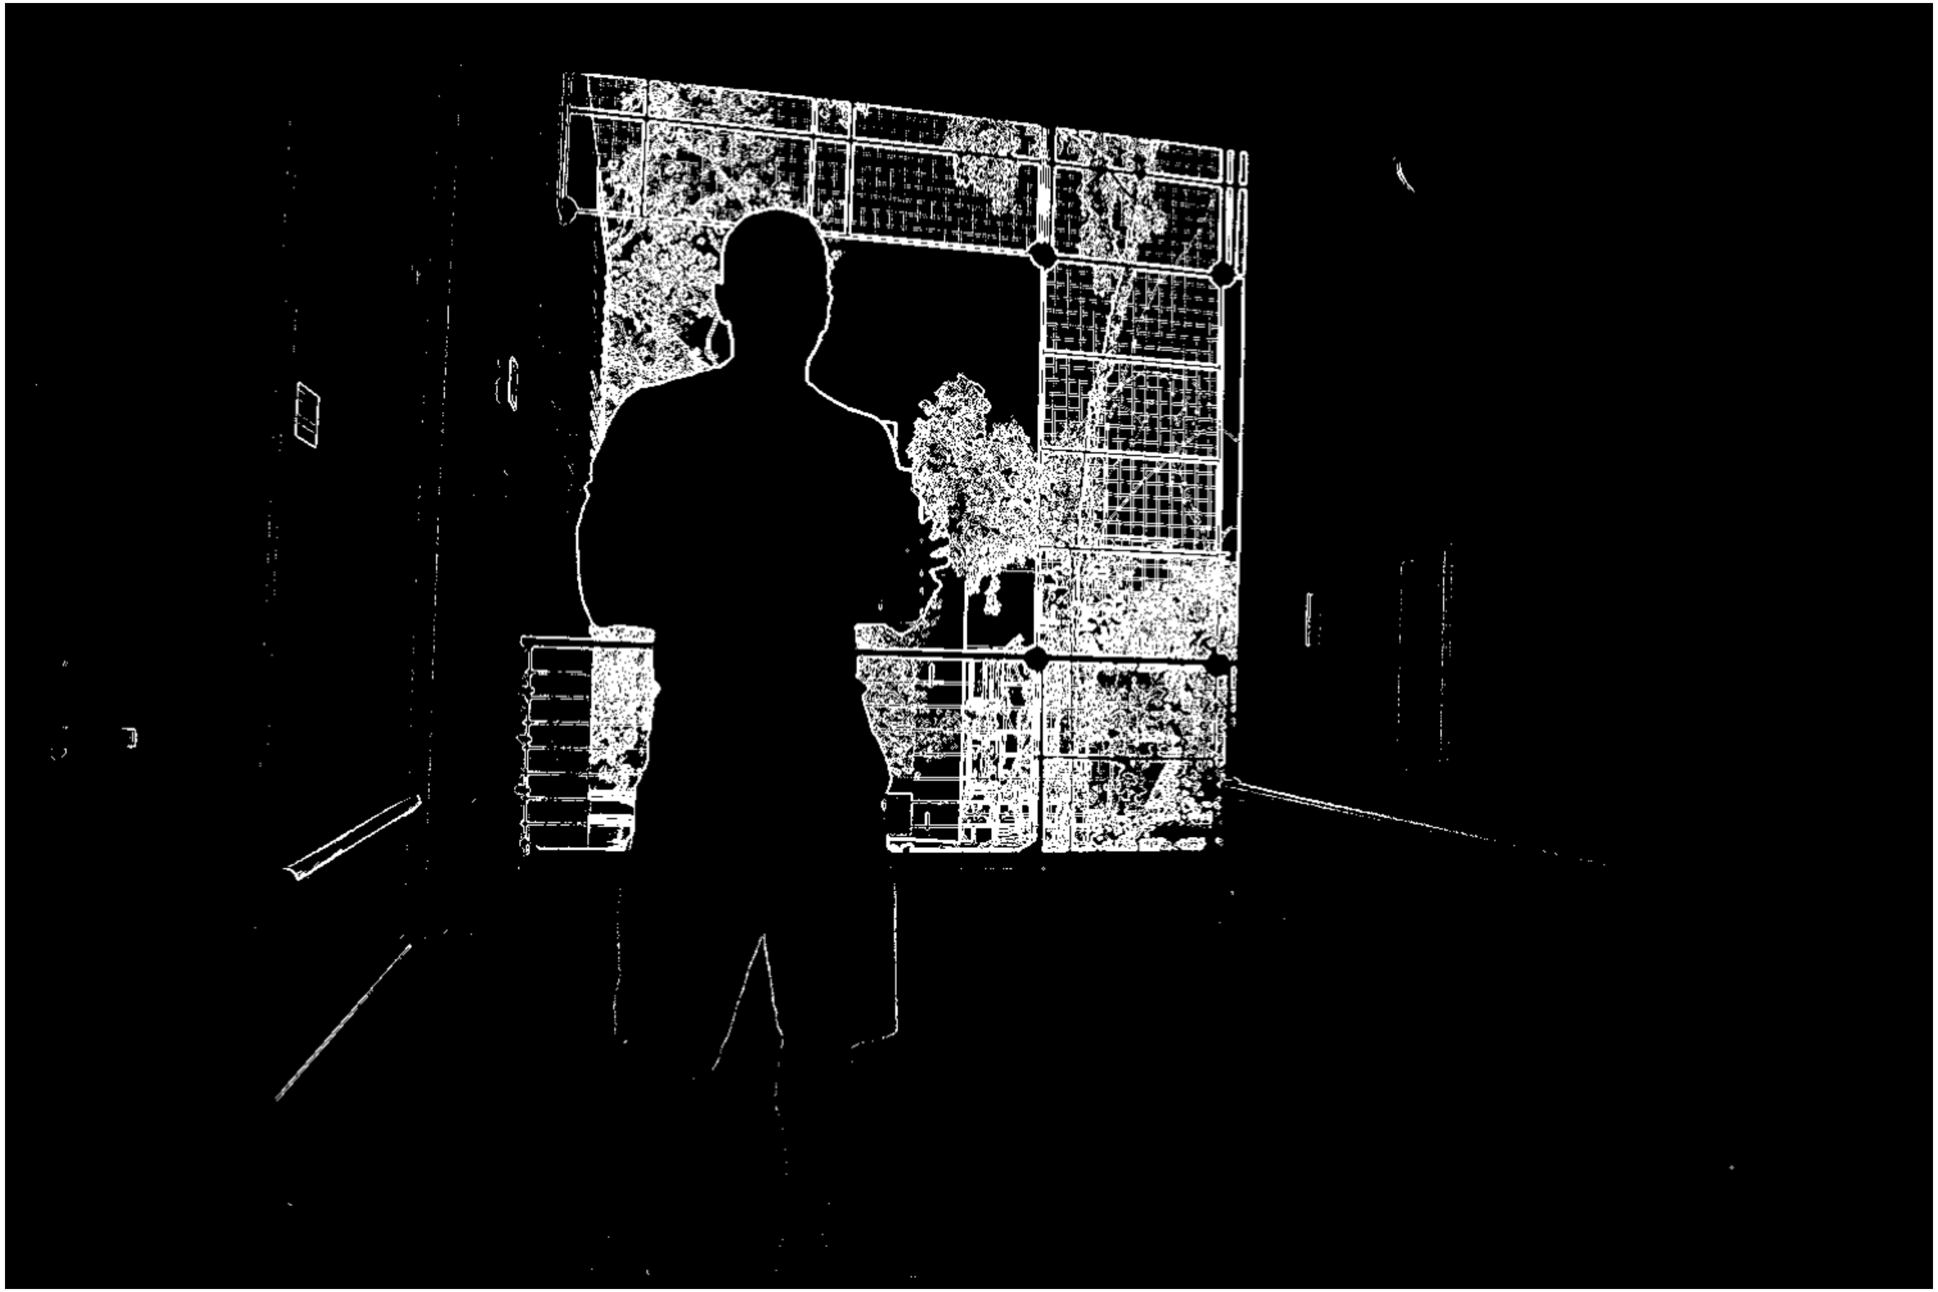

# Input LDR image 2

Exposure Value: 0.0

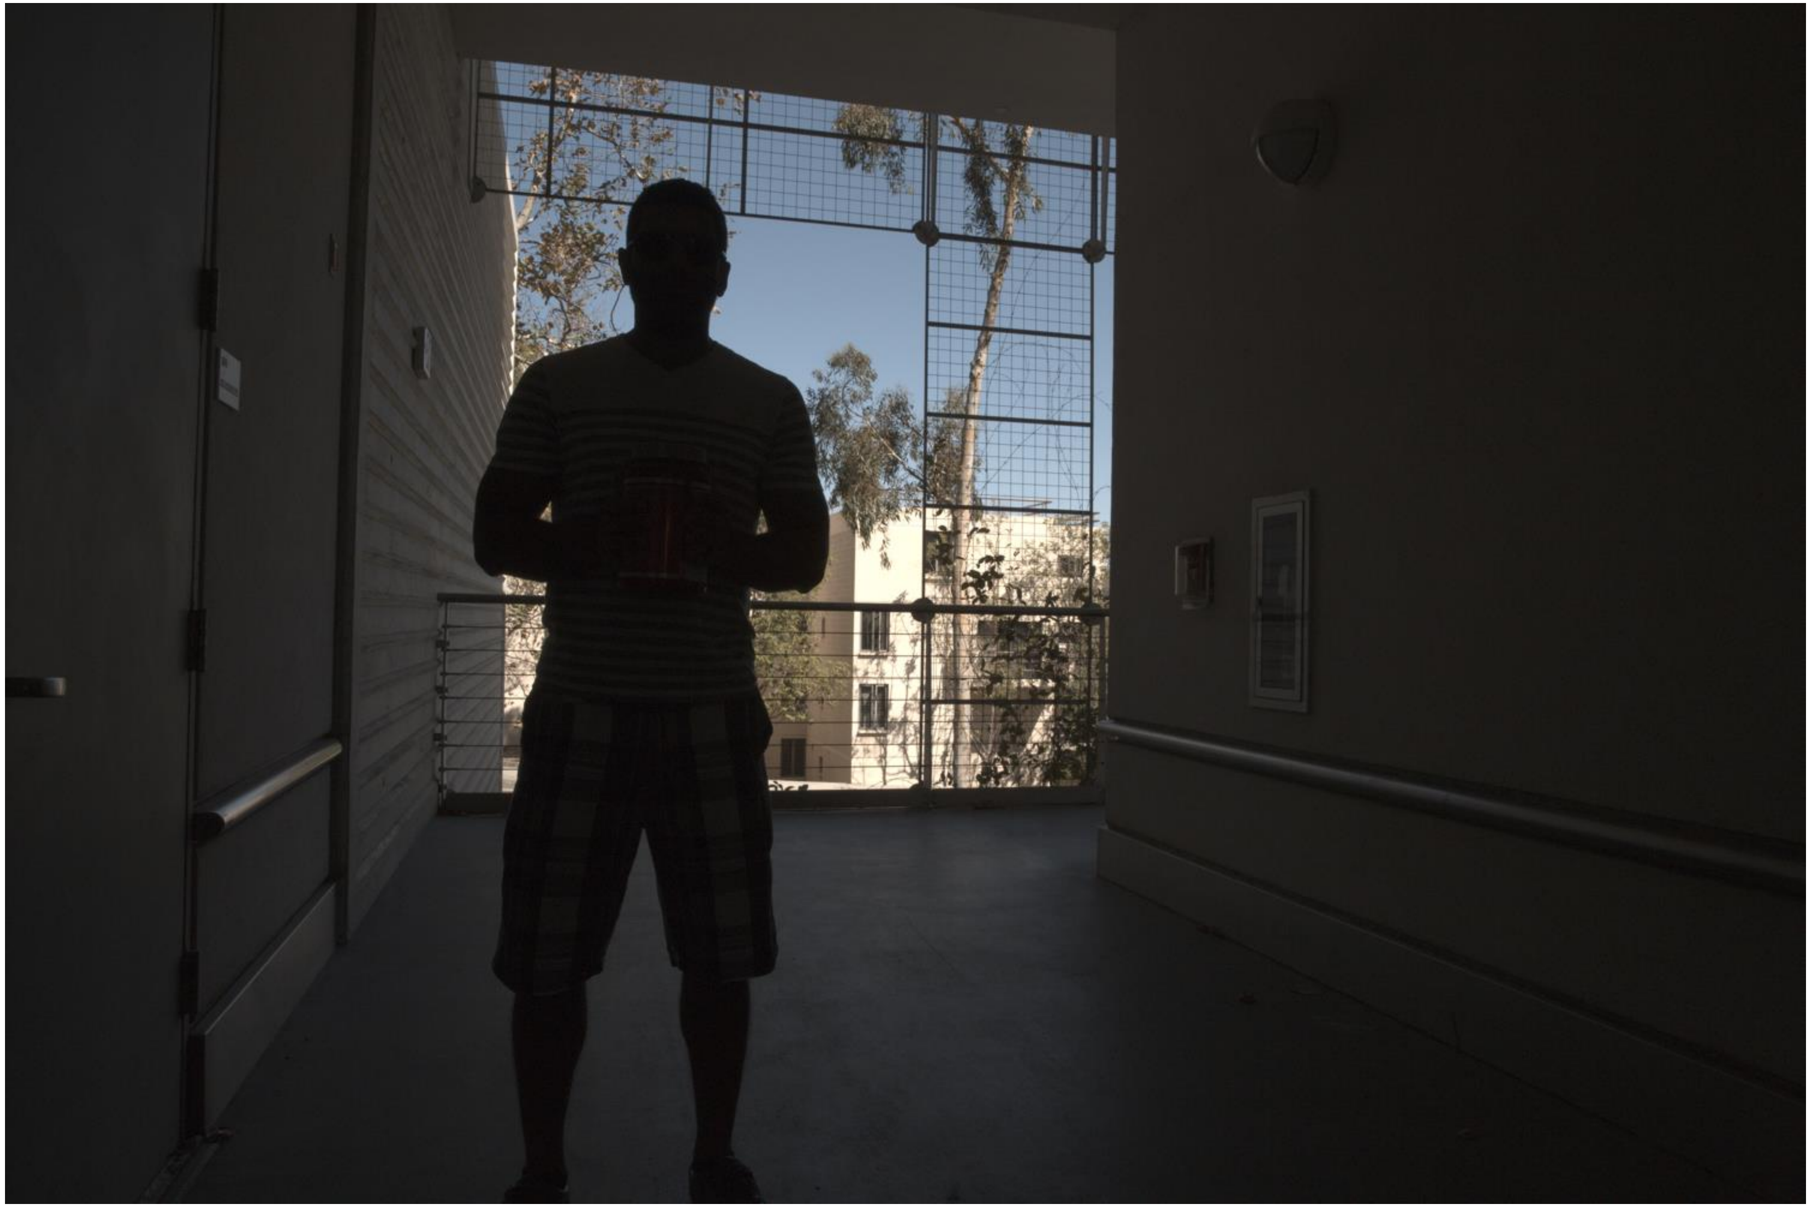

# Gradient map of Input LDR image 2

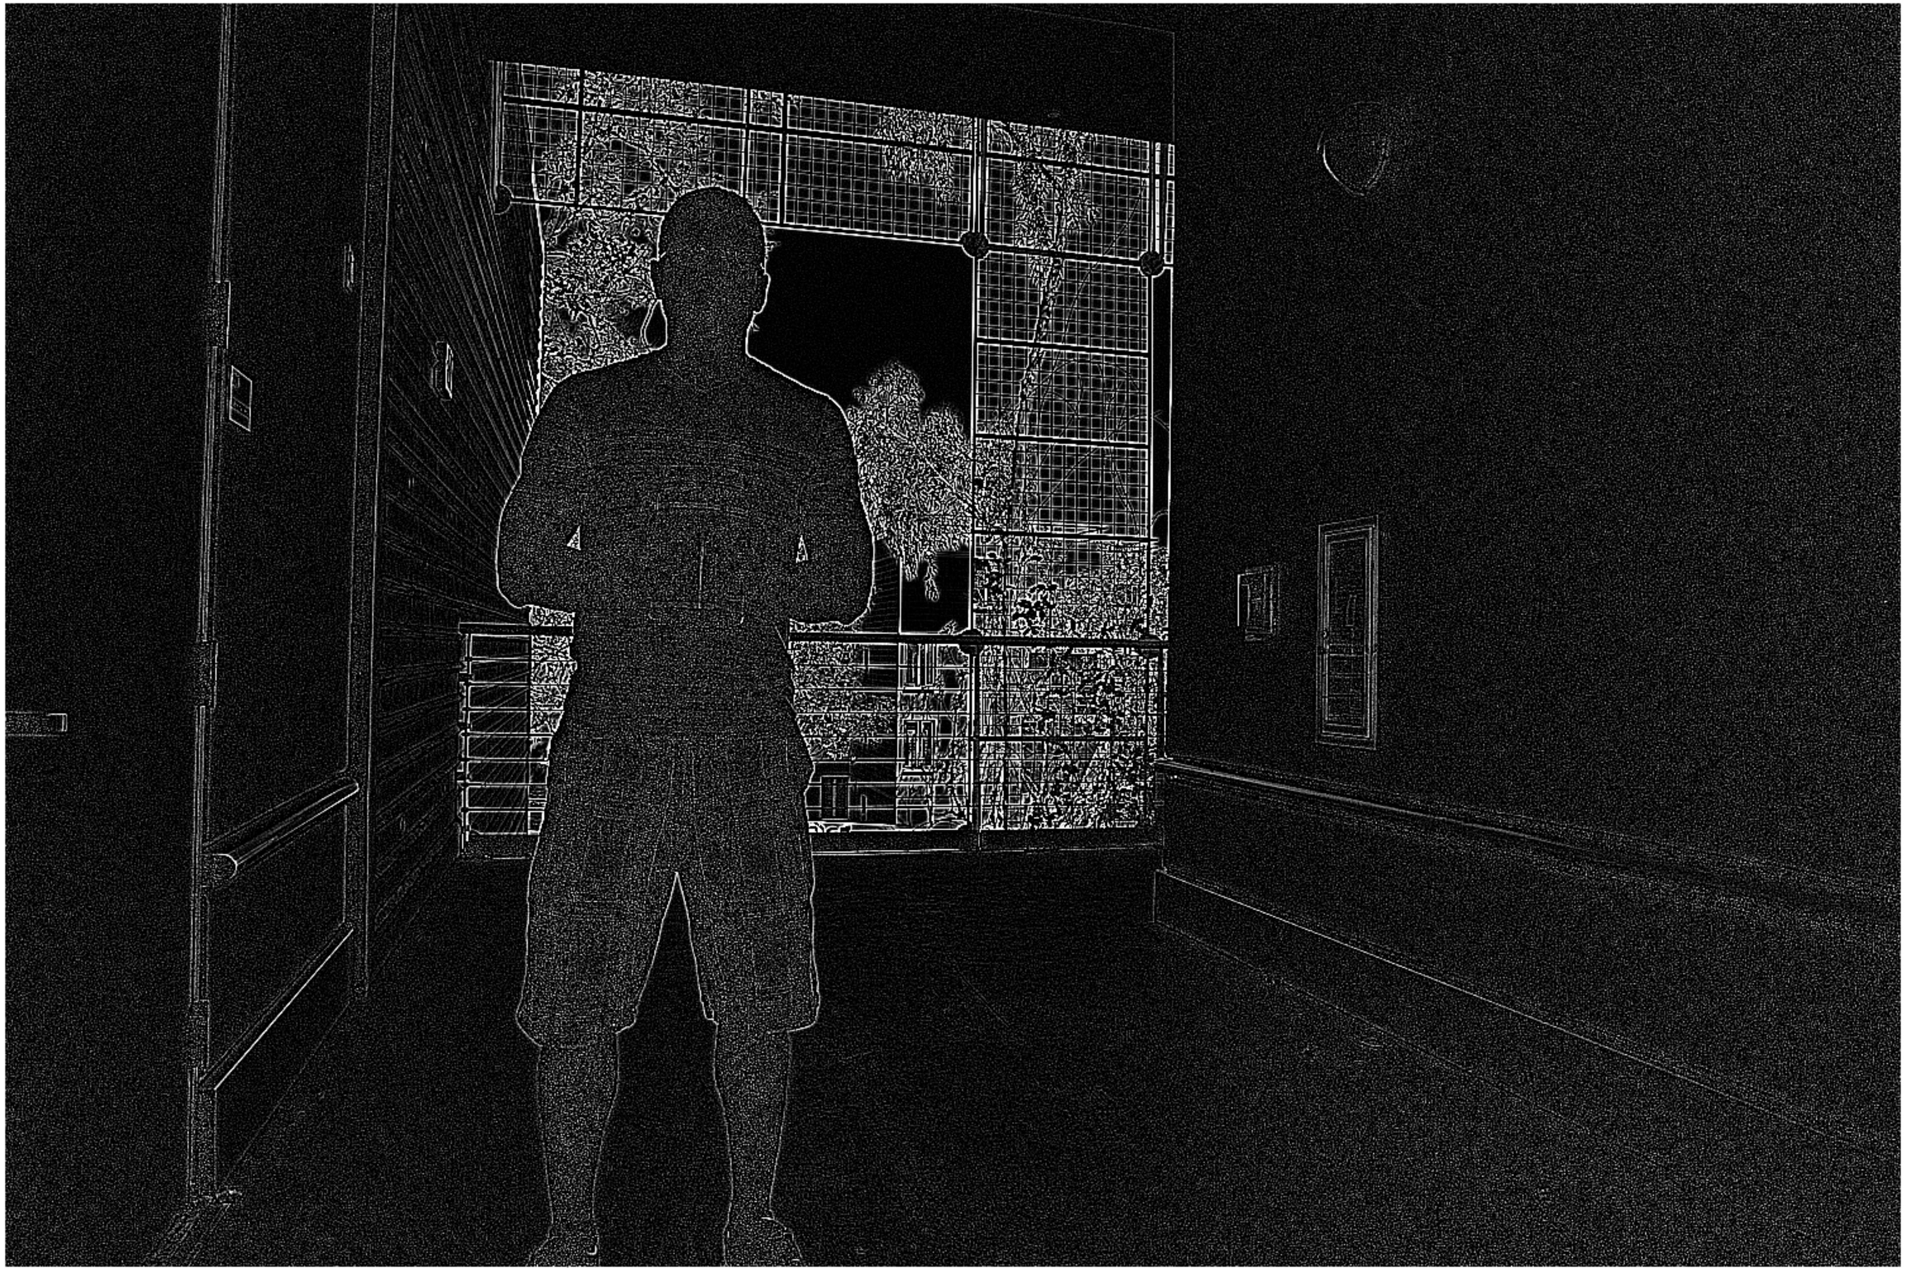

# Structure Tensor map of Input LDR image 2

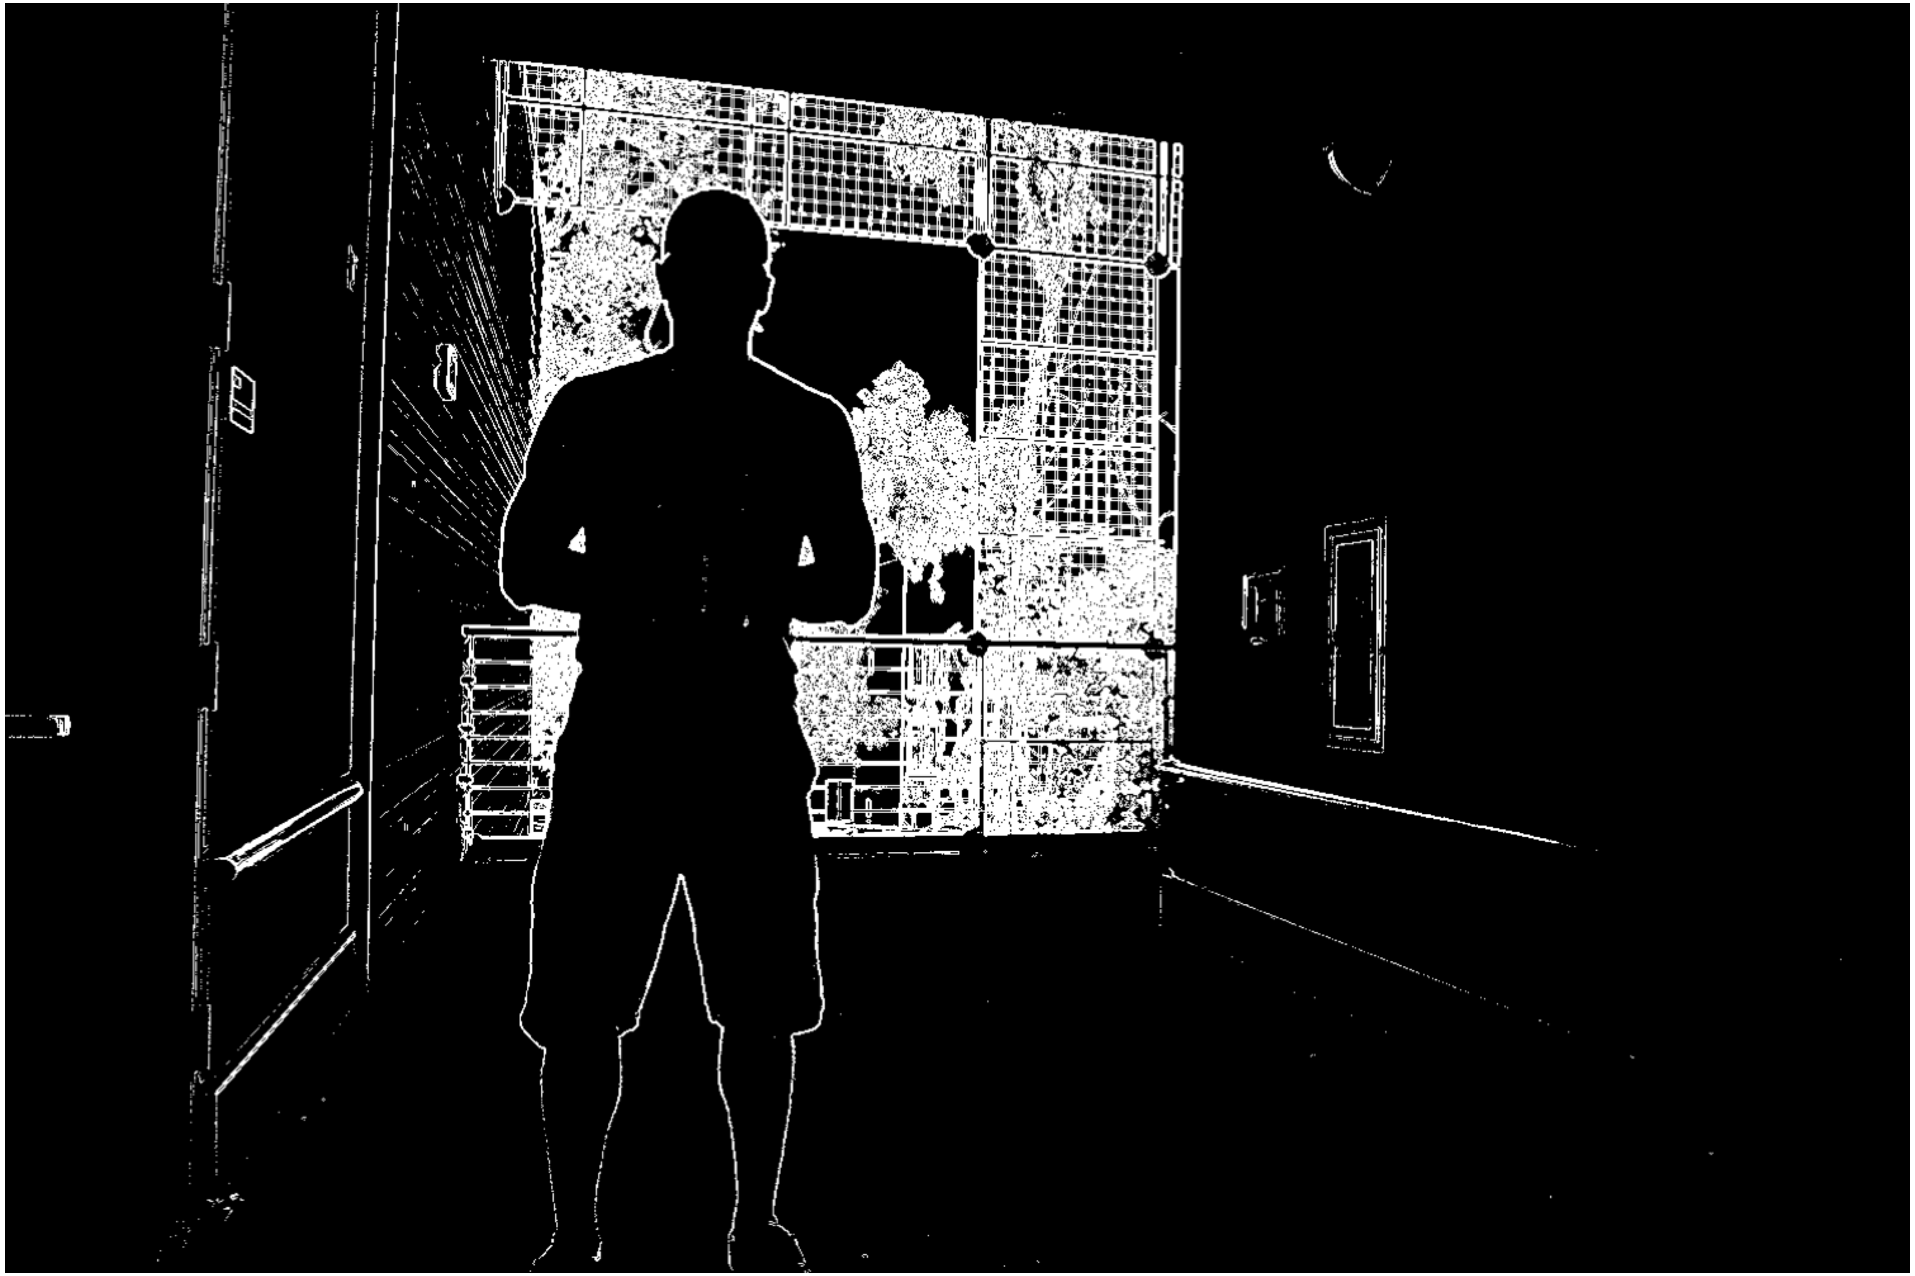

# Input LDR image 3

Exposure Value: +2.0

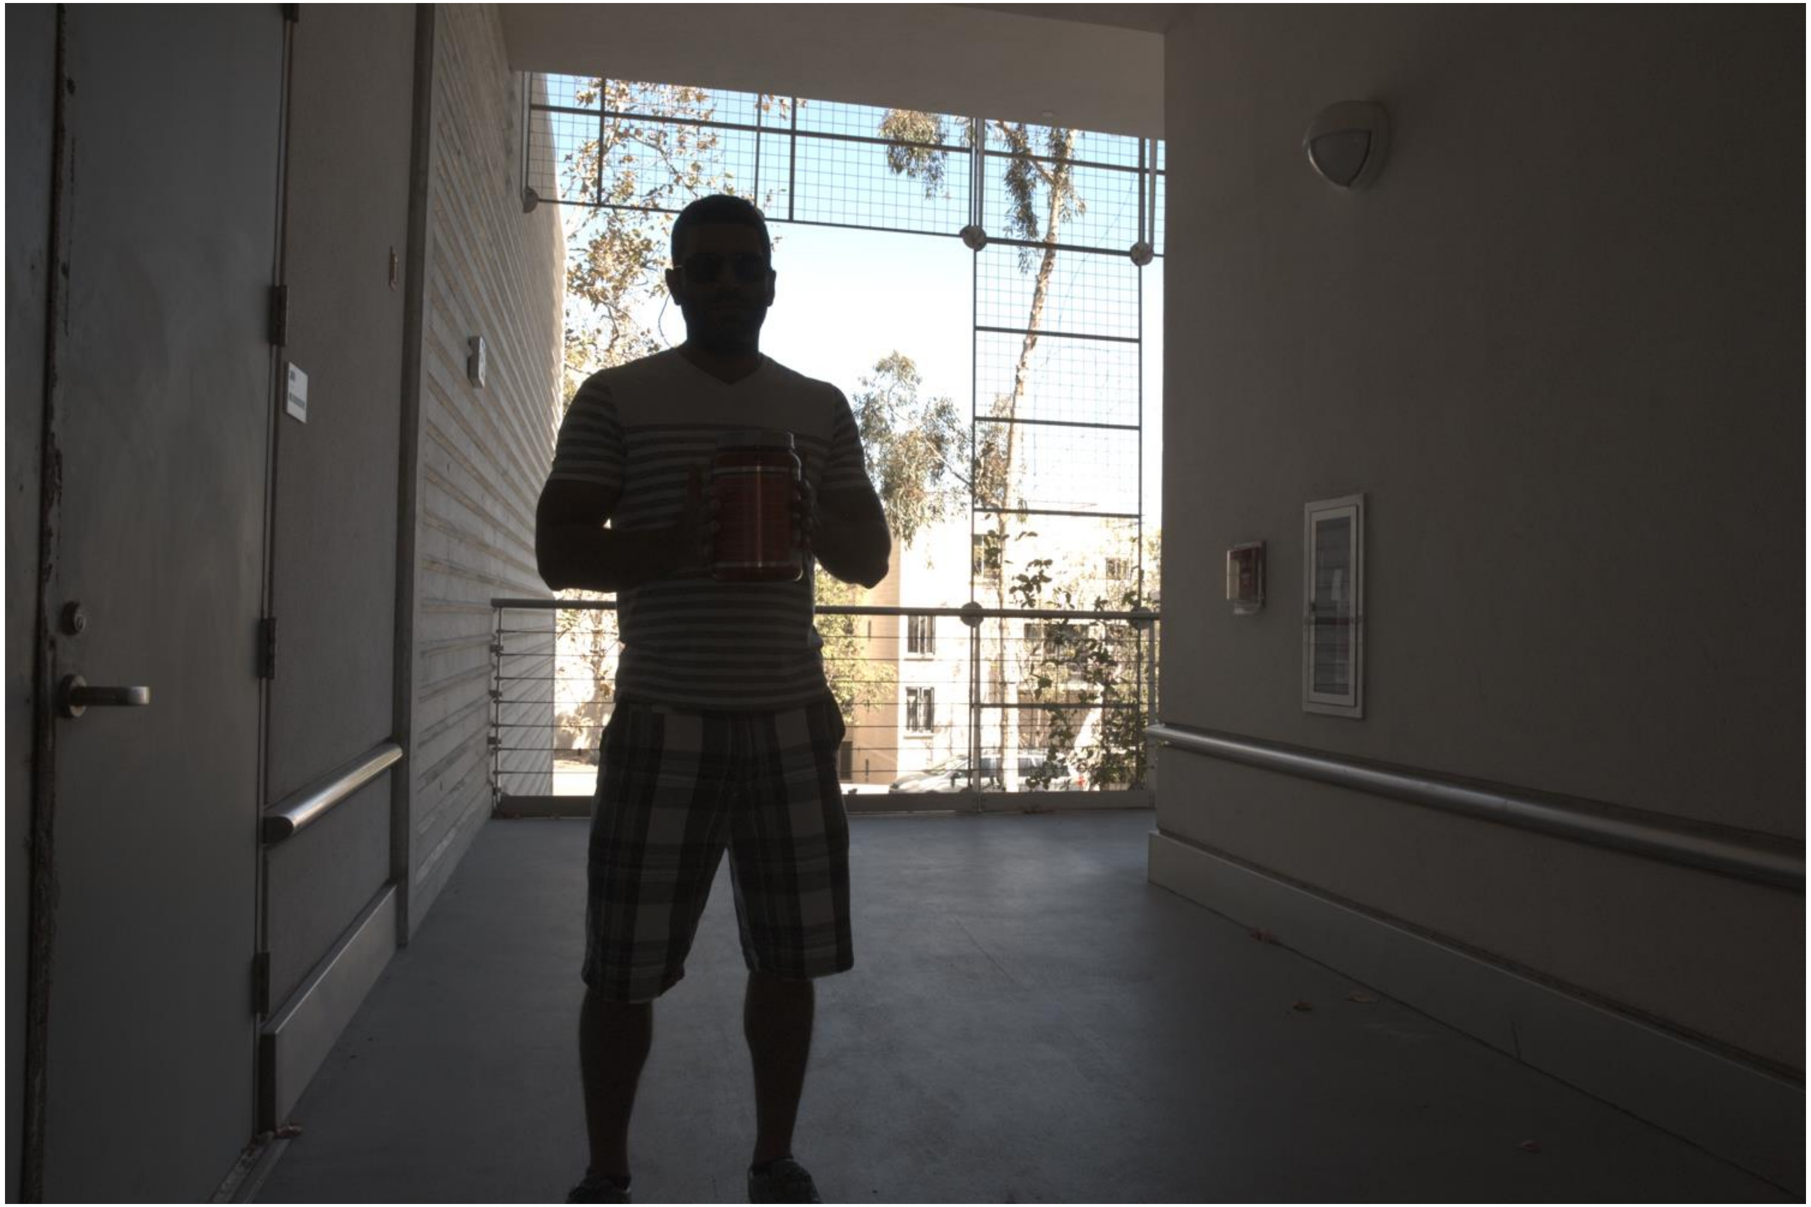

# Gradient map of Input LDR image 3

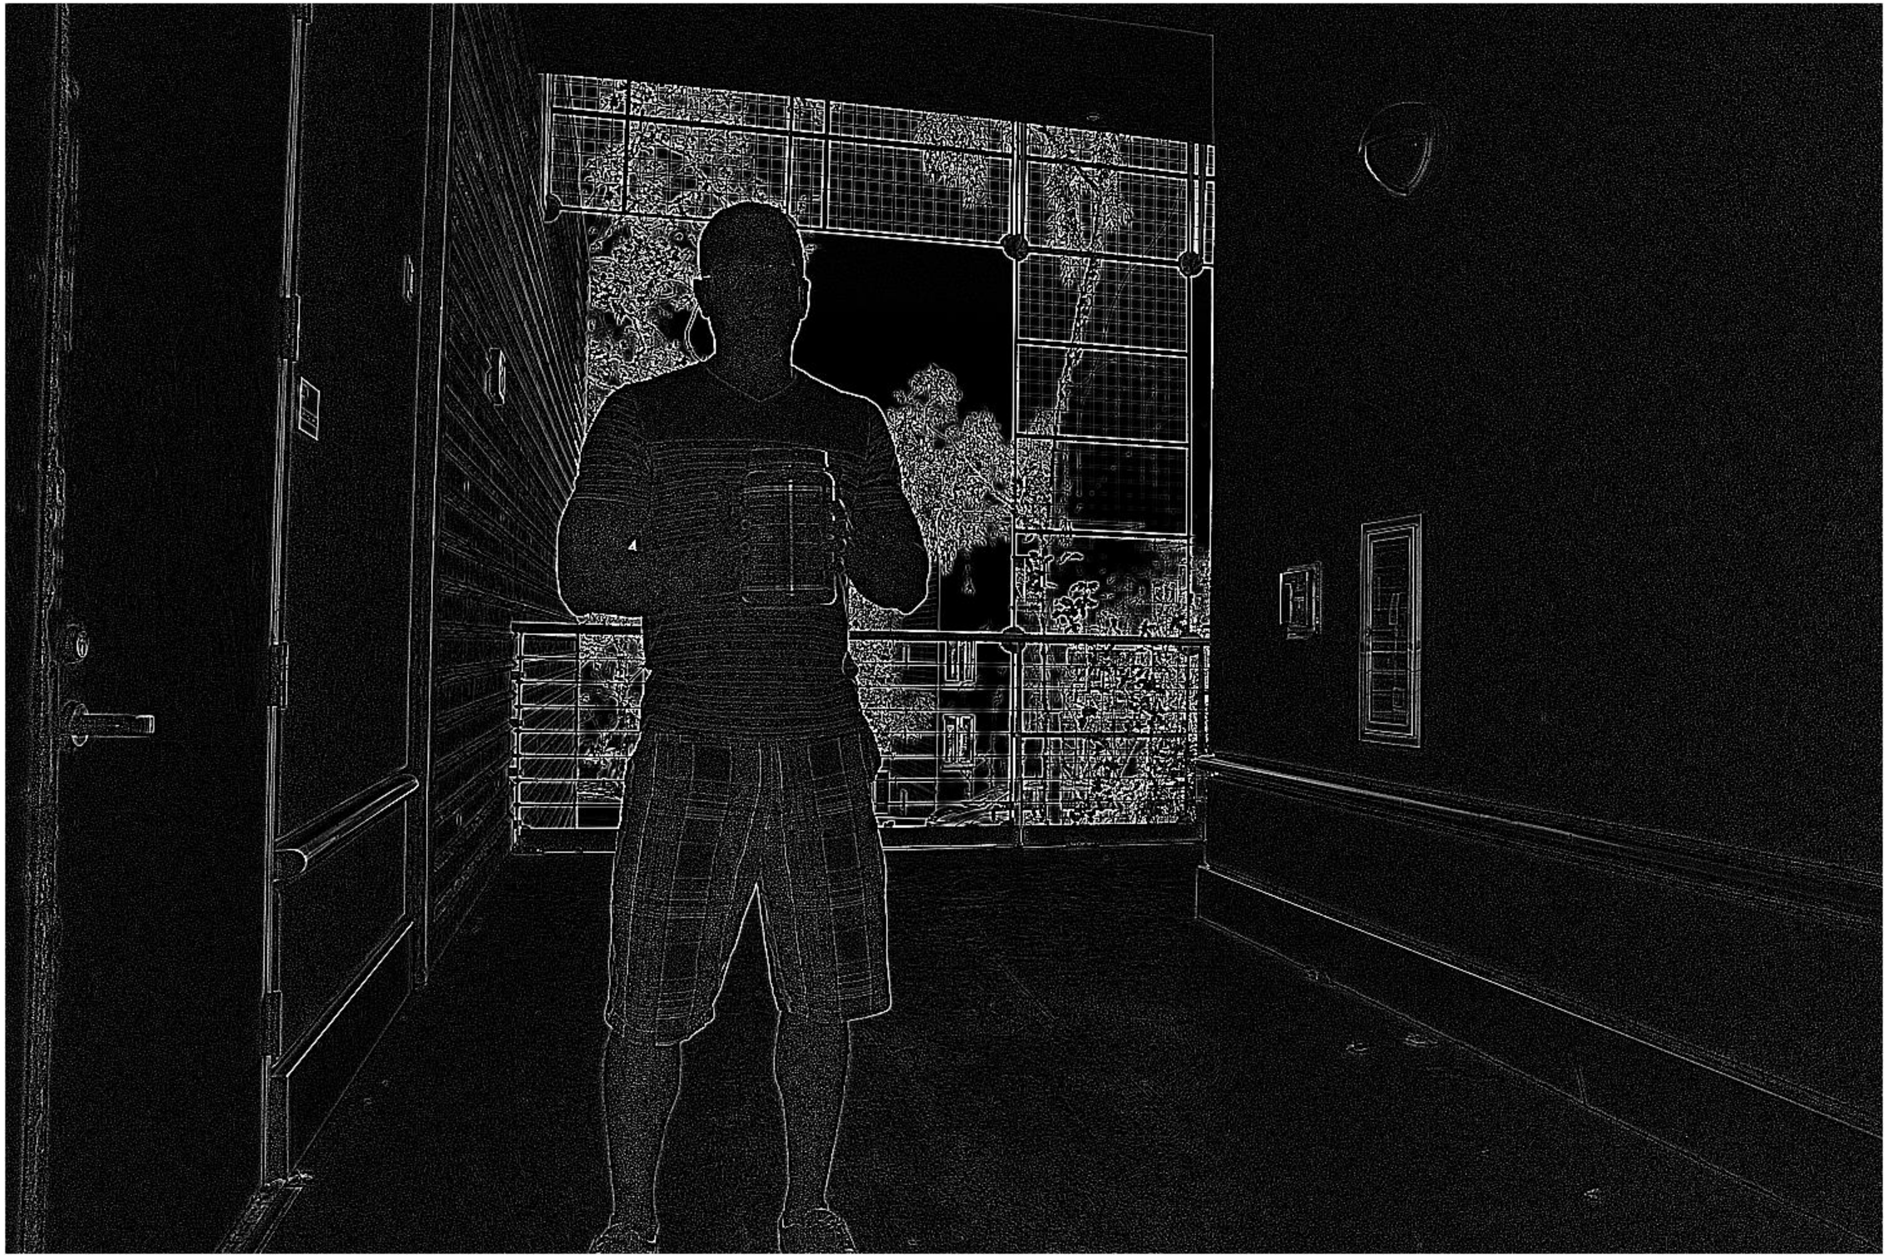

# Structure Tensor map of Input LDR image 3

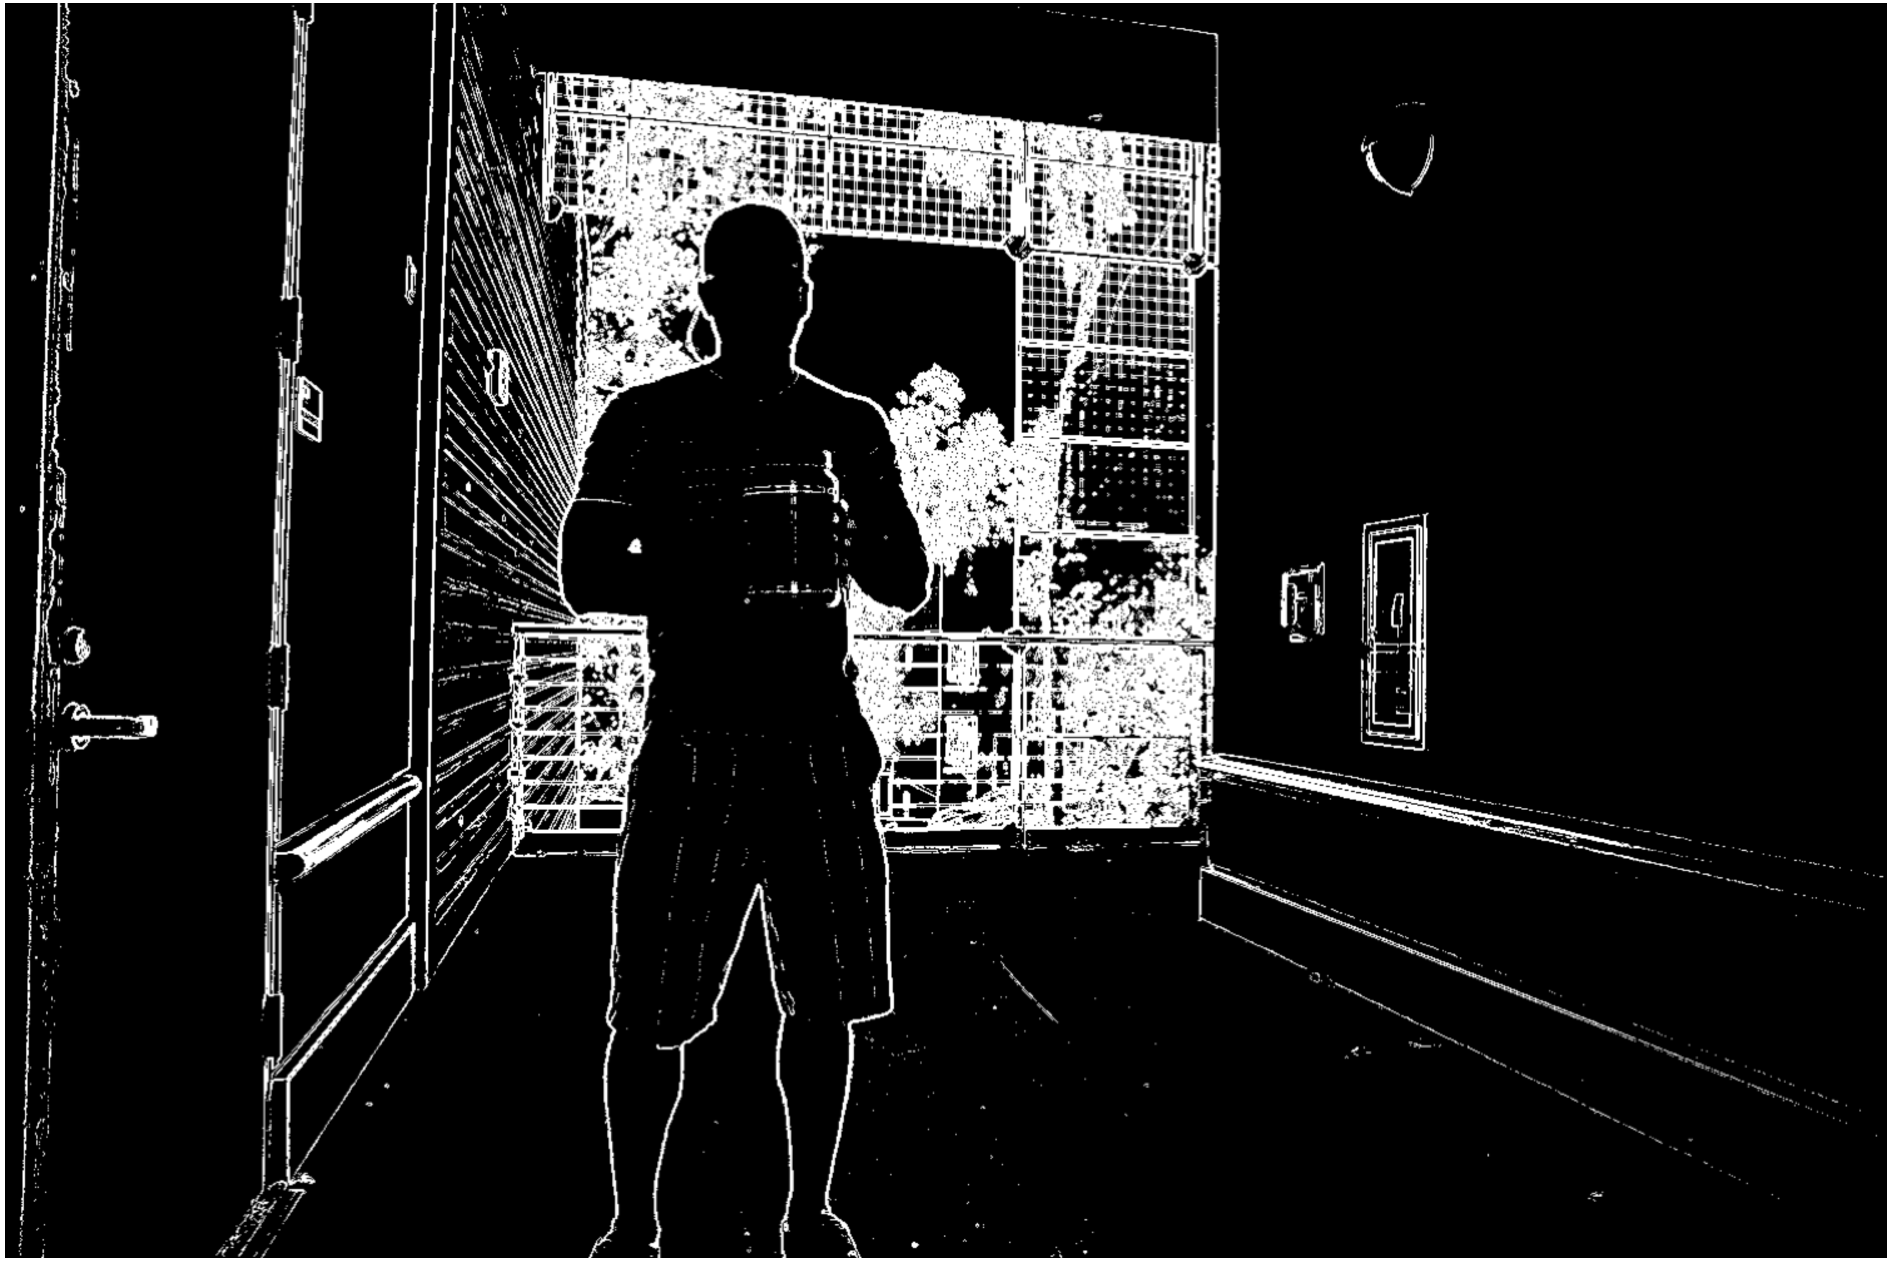

# Output
Mertens et al. (with ghosting artifacts)

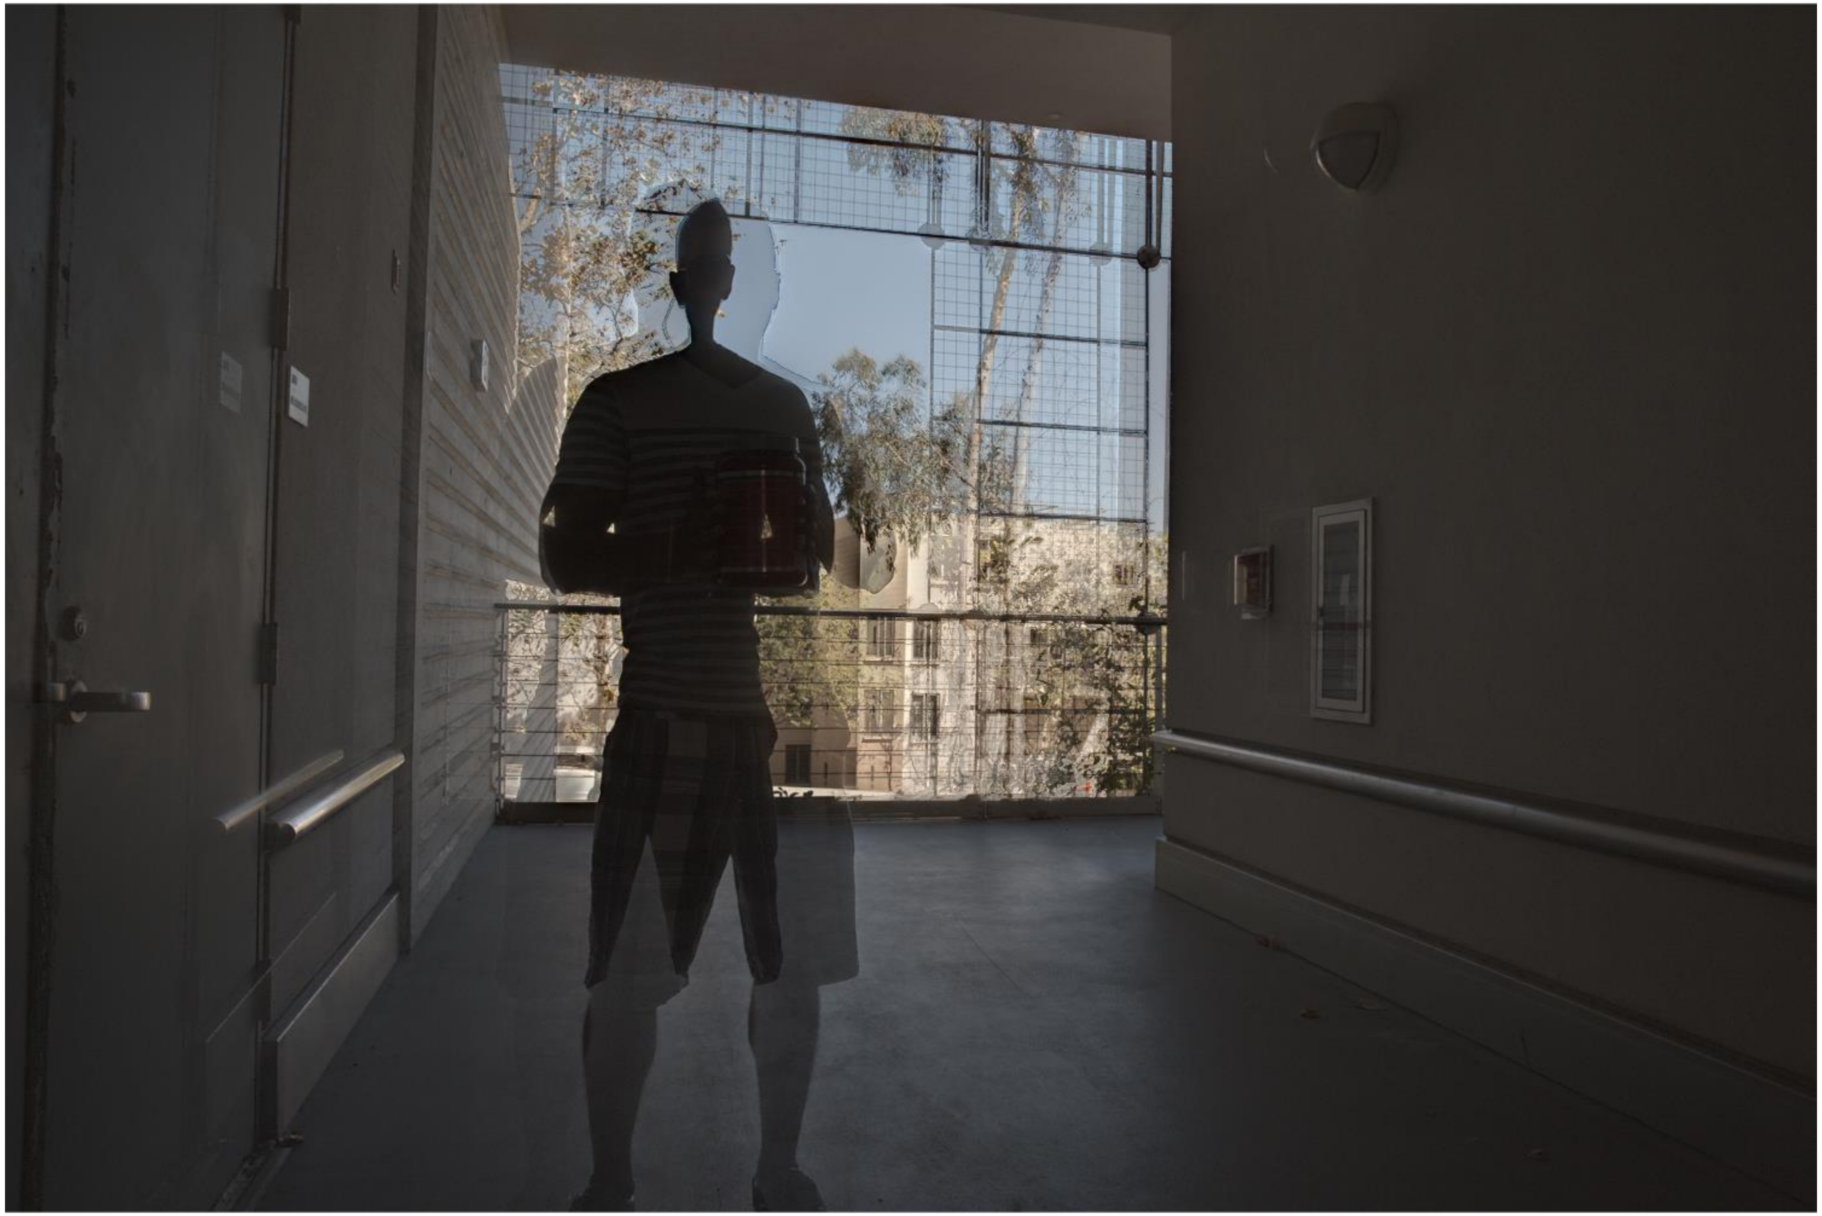

# Gradient map of Mertens

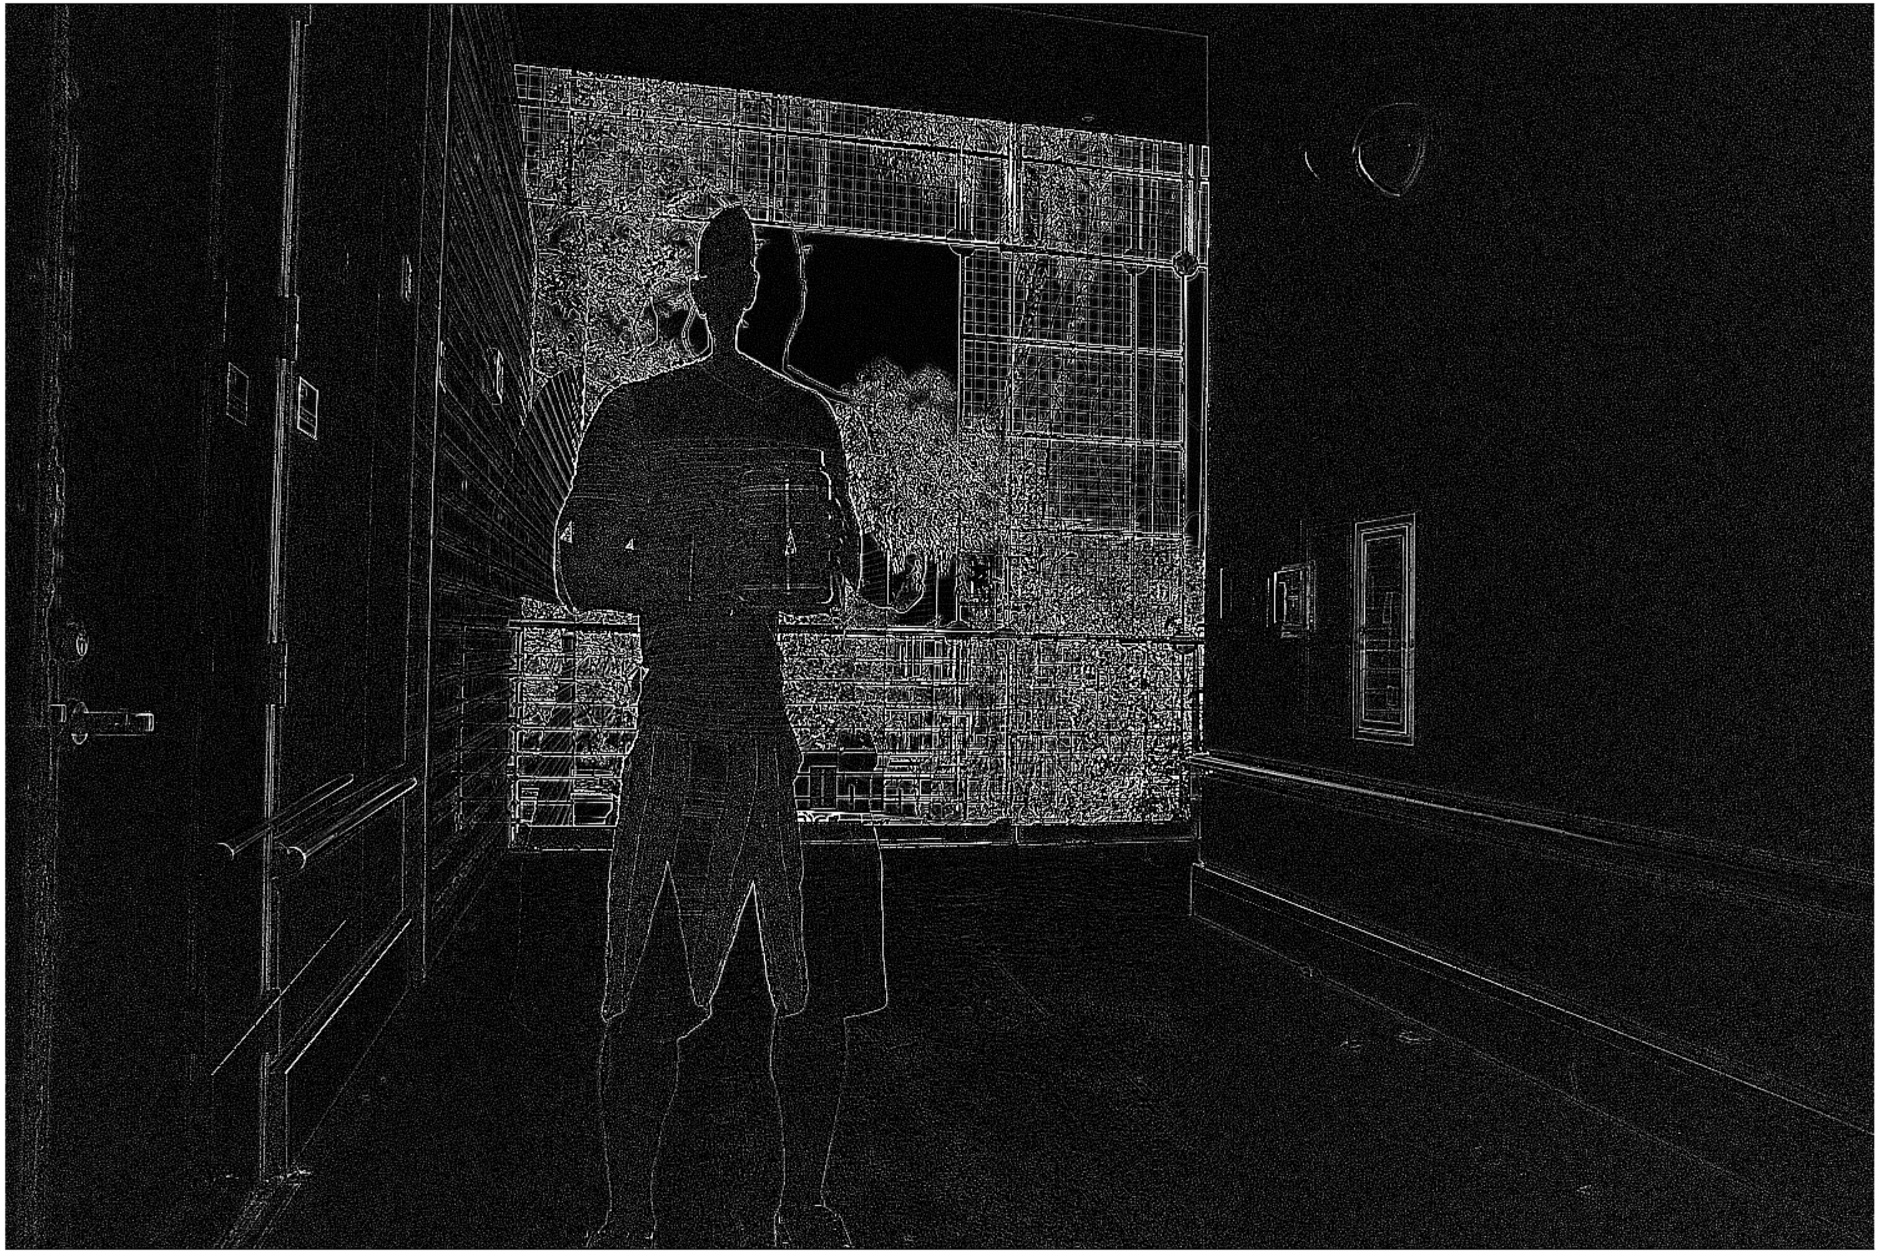

# Structure Tensor map of Mertens

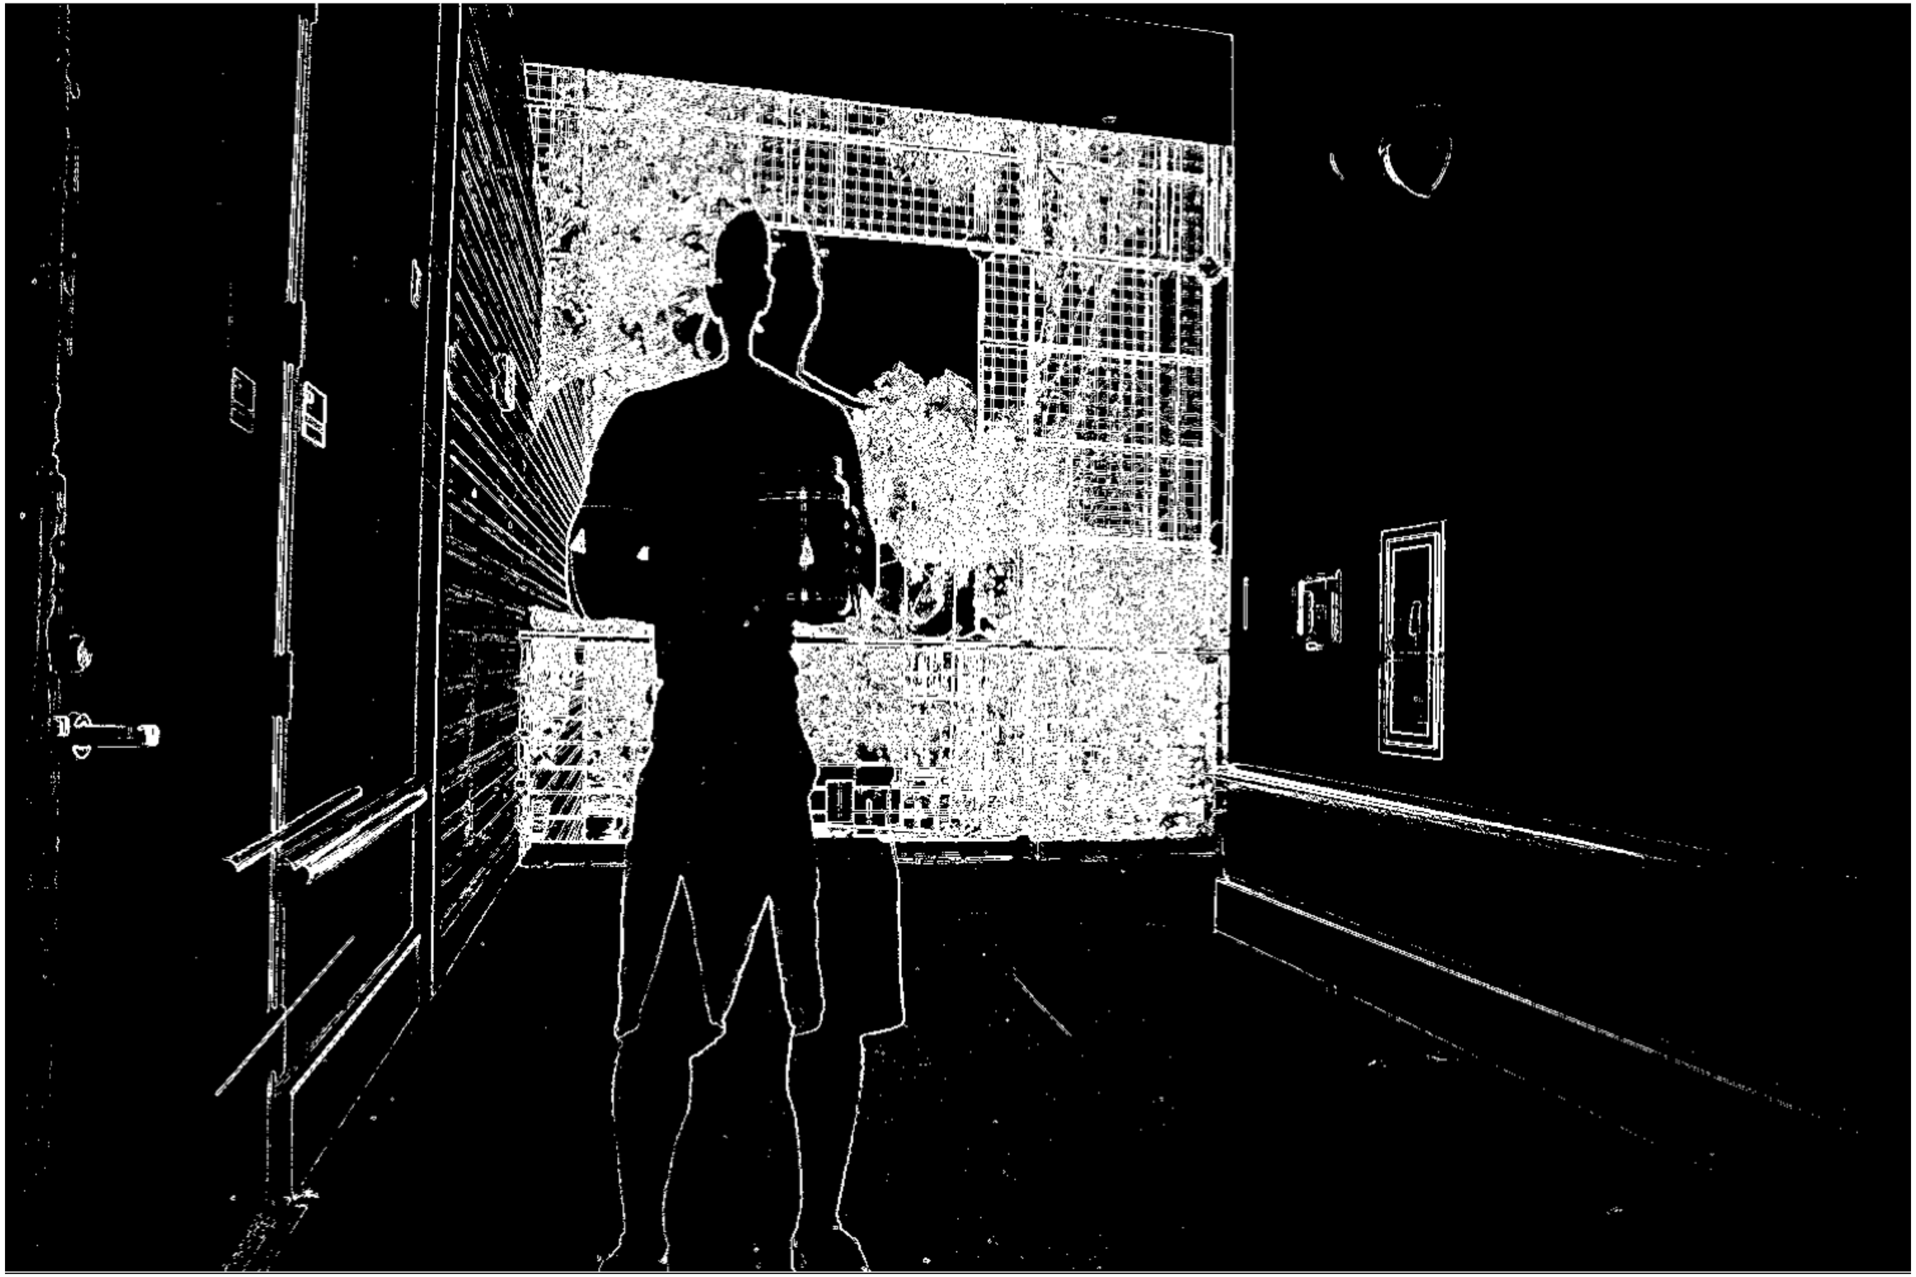

# Output

Ground Truth (without ghosting artifact)

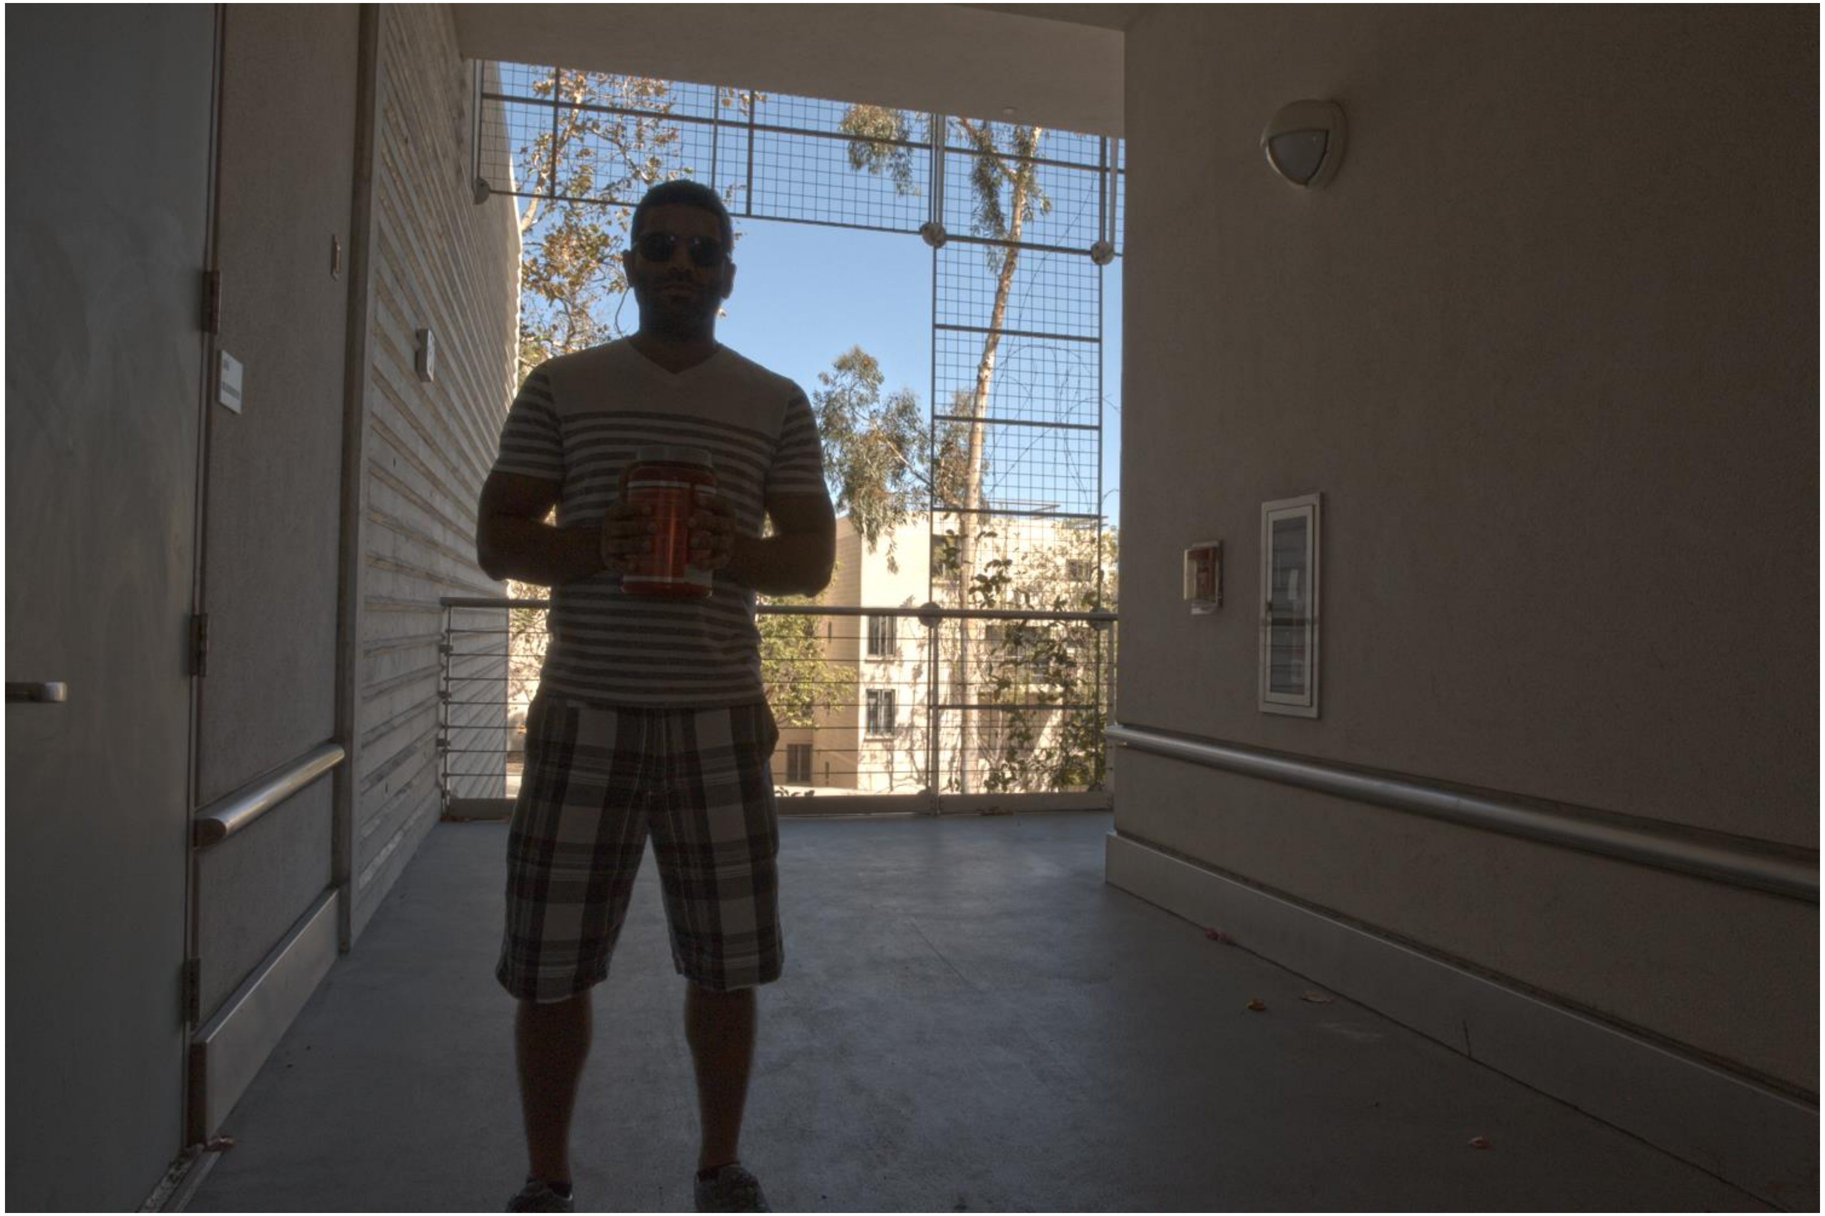

# Gradient map of Ground Truth

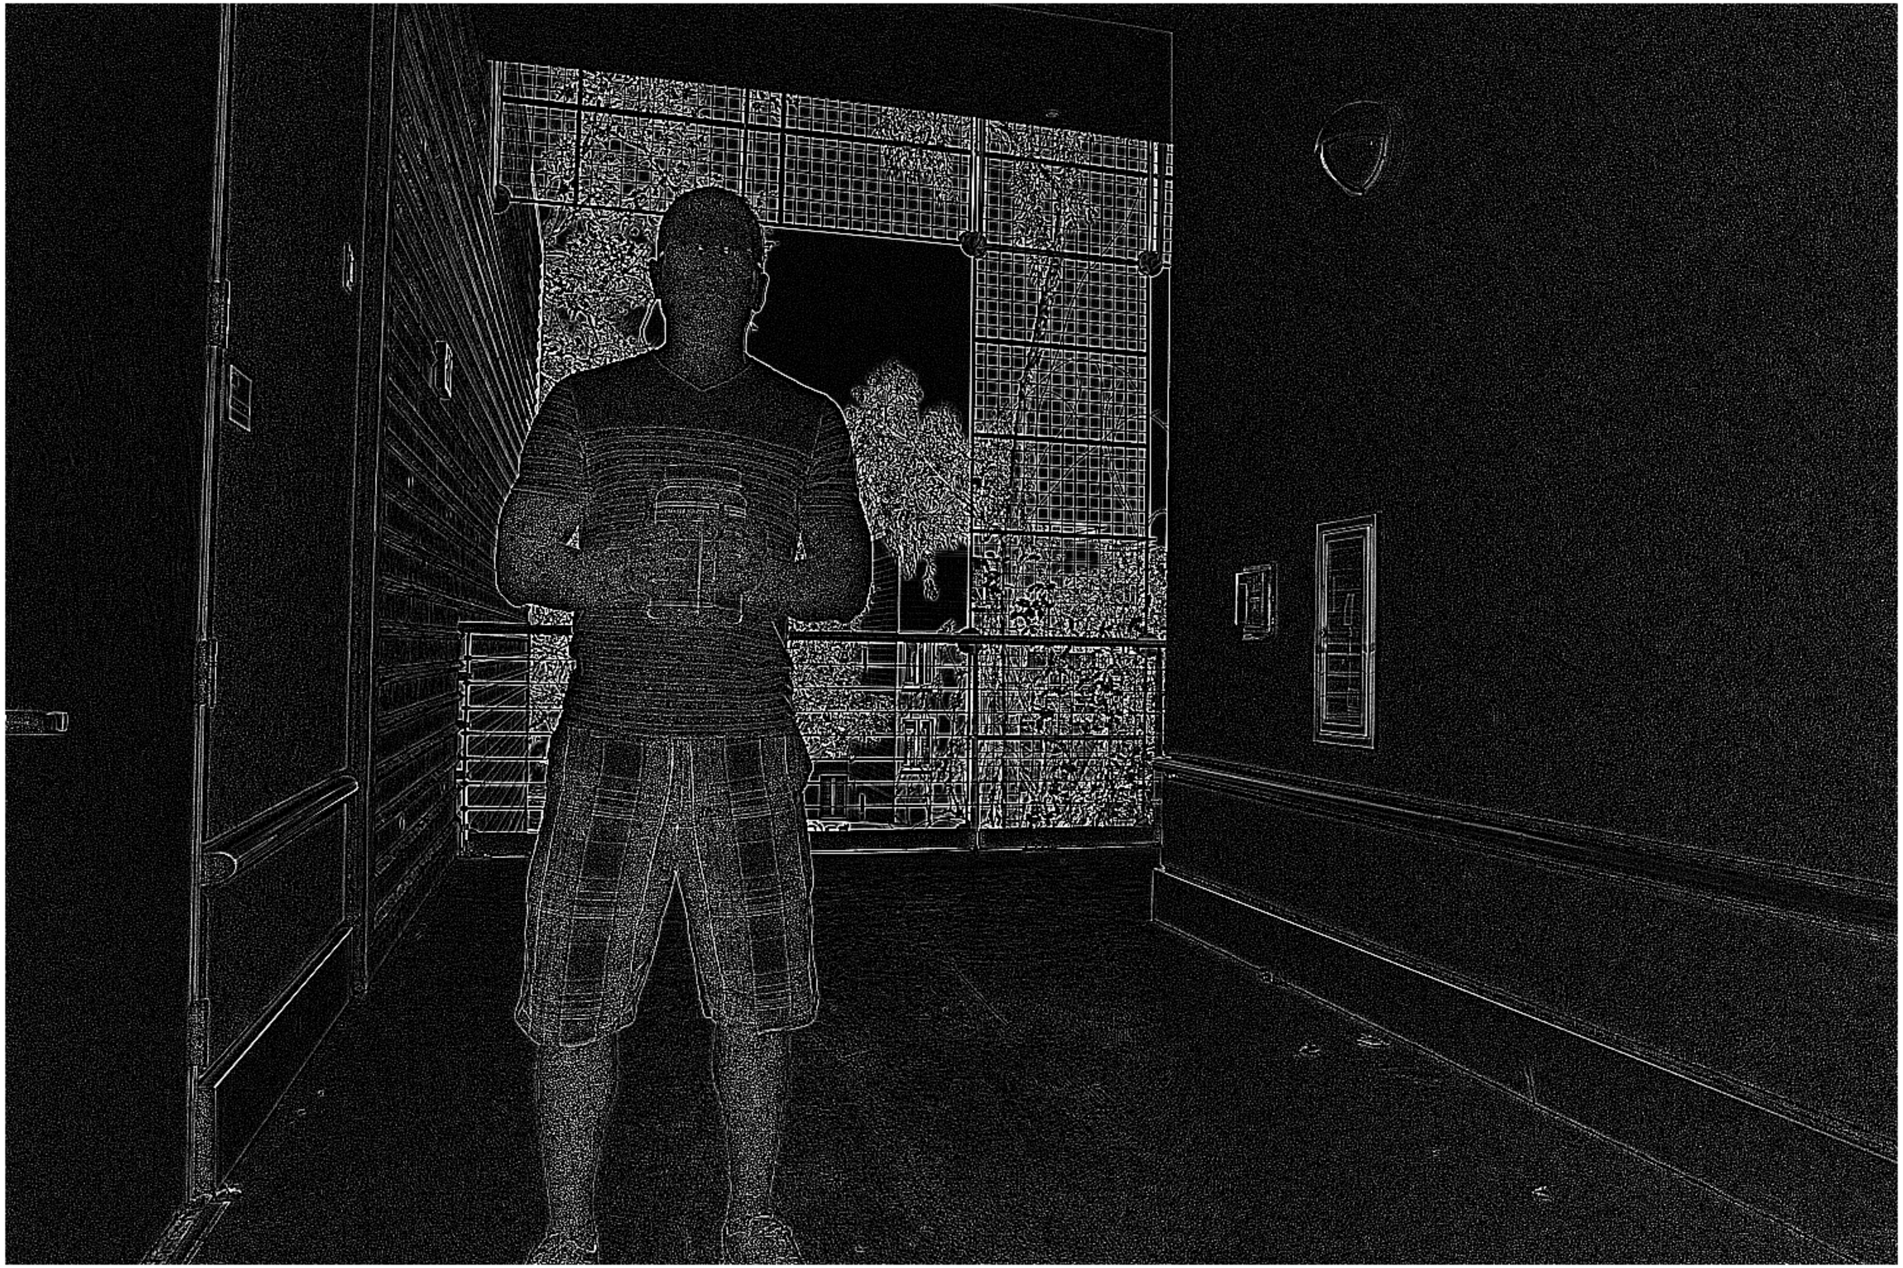

# Structure Tensor map of Ground Truth

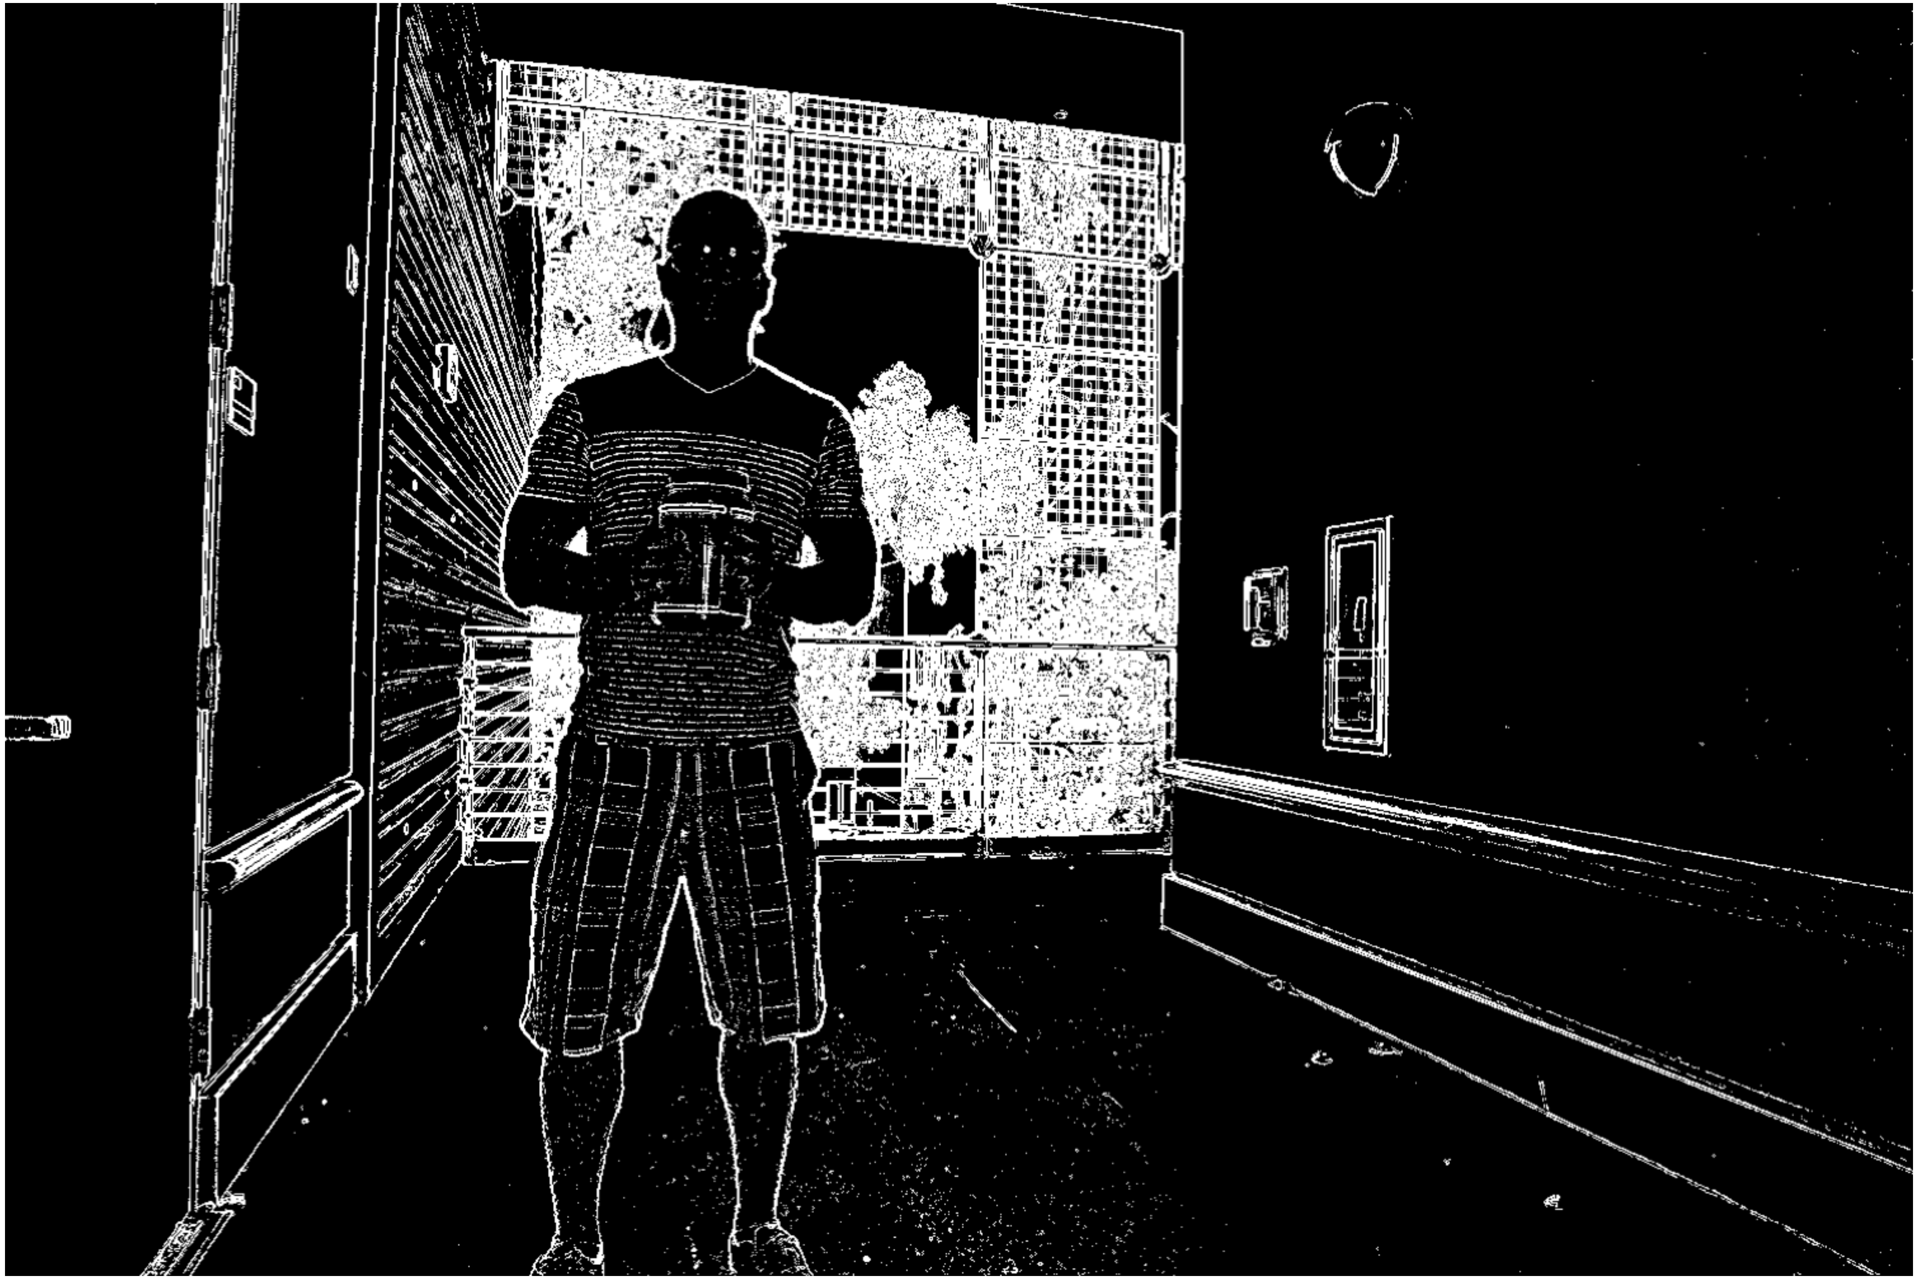

Supplement: Supplementary file 1 [file HDR_supp.pdf]
